# Supplementary material for: Computational Design of Lightweight Trusses
Source: arXiv:1901.05637 source file (2019-01-17)
Supplement: Supplementary file 2 [file Additional.tex]

\clearpage
\newpage
\section*{Functional Specifications}
In the following, we discuss the validity of functional specifications and special cases that are not directly relevant to the main part of our framework, even though they are interesting for the problem itself.

\subsection*{Equilibrium Force Systems}
The input functional specification is essentially an equilibrium force system. For a system with forces $F_1$,$F_2$,...,$F_n$ acting at points $P_1$,$P_2$,...,$P_n$, there are two constraints of equilibrium: the balance of forces, $\sum_{i=1}^{n}F_i=\vec{0}$, and the balance of torques, $\sum_{i=1}^{n}{F_i\times P_i} =\vec{0}$. In mechanical engineering, the equilibrium force systems are usually classified into three types: parallel force systems, concurrent force systems, and non-concurrent force systems as shown in Figure \ref{fig:forcesys}. 
%We test our algorithm in

\begin{figure}[H]	\centering{
		\begin{overpic}
			[width=.99\columnwidth]{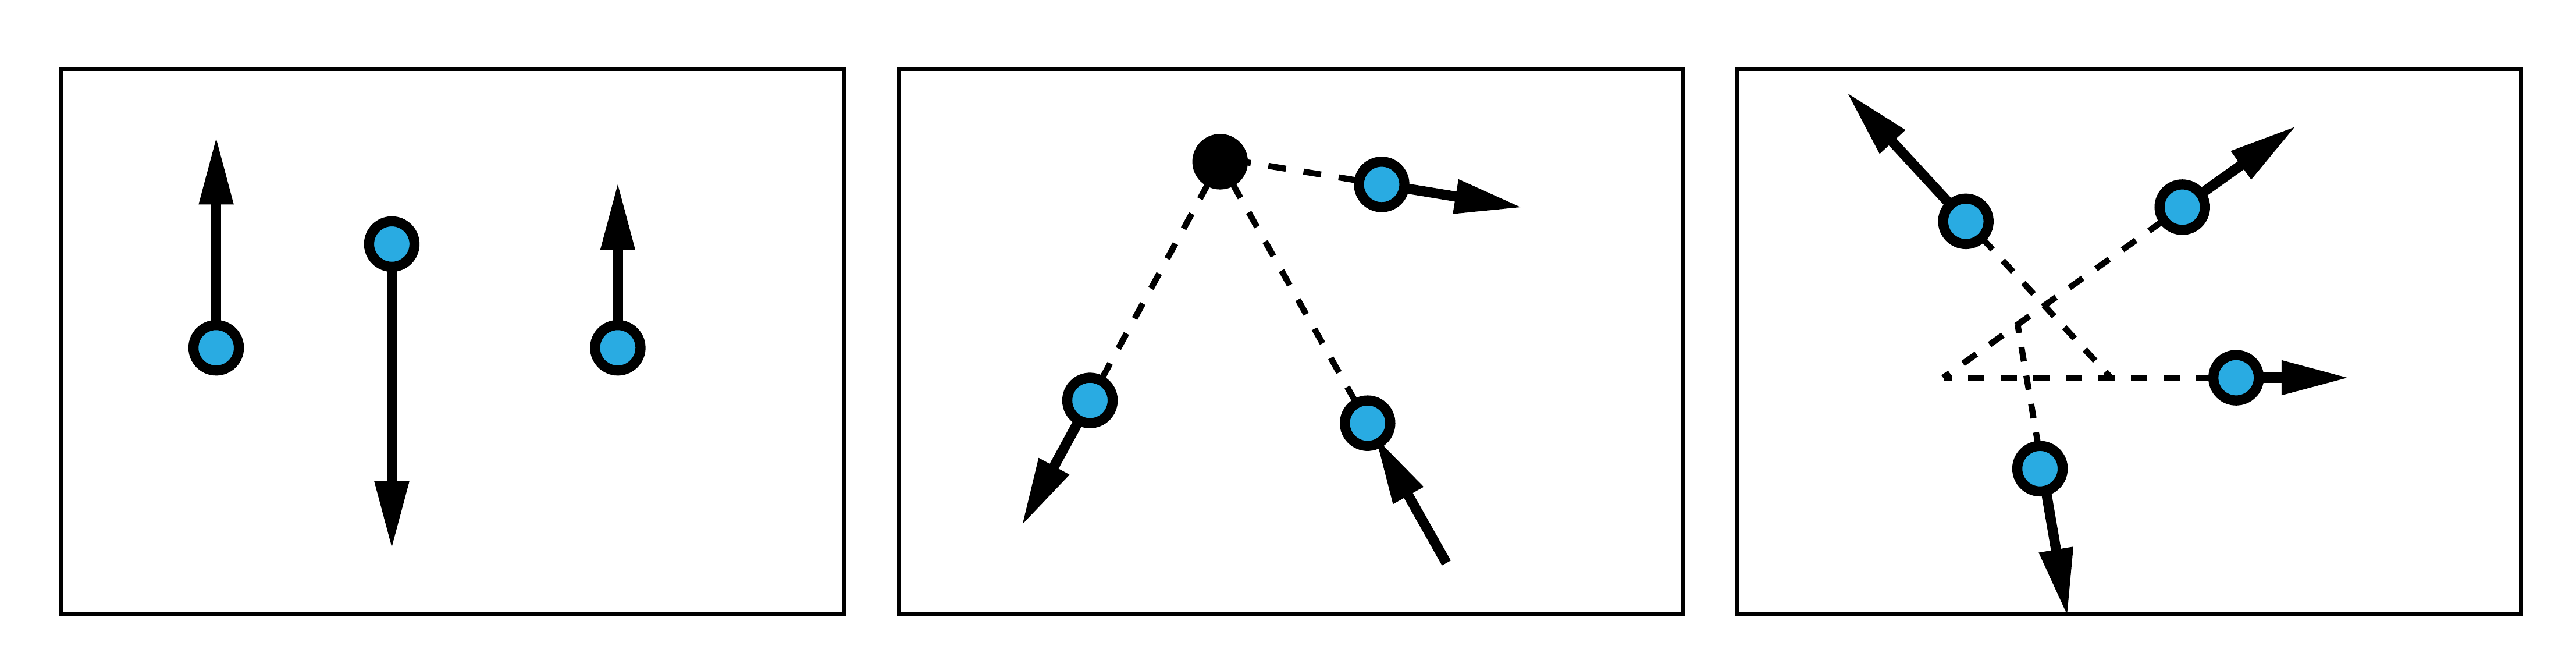}
			%[width=.99\columnwidth]{images/test}
			\cput(18,-2){\contour{white}{$(a)$}}	
			\cput(50,-2){\contour{white}{$(b)$}}
			\cput(82,-2){\contour{white}{$(c)$}}				
		\end{overpic}
	}	
	\caption{
		\label{fig:forcesys}
		Three equilibrium force systems. (a) A parallel force system. (b) A concurrent force system. (c) A non-concurrent force system.}
\end{figure}

\subsection*{Special Cases}

The theorem of Maxwell (1872) states that $\sum{f_il_i}=C$, where $C$ is the same constant for any statically admissible truss layout considering a giving set of external forces. As a consequence, if it is found possible to design a structure all of whose members are in tension, or alternatively in compression, then the optimum design has been achieved, because $\sum{\left | f_i \right |l_i}=\left | C \right |$. The above statement assumes that the input force system is precisely given. For example, a self-equilibrium force system with no supporting points, such as the 3-force problem in 2D and 4-force problem in 3D. However, it is not correct when some supporting points are given without prescribing their reaction forces. For example, as shown in Figure \ref{fig:2bars}, we can find a structure of two bars with compression on the left, but it is not an optimal structure because reaction forces at boundary could be changed to achieve a better results as show on the right.
\begin{figure}[H]	\centering{
		\begin{overpic}			
			[width=.45\columnwidth,trim={2cm 11.5cm 2cm 11.5cm},clip]{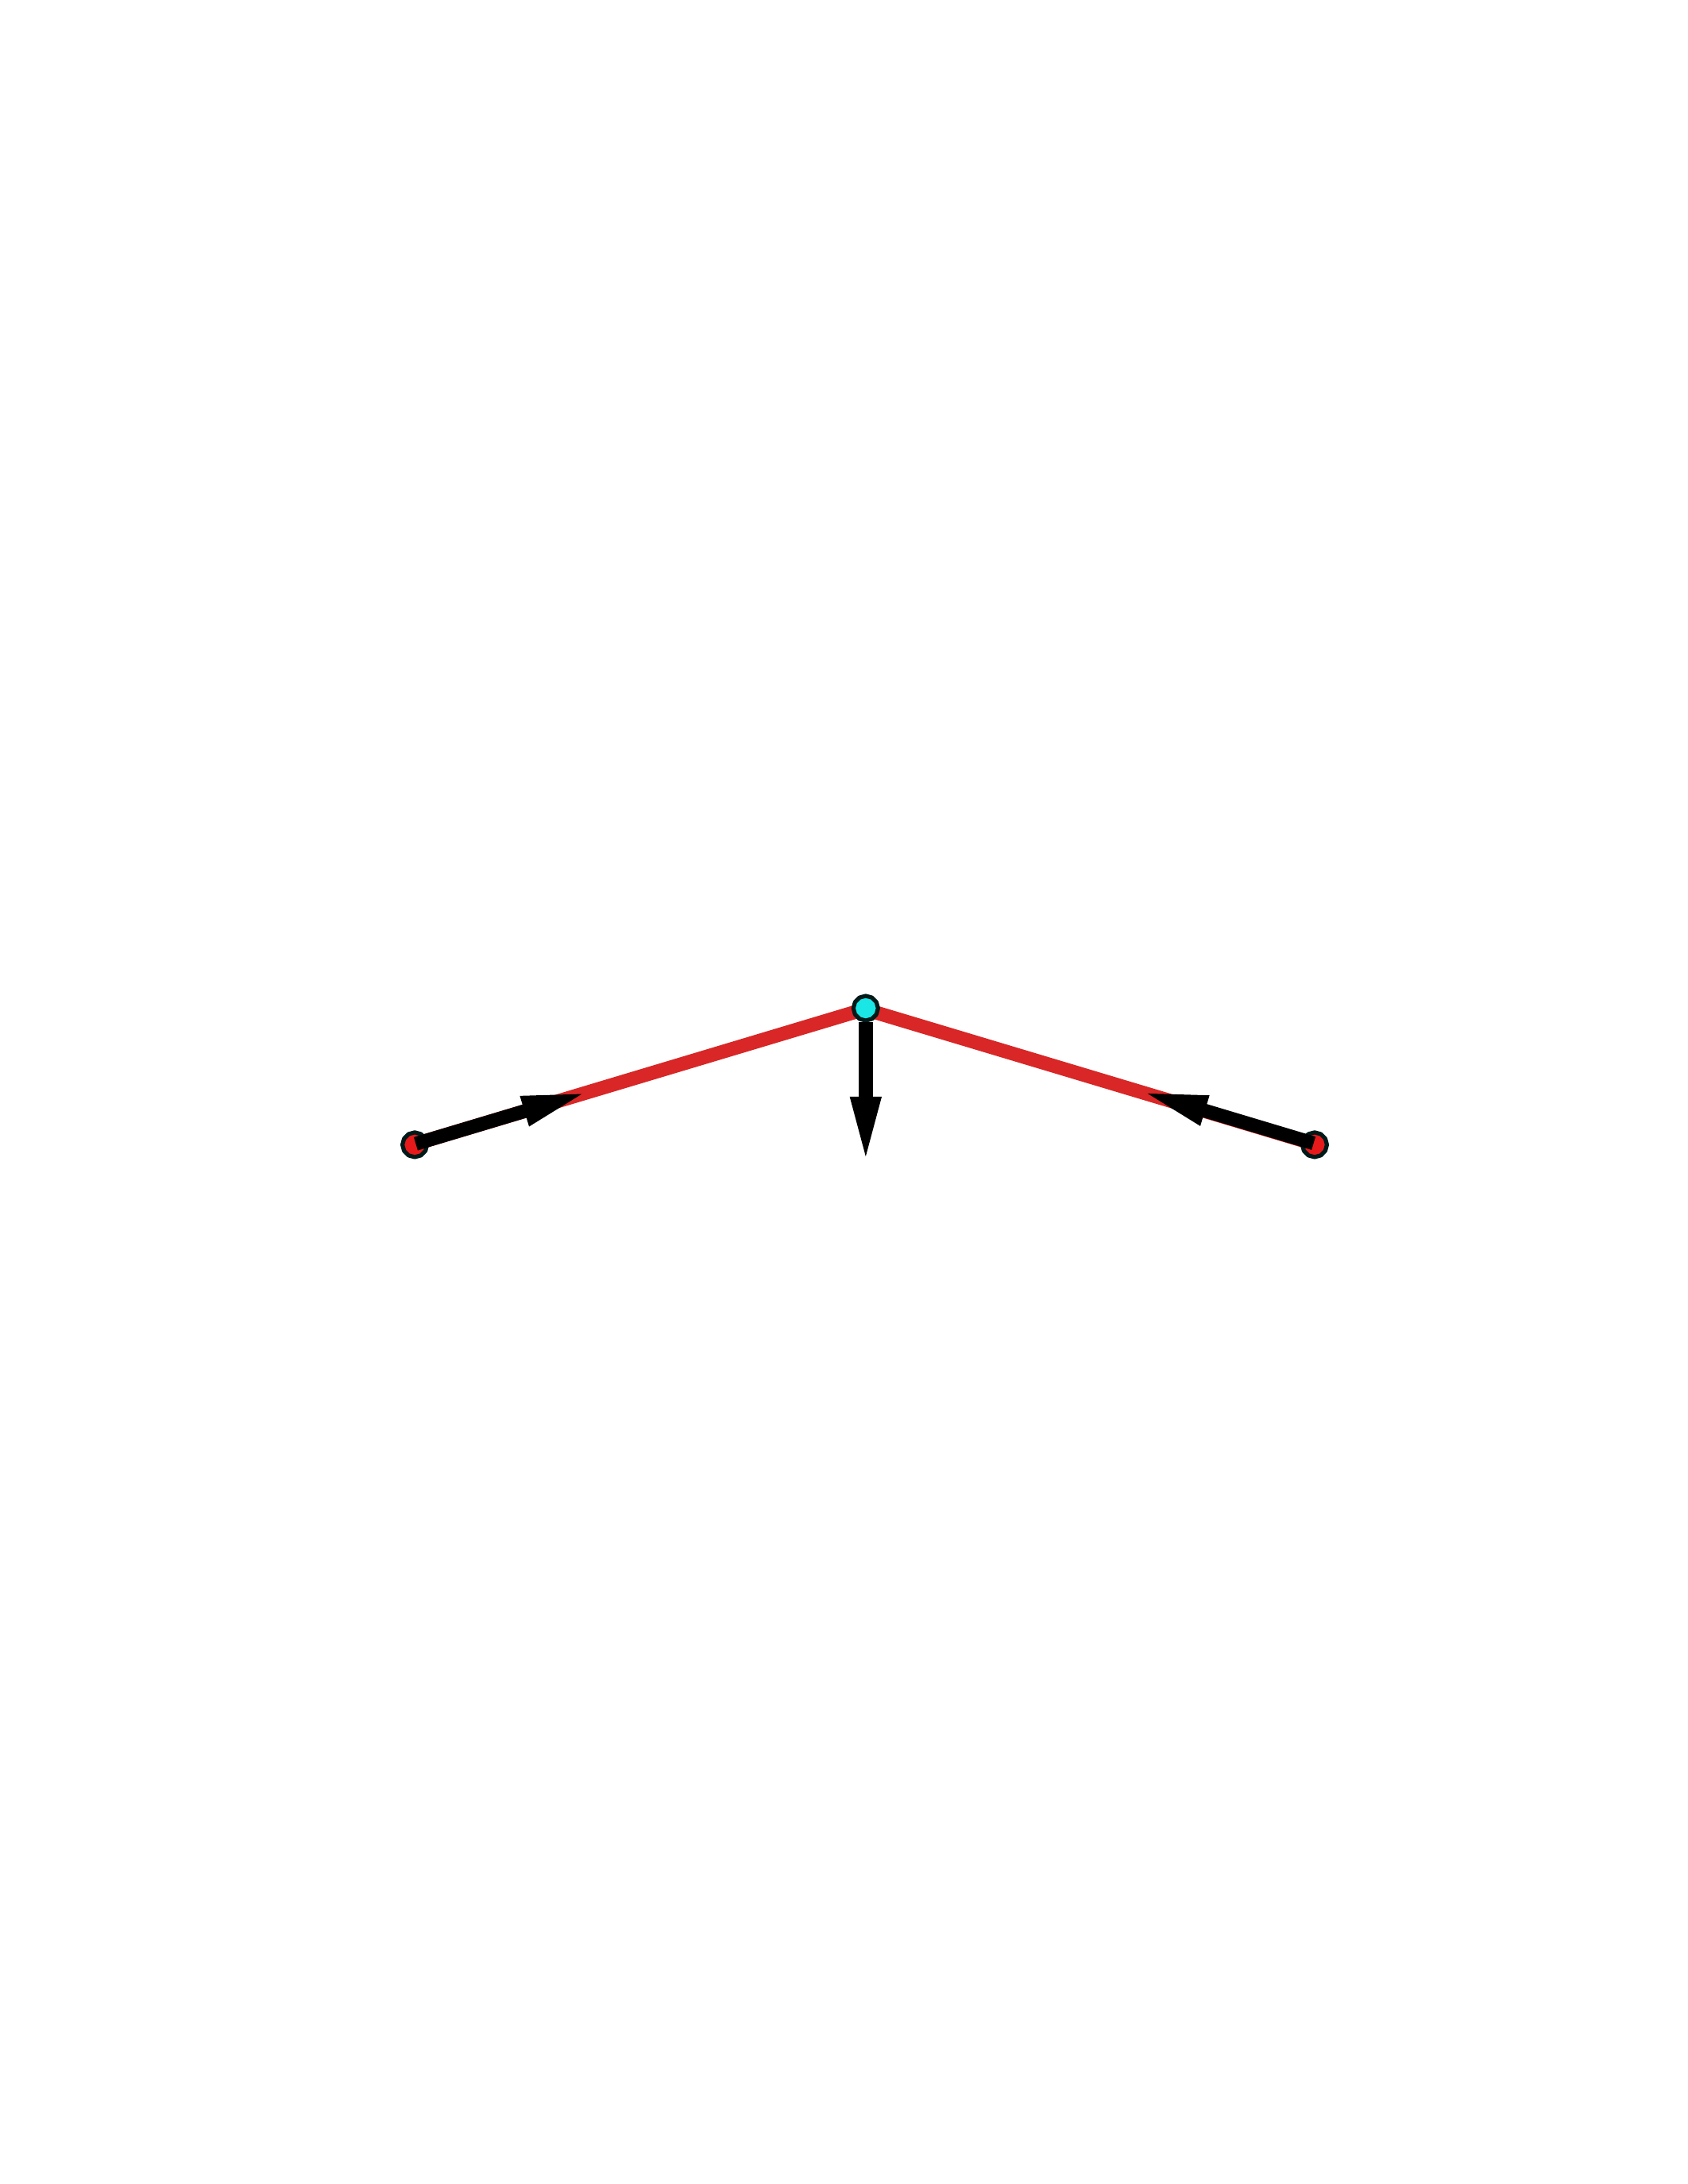}	
			\cput(50,2){\contour{white}{$(a)$}}		
		\end{overpic}
		\begin{overpic}			
			[width=.45\columnwidth,trim={2cm 10.5cm 2cm 11.5cm},clip]{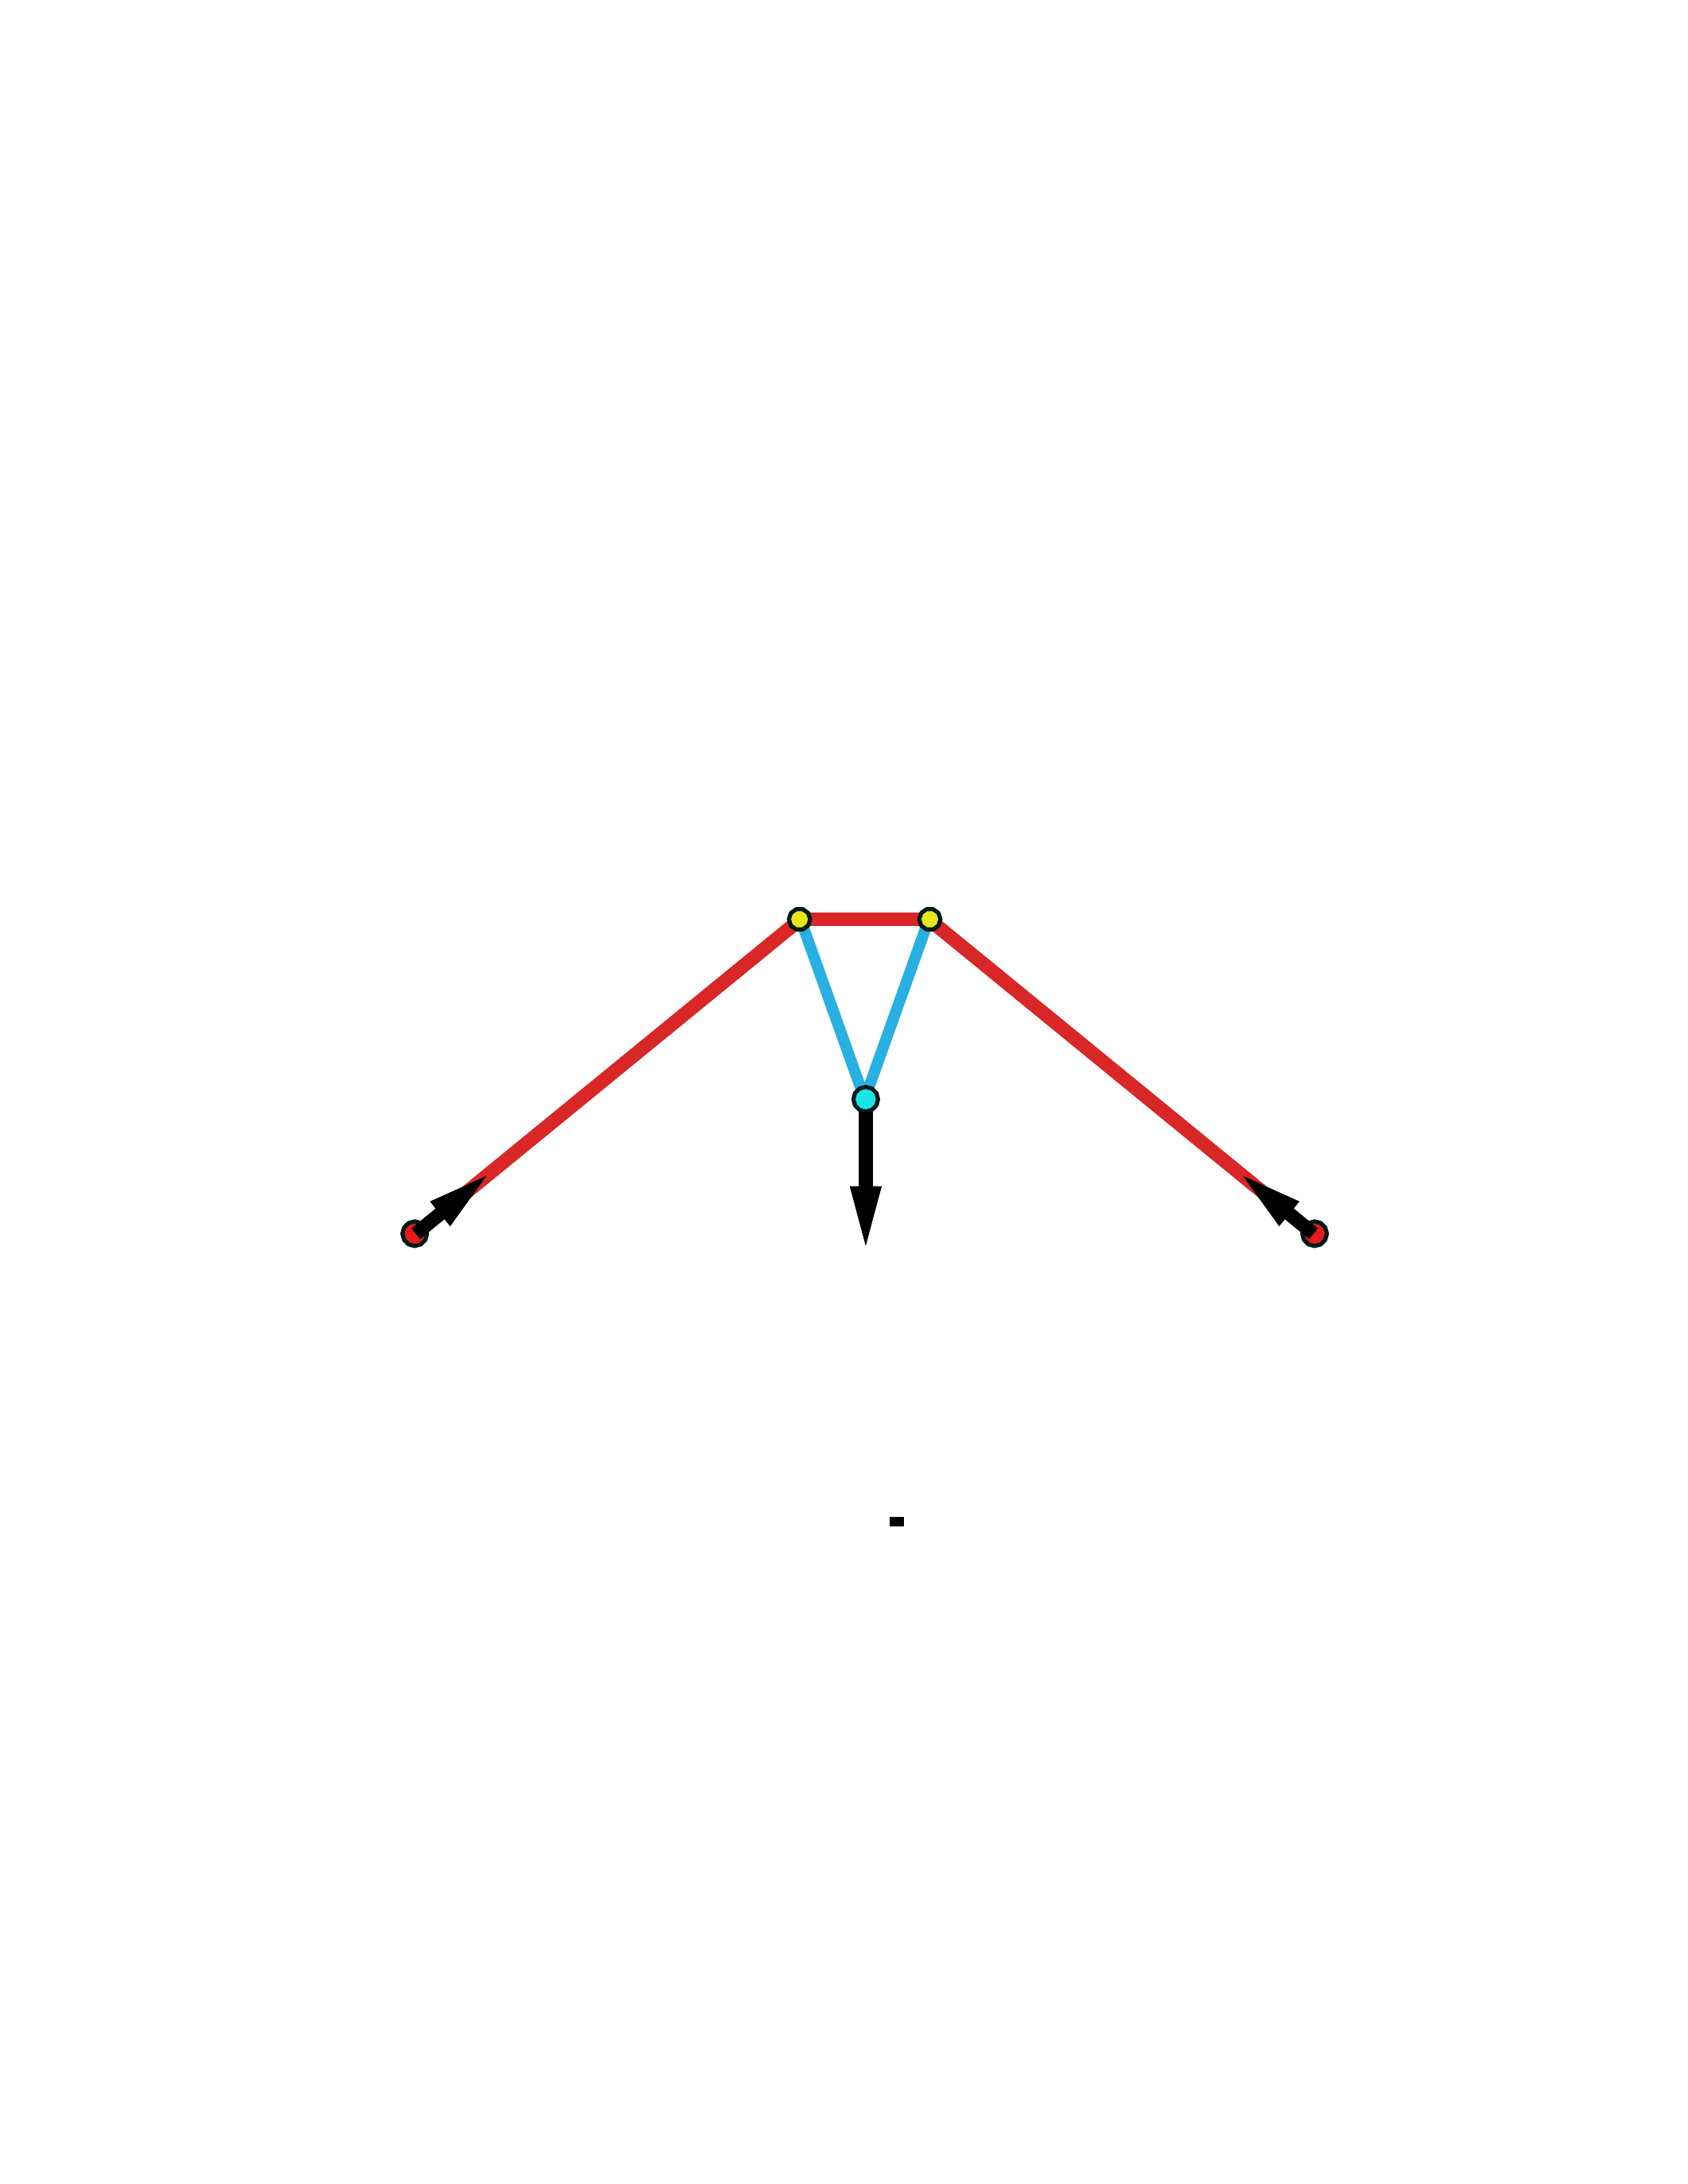}	
			\cput(50,2){\contour{white}{$(b)$}}	
		\end{overpic}
		
	}	
	\caption{
		\label{fig:2bars}
		The inputs are two supporting points and one external load. (a) A truss of two bars in compression. (b) A better design as reaction forces at supporting points are changed to obtain a less-material structure.}
\end{figure}
%Derived from Michell Theroem, xxx state that if in a particular problem it is found possible to design a structure all of whose members are in tension, or alternatively compression, then the optimum design has been achieved. This statement is also proved in xxx. The above particular problem assume the force system is precisely given. For example, a self-equilibrium force system with no supporting points, such as the 3-force problem in 2D and 4-force problem in 3D. However, this statement may not sure when some supporting points are given without prescribing their reaction forces. For example, as shown in xxx, we can find a structure of two bars with compression, but it is not a optimal structure because reaction forces at boundary could be changed to achieve a better results as show in figure xxx right.

According to the theorem of Maxwell, we can easily find some special cases. For example, given a concurrent force systems with forces $F_1$,$F_2$,...,$F_n$ through a common point $O$ and their corresponding action points $P_1$,$P_2$,...,$P_n$, we have $F_i=\lambda_i\overrightarrow{OP_i}$. If all the $\lambda_i$ have the same sign, either positive or negative, then the truss connect all $P_i$ and $O$ is an optimal design. Note that the optimum for these special boundary conditions is usually not unique. Figure \ref{fig:nonunique} shows multiple optimal designs for the same boundary condition where 3 forces are self-equilibrium in 2D plane. From a design standpoint, the non-uniqueness provide flexibility of topology and geometry design for these special boundary conditions. 
\begin{figure}[H]	\centering{
		\begin{overpic}			
			[width=.32\columnwidth,trim={5cm 9cm 4.5cm 9cm},clip]{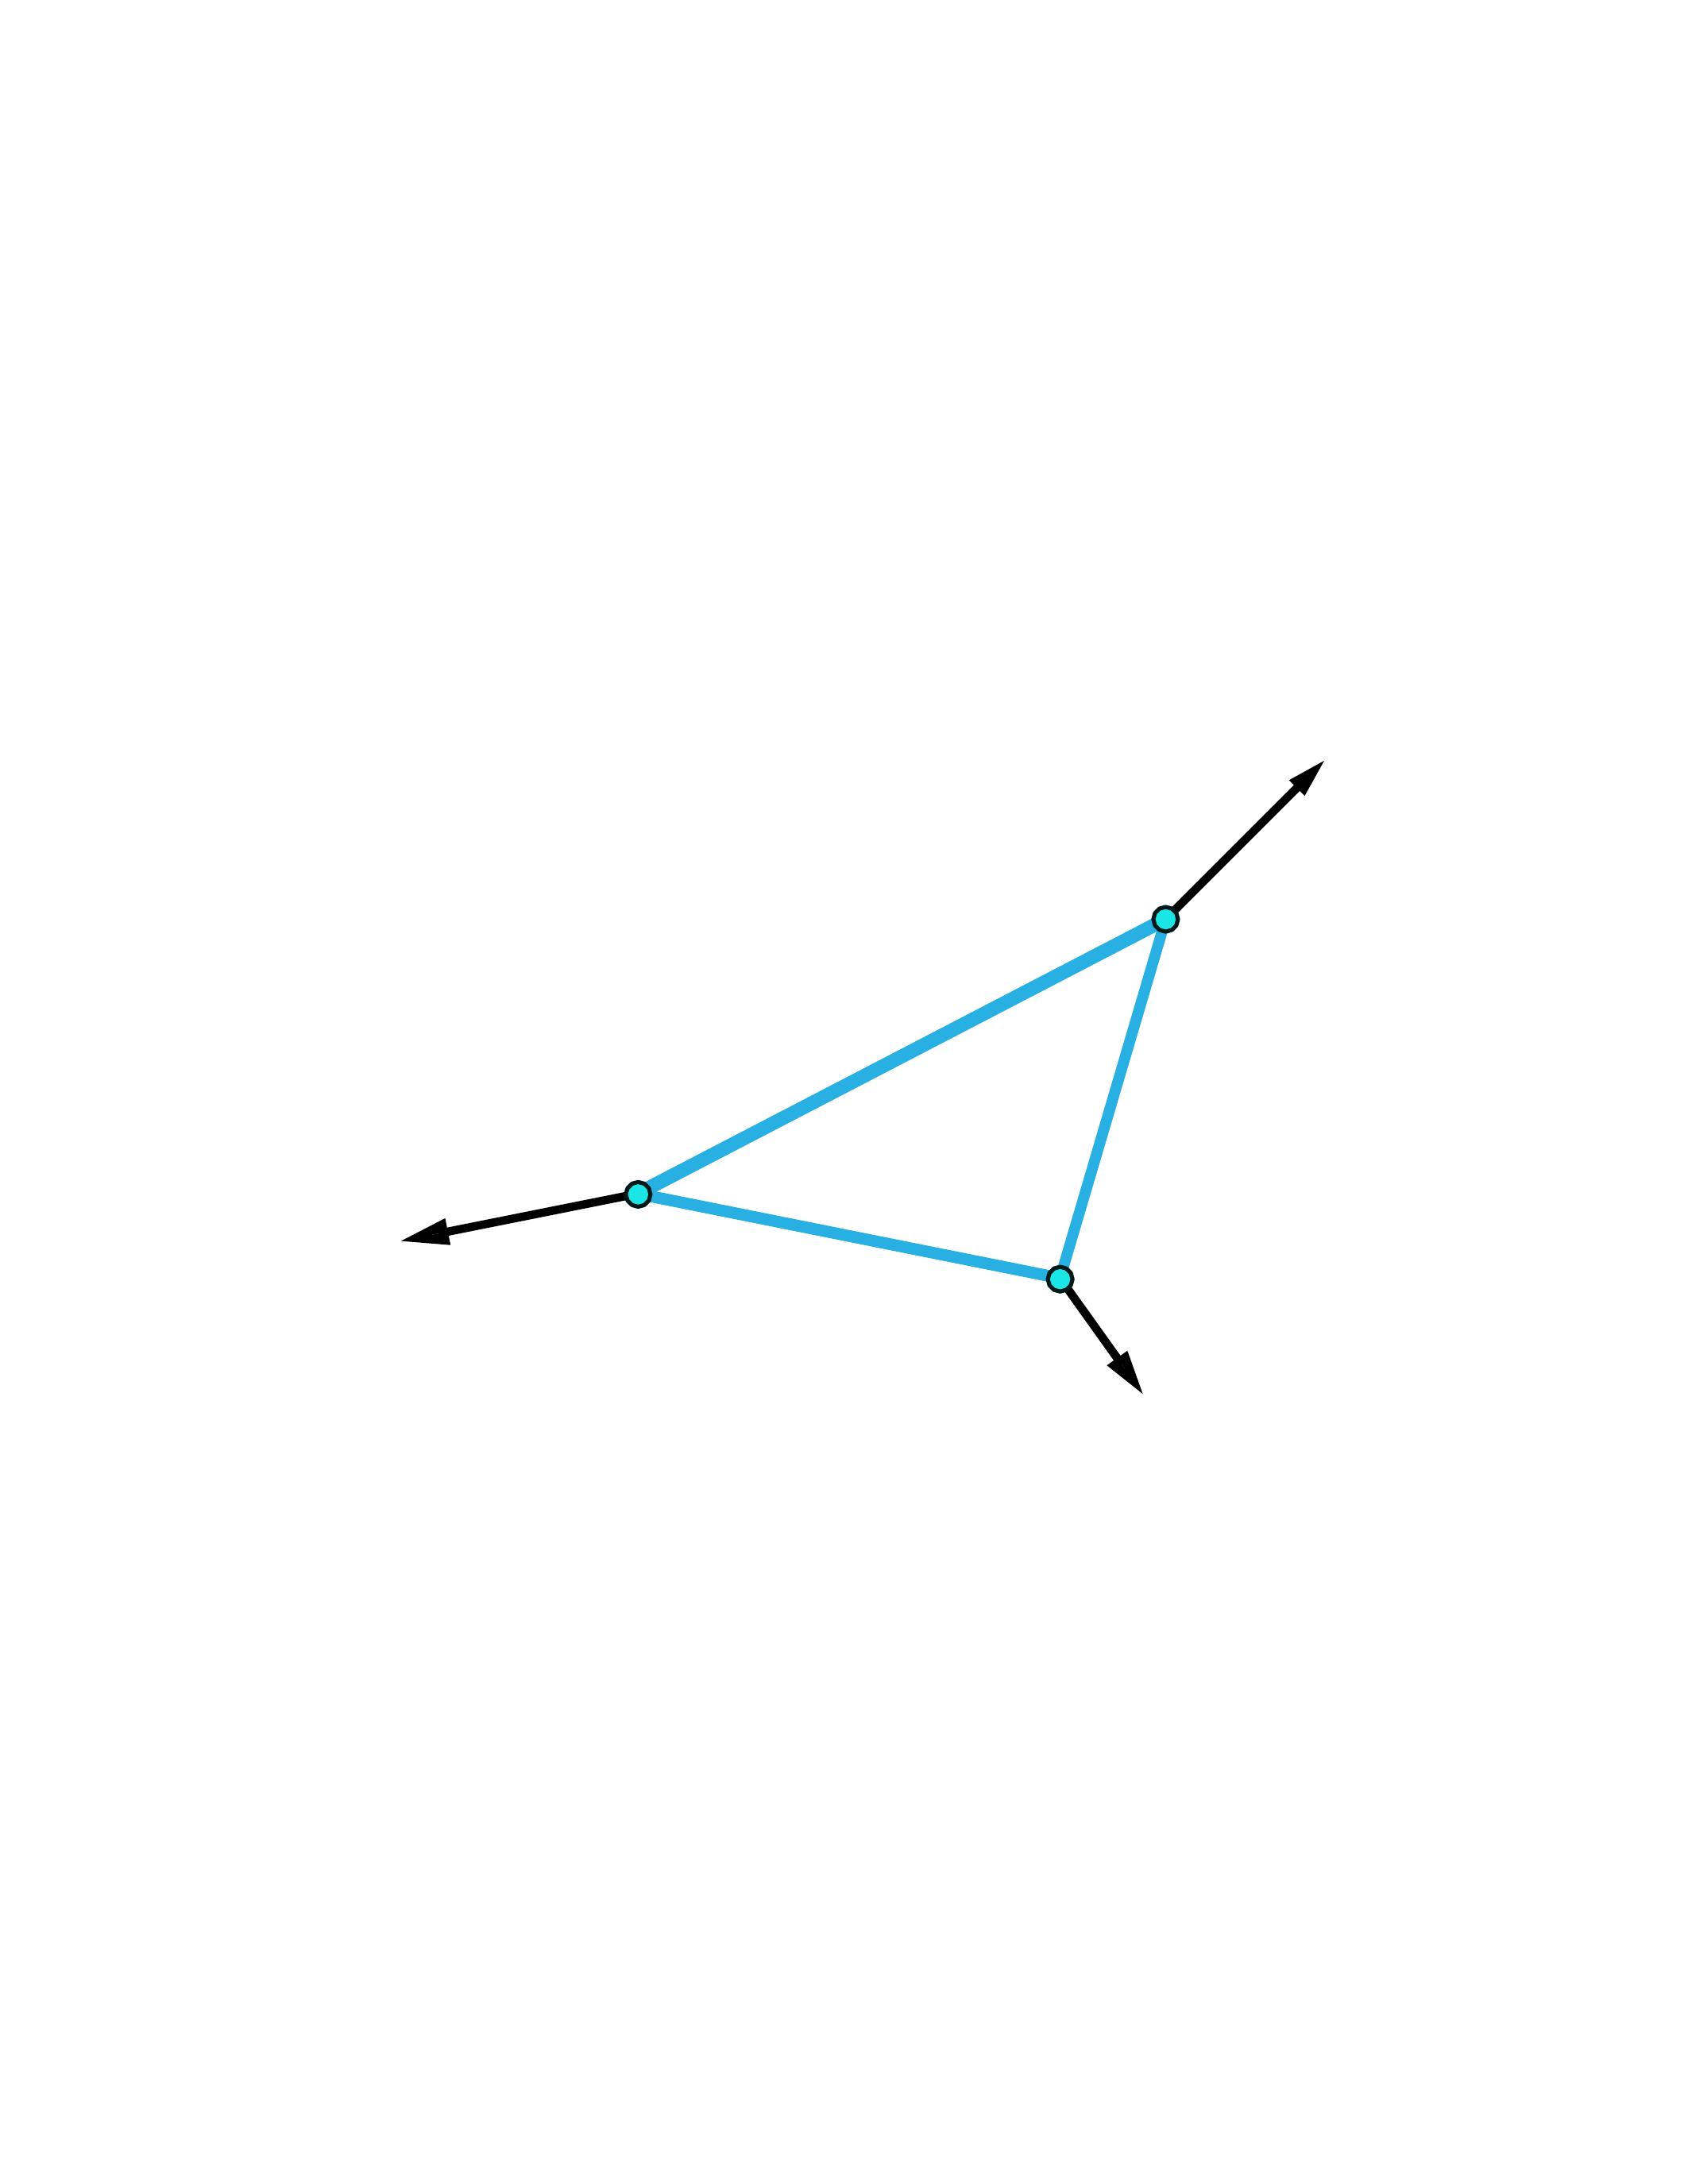}	
			\cput(50,2){\contour{white}{$(a)$}}		
		\end{overpic}
		\begin{overpic}			
			[width=.32\columnwidth,trim={5cm 9cm 4.5cm 9cm},clip]{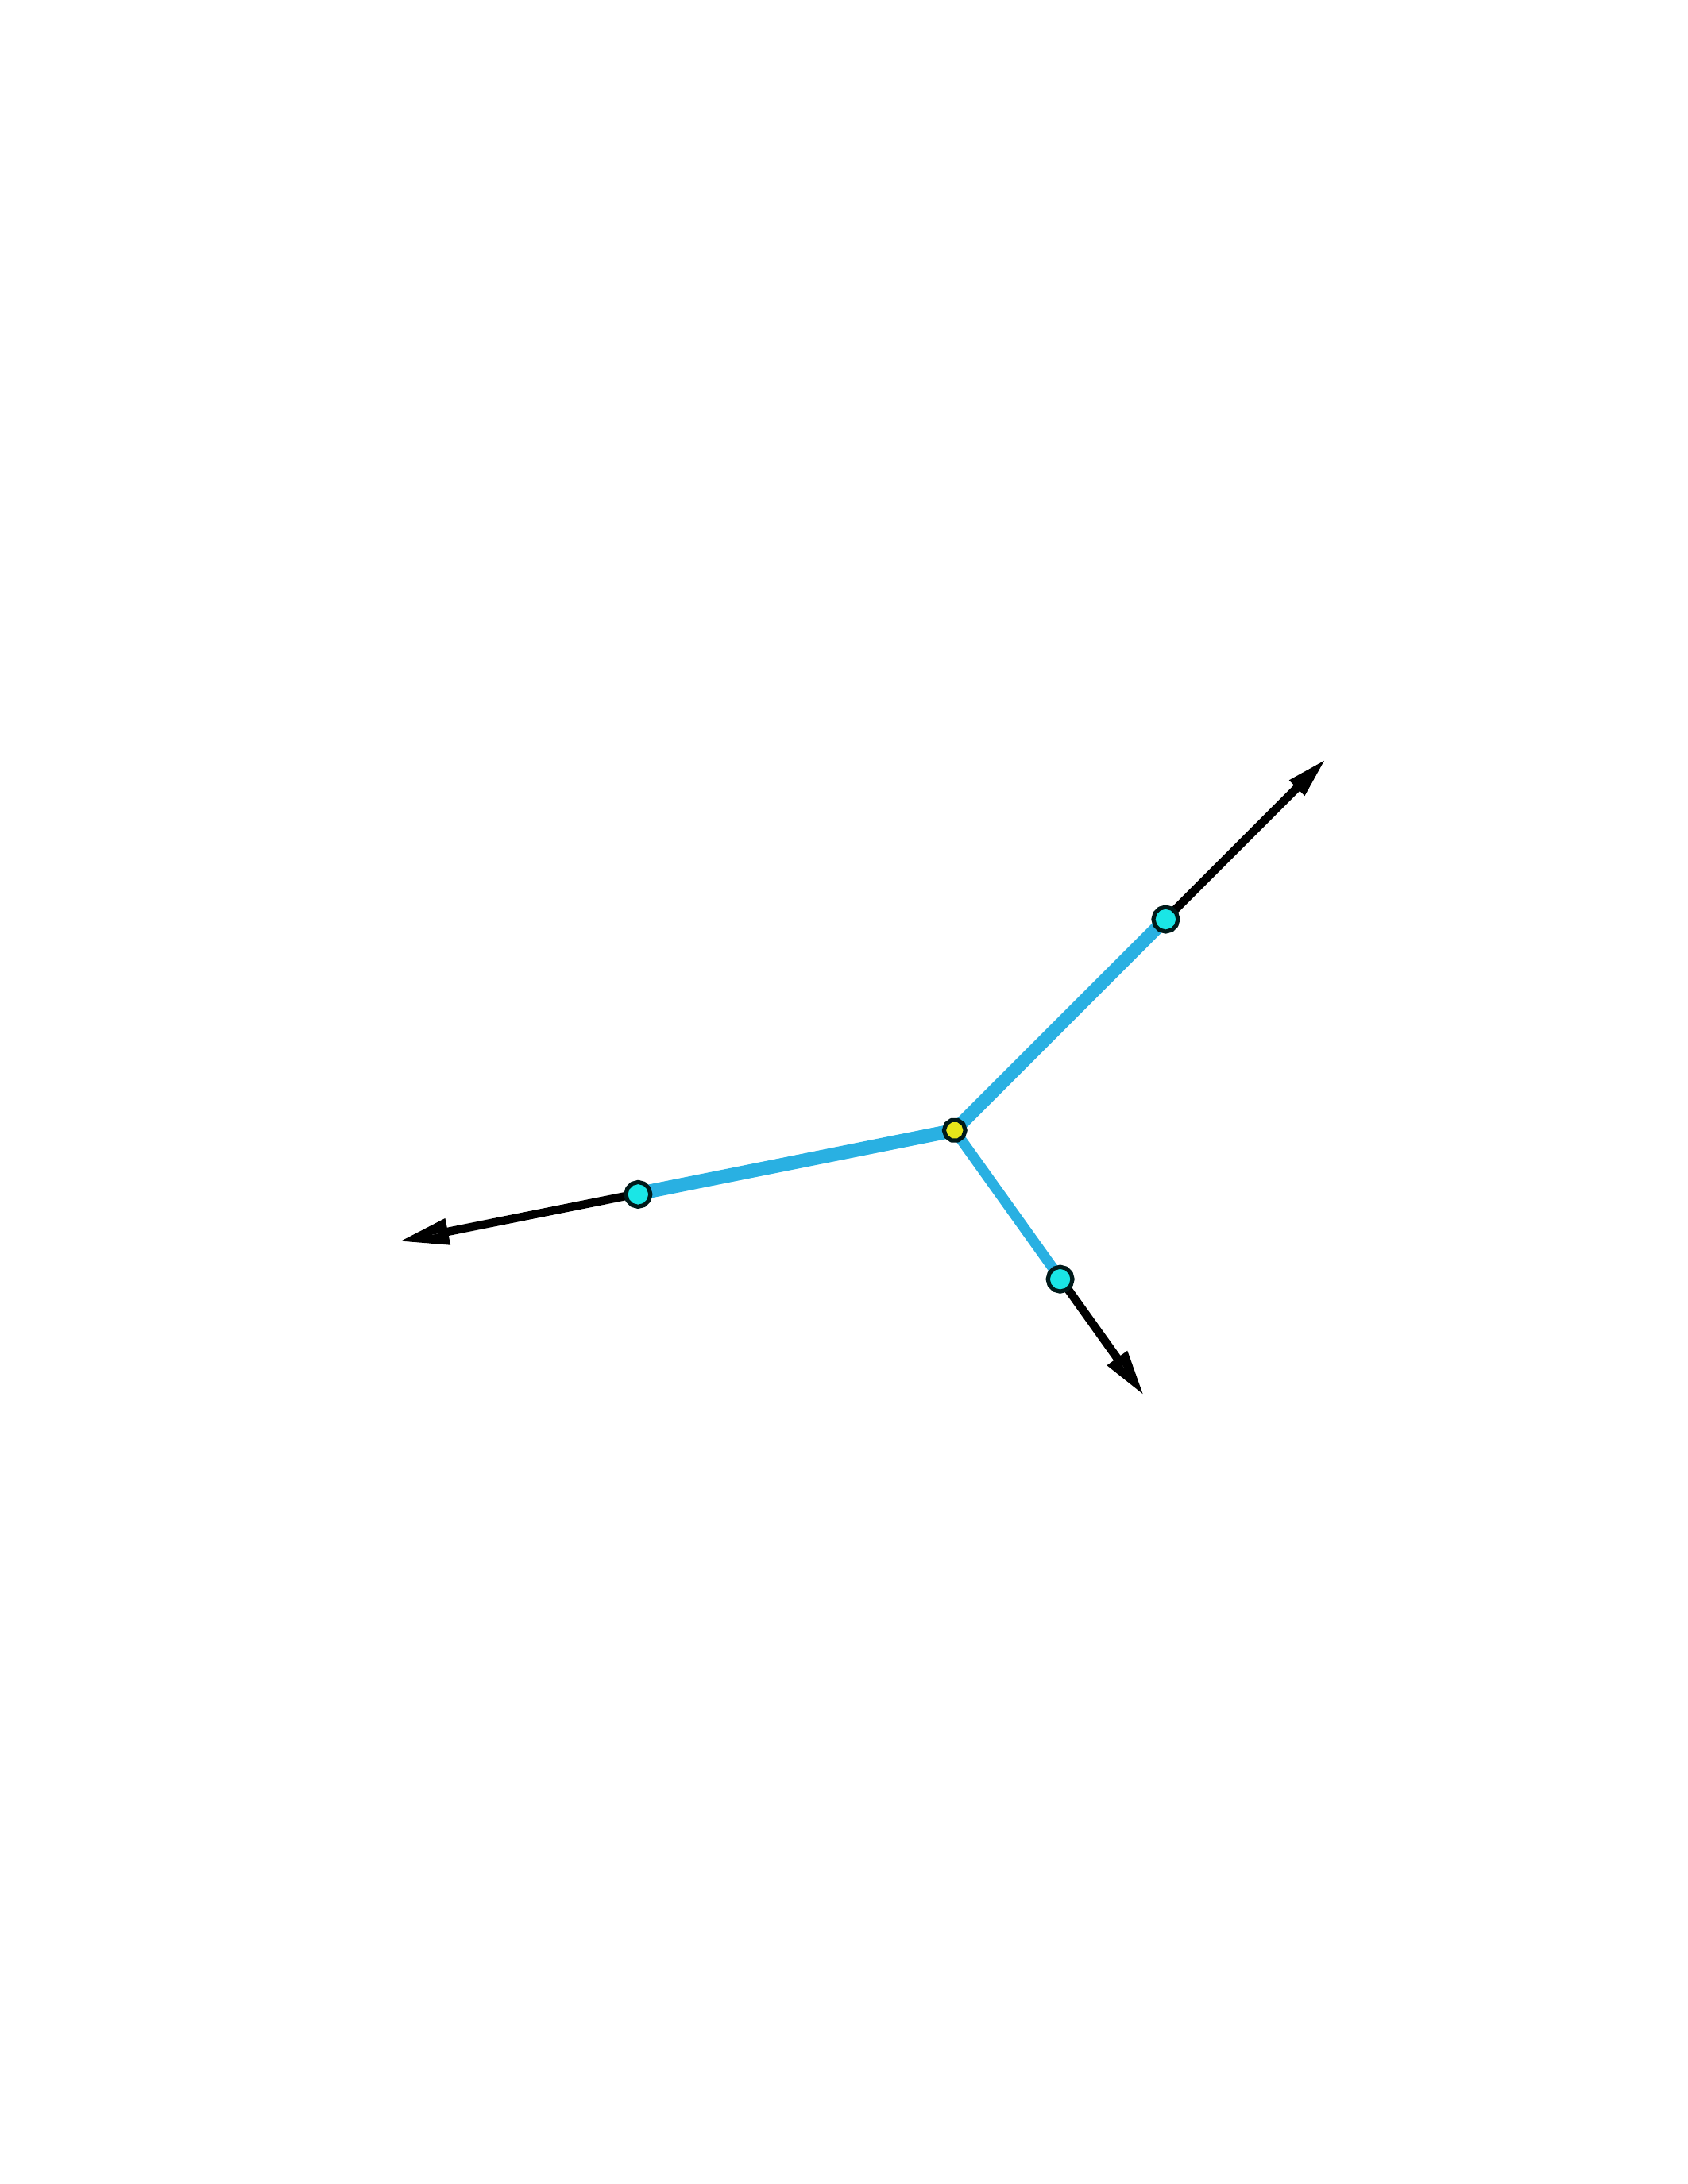}	
			\cput(50,2){\contour{white}{$(b)$}}	
		\end{overpic}
		\begin{overpic}			
			[width=.32\columnwidth,trim={5cm 9cm 4.5cm 9cm},clip]{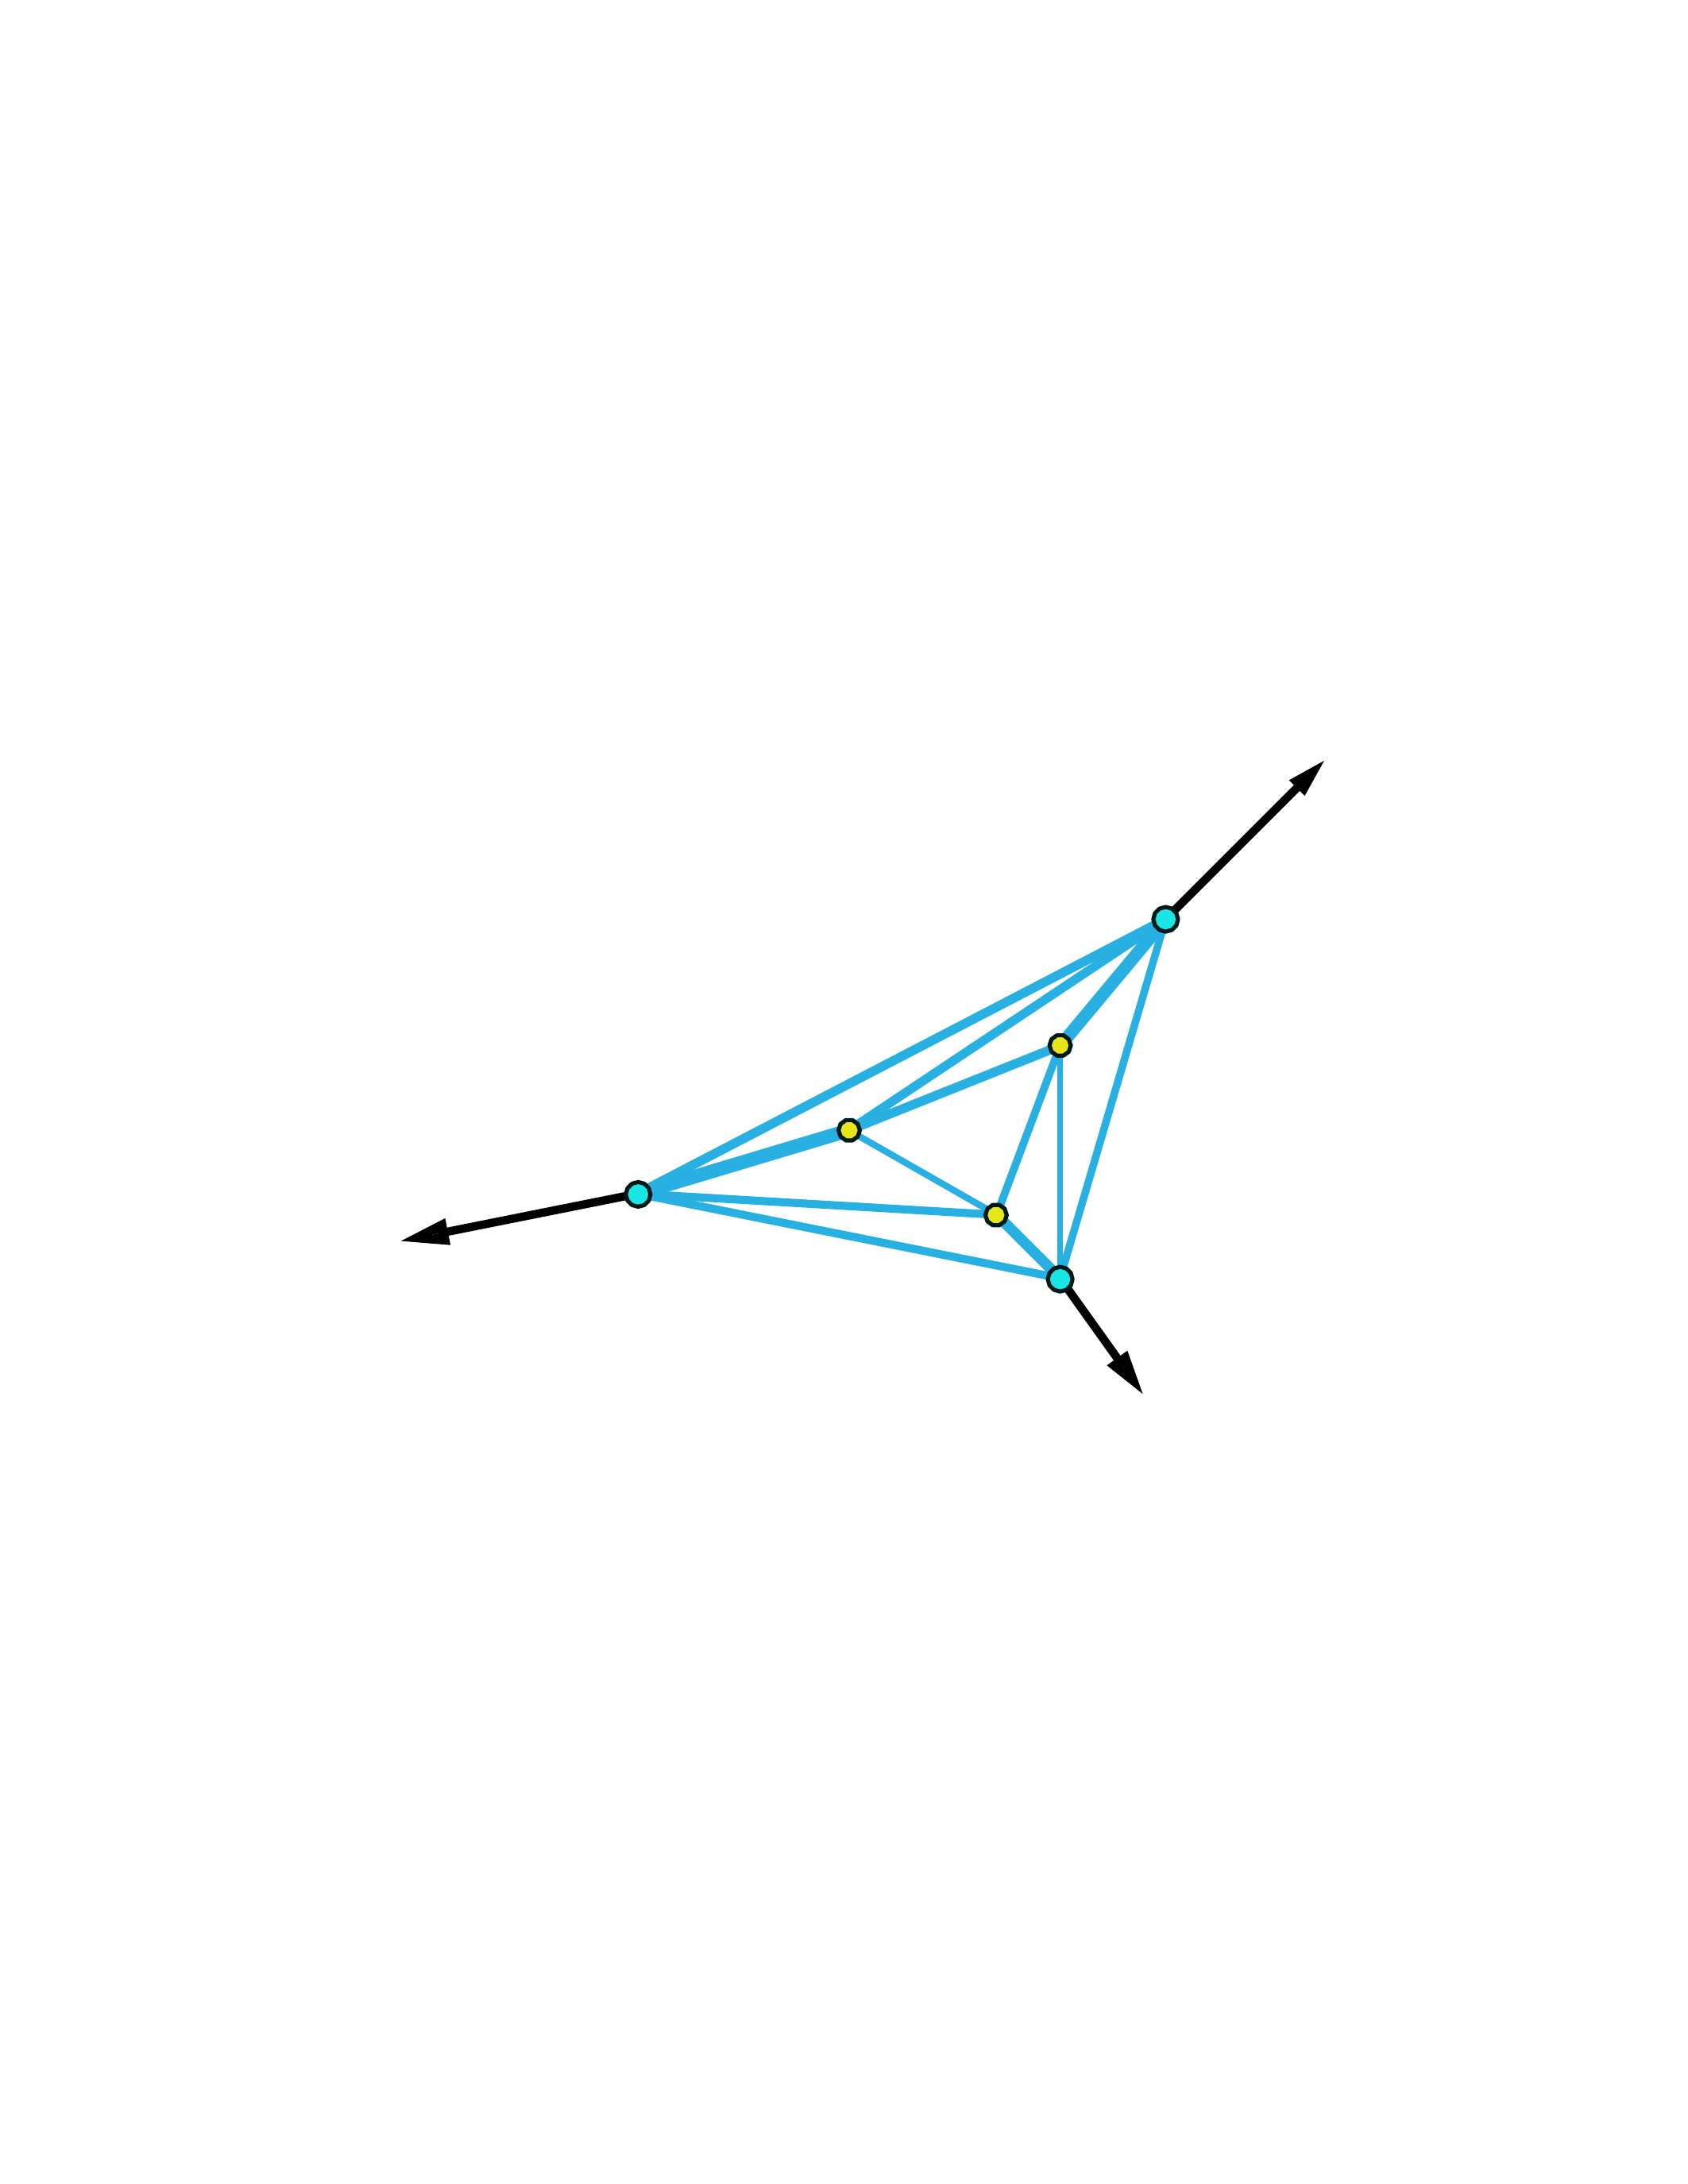}	
			\cput(50,0){\contour{white}{$(c)$}}		
		\end{overpic}
	}	
	\caption{
		\label{fig:nonunique}
		Three different truss designs for the same special boundary condition. These truss use the same amount of material. There are  infinite many such optimal trusses for a special boundary condition. }
\end{figure}

To systematically investigate the functional specifications under which a design with all bars in compression or tension can be found is interesting but out of the scope of this paper. Our numerical computational method can be use to detect such kinds of functional specifications in the coarse truss optimization stage. Under such kinds of special functional specifications, further subdivision is not necessary.
\clearpage
\section*{Additional Results}
In addition to the examples shown in the paper, additional results are provided below.

%\clearpage
\begin{figure*}[tb]\centering{
		\begin{overpic}			
			[width=1.3\columnwidth,trim={2cm 8cm 2cm 8cm},clip]{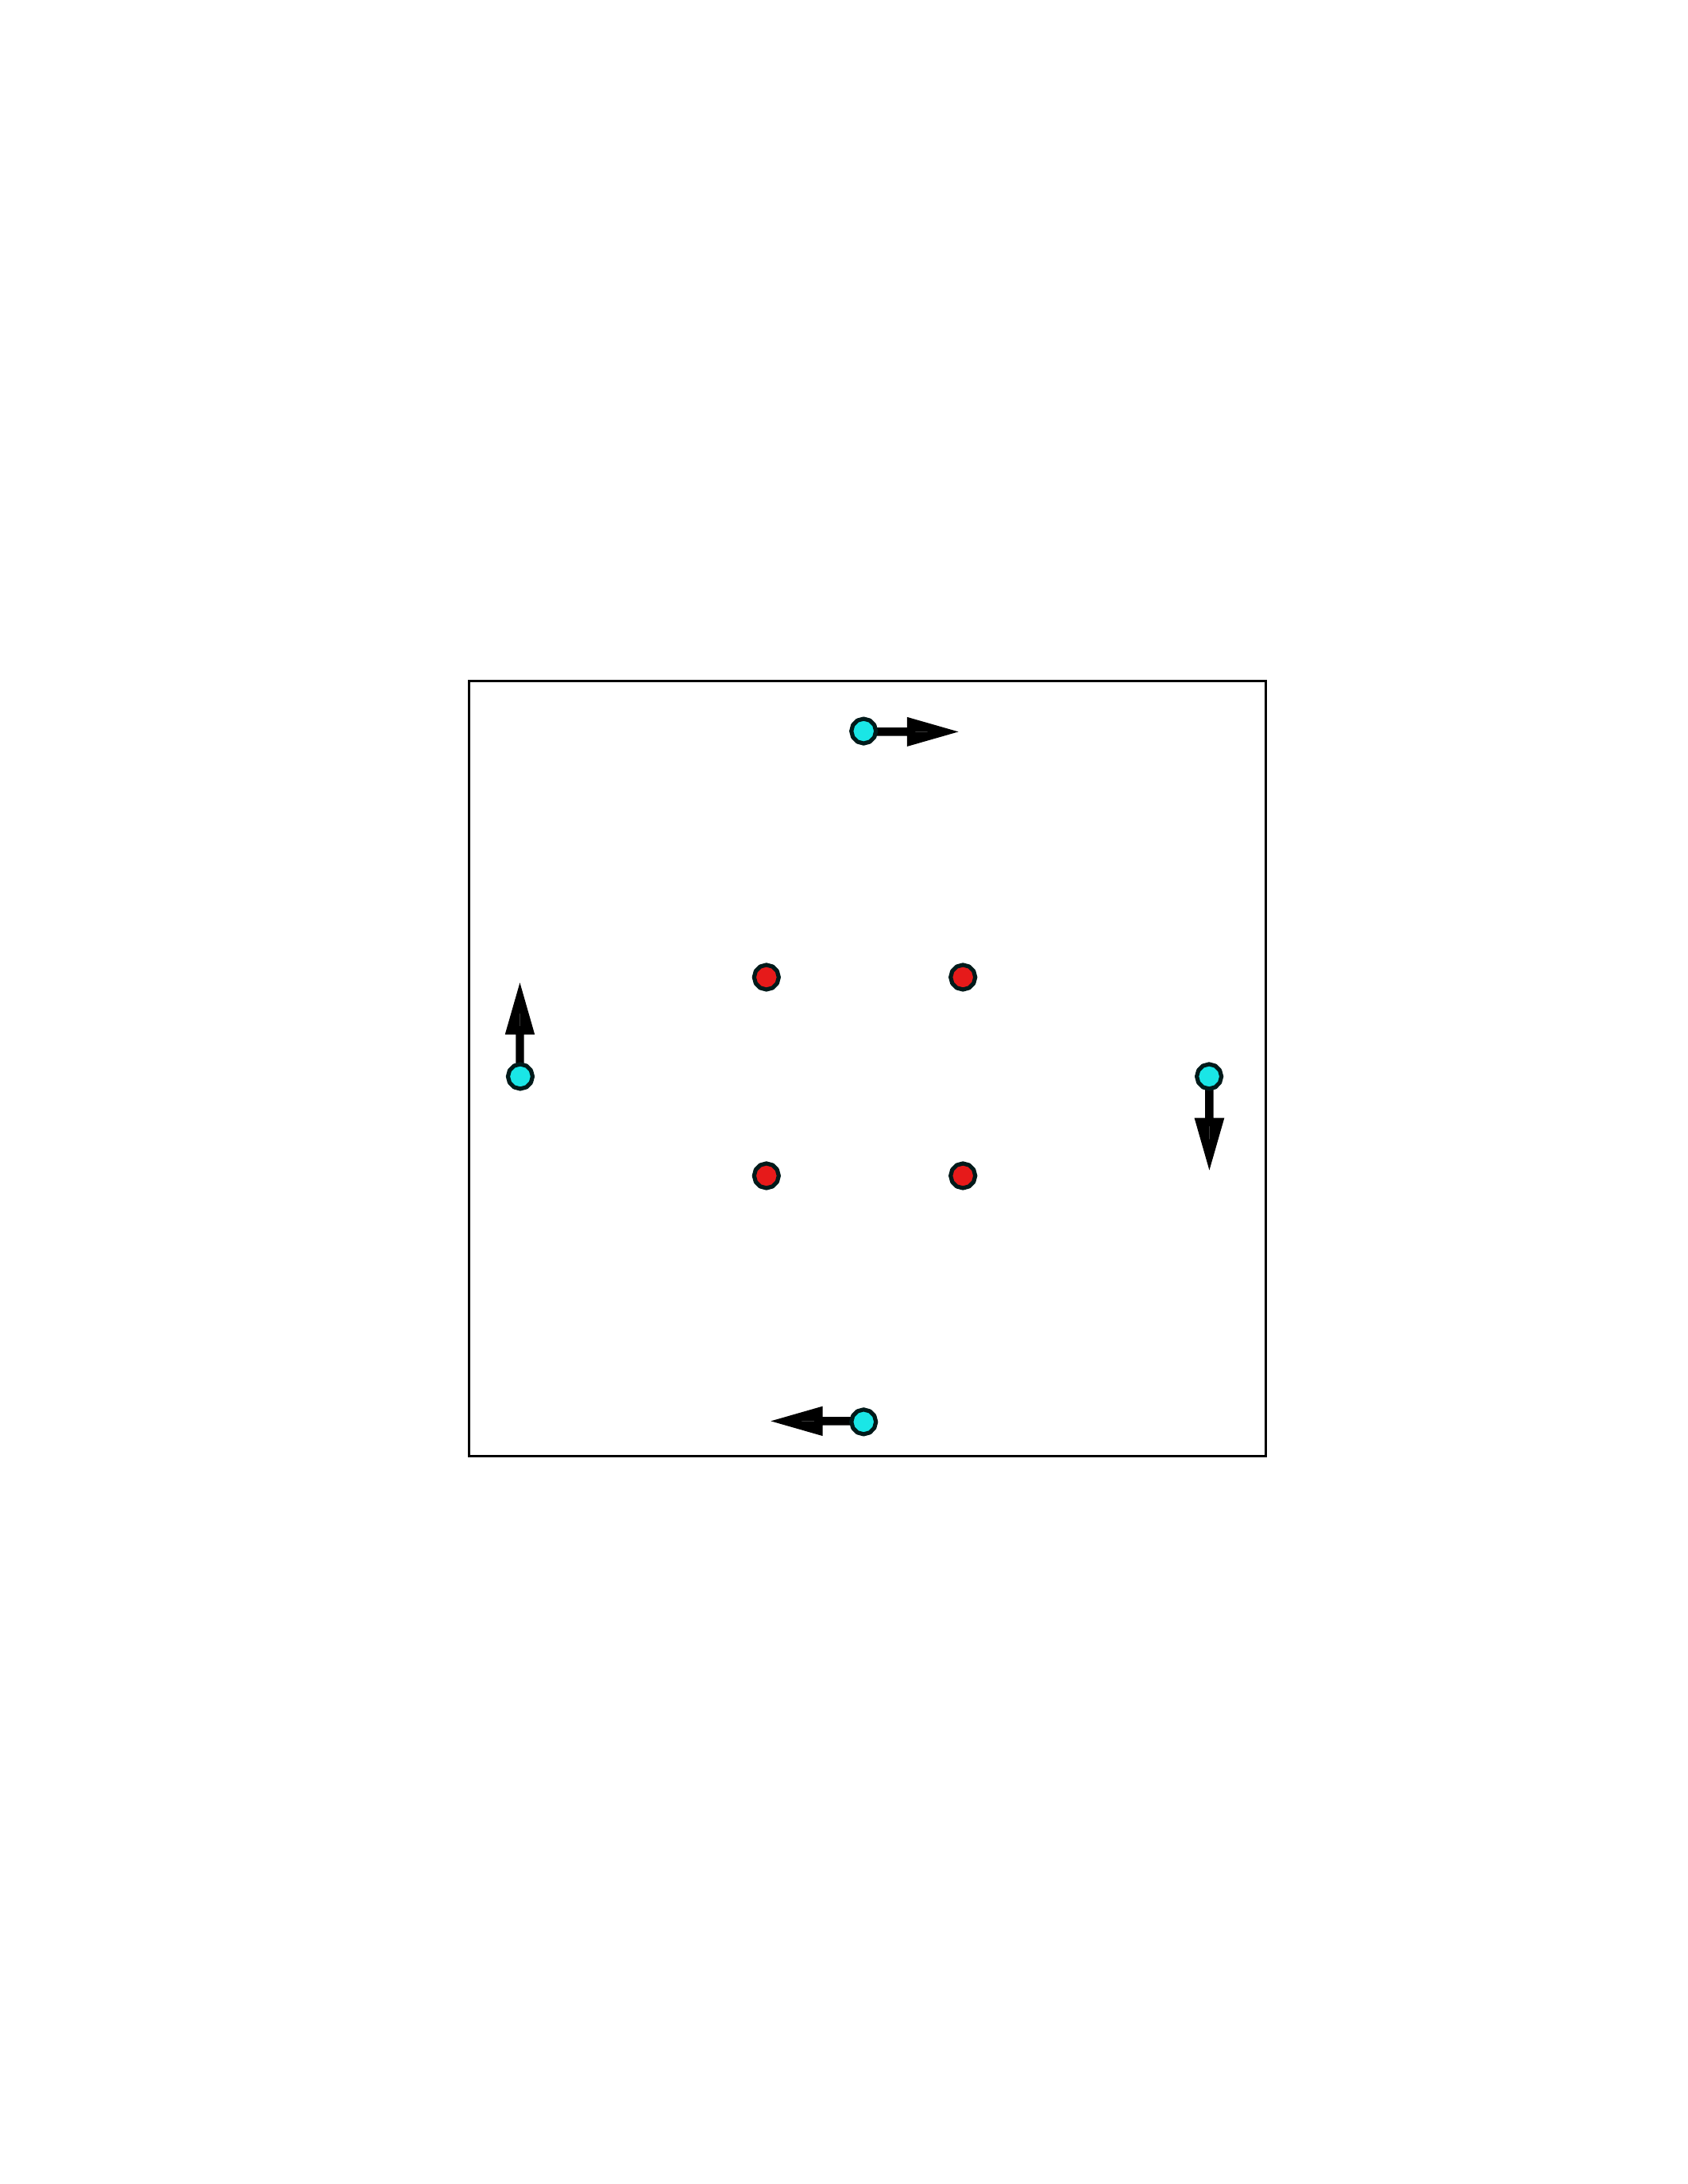}	
			\cput(50,2){\contour{white}{$(a)$}}		
		\end{overpic}
		\begin{overpic}			
			[width=0.8\columnwidth,trim={12cm 2cm 12cm 2cm},clip]{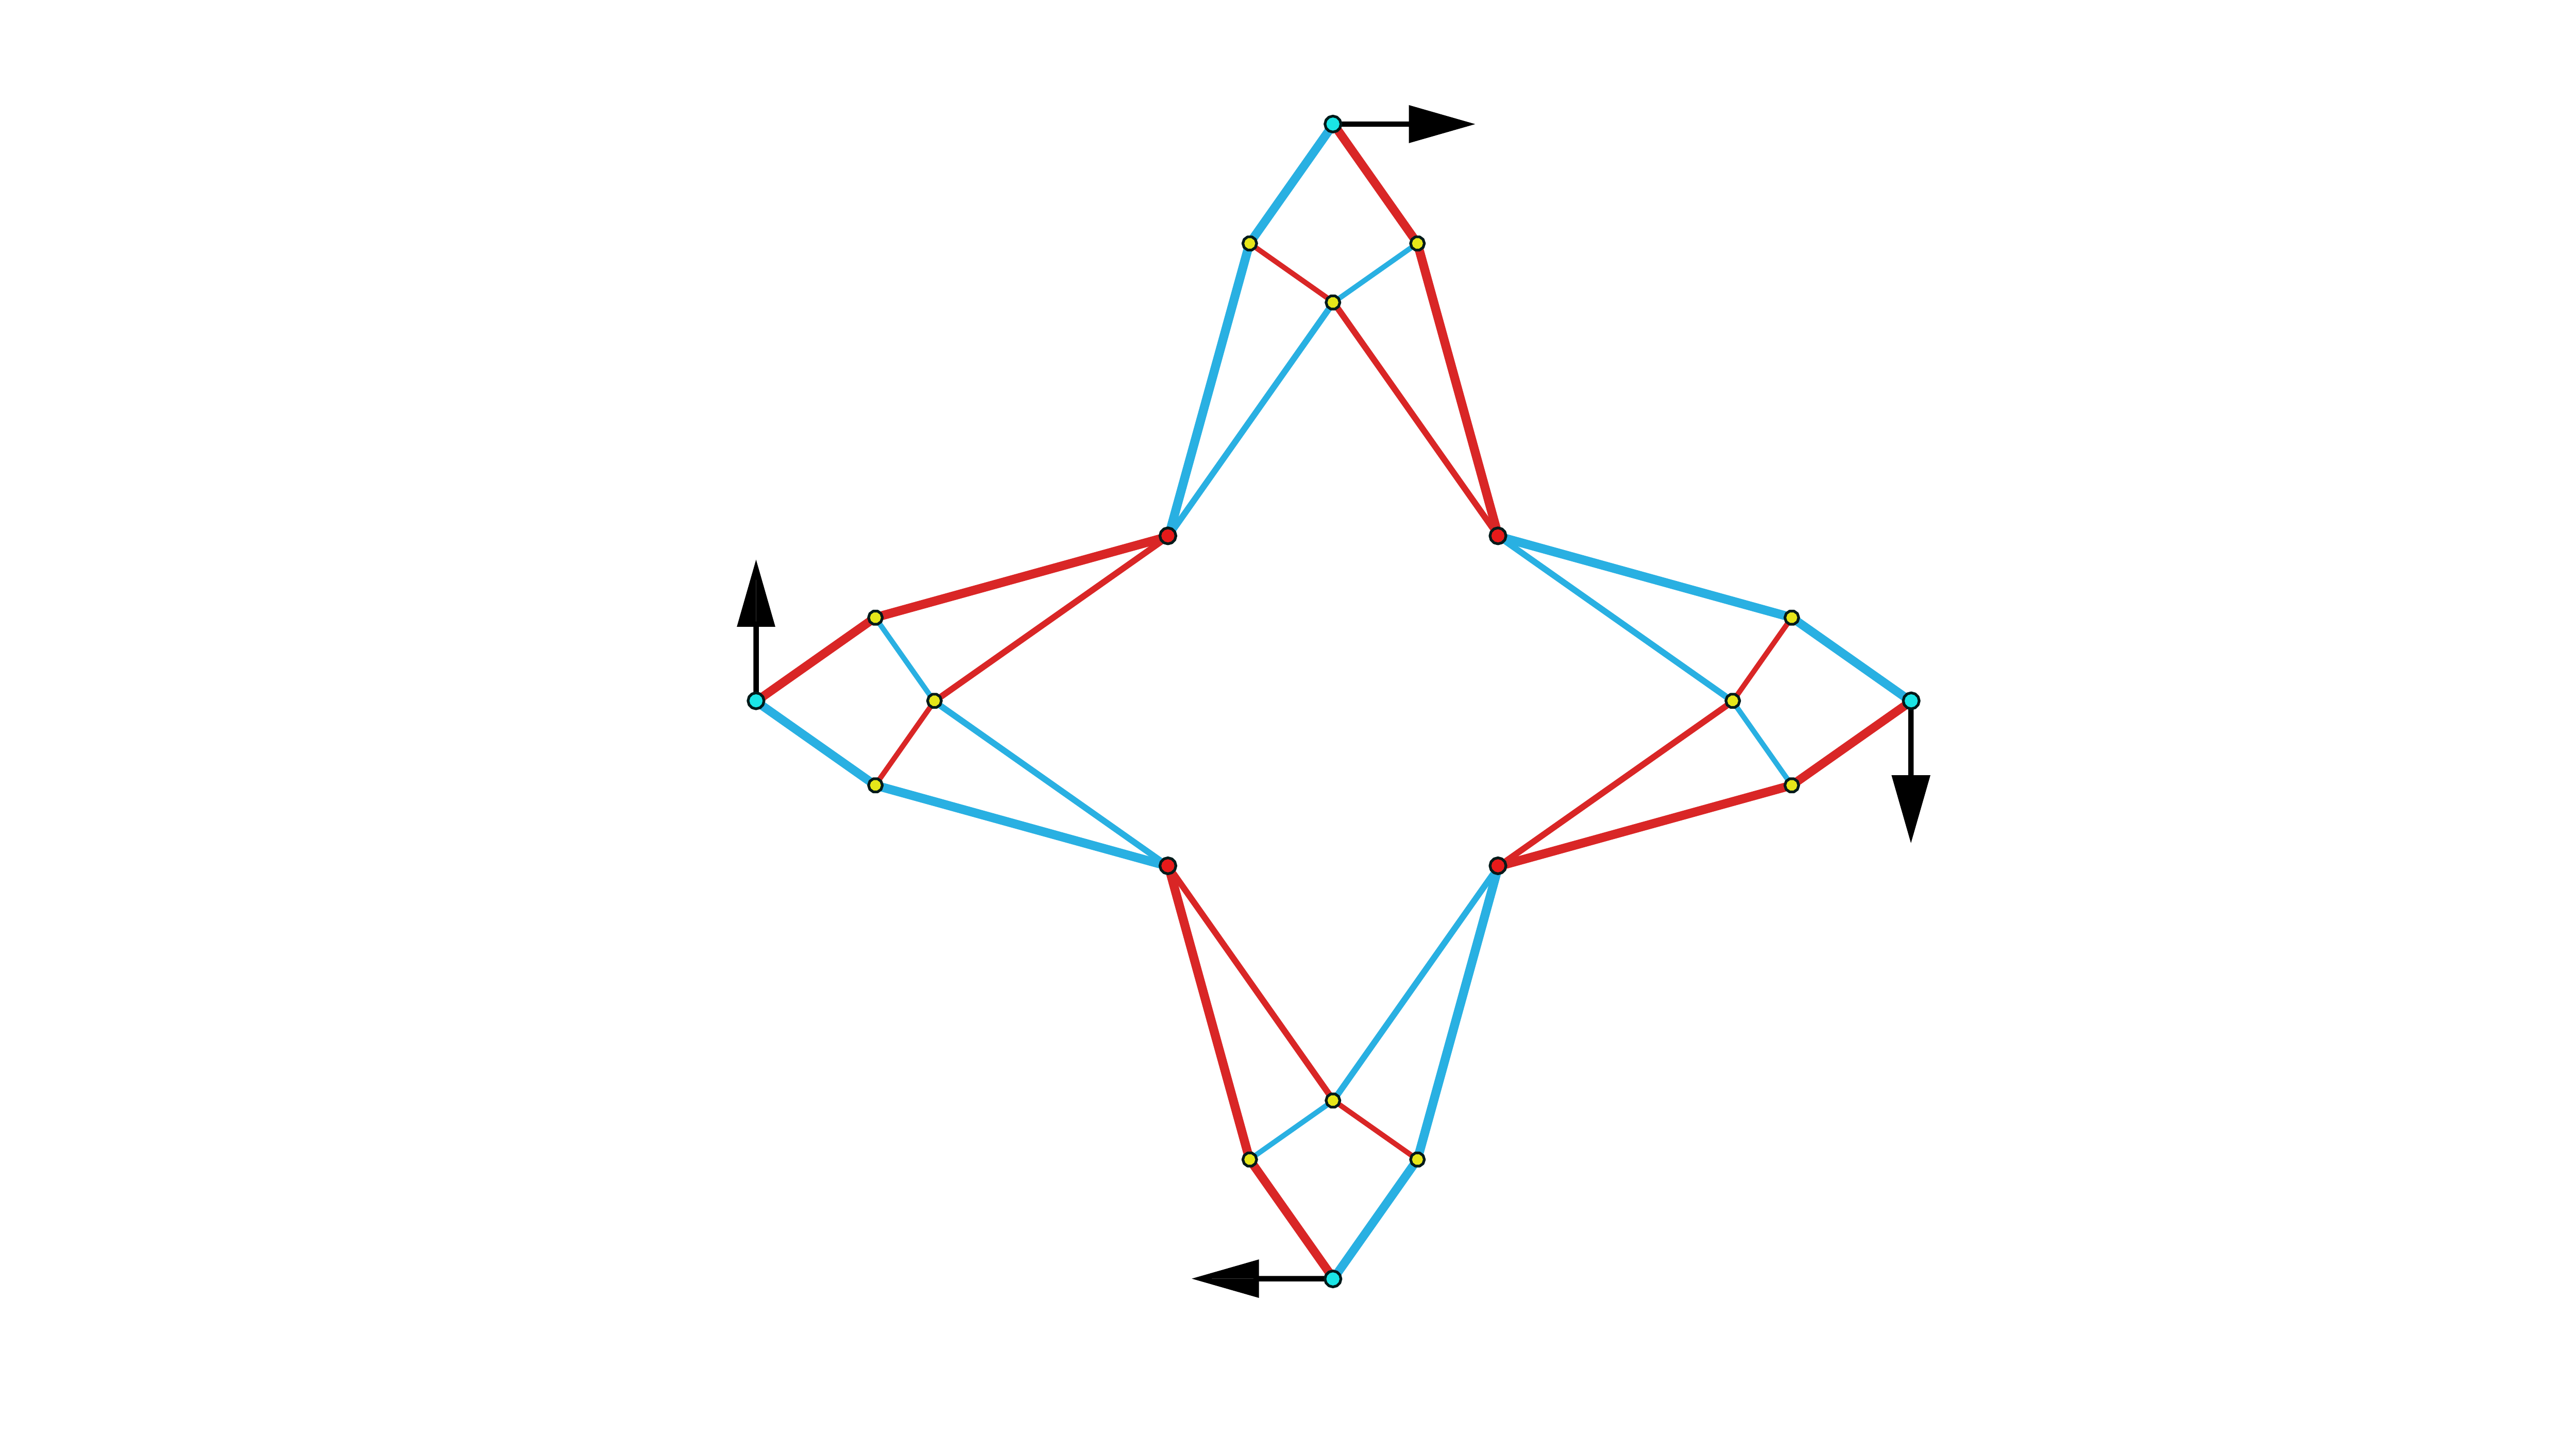}	
			\cput(50,2){\contour{white}{$(b)$}}	
		\end{overpic}
		\begin{overpic}			
			[width=0.8\columnwidth,trim={12cm 2cm 12cm 2cm},clip]{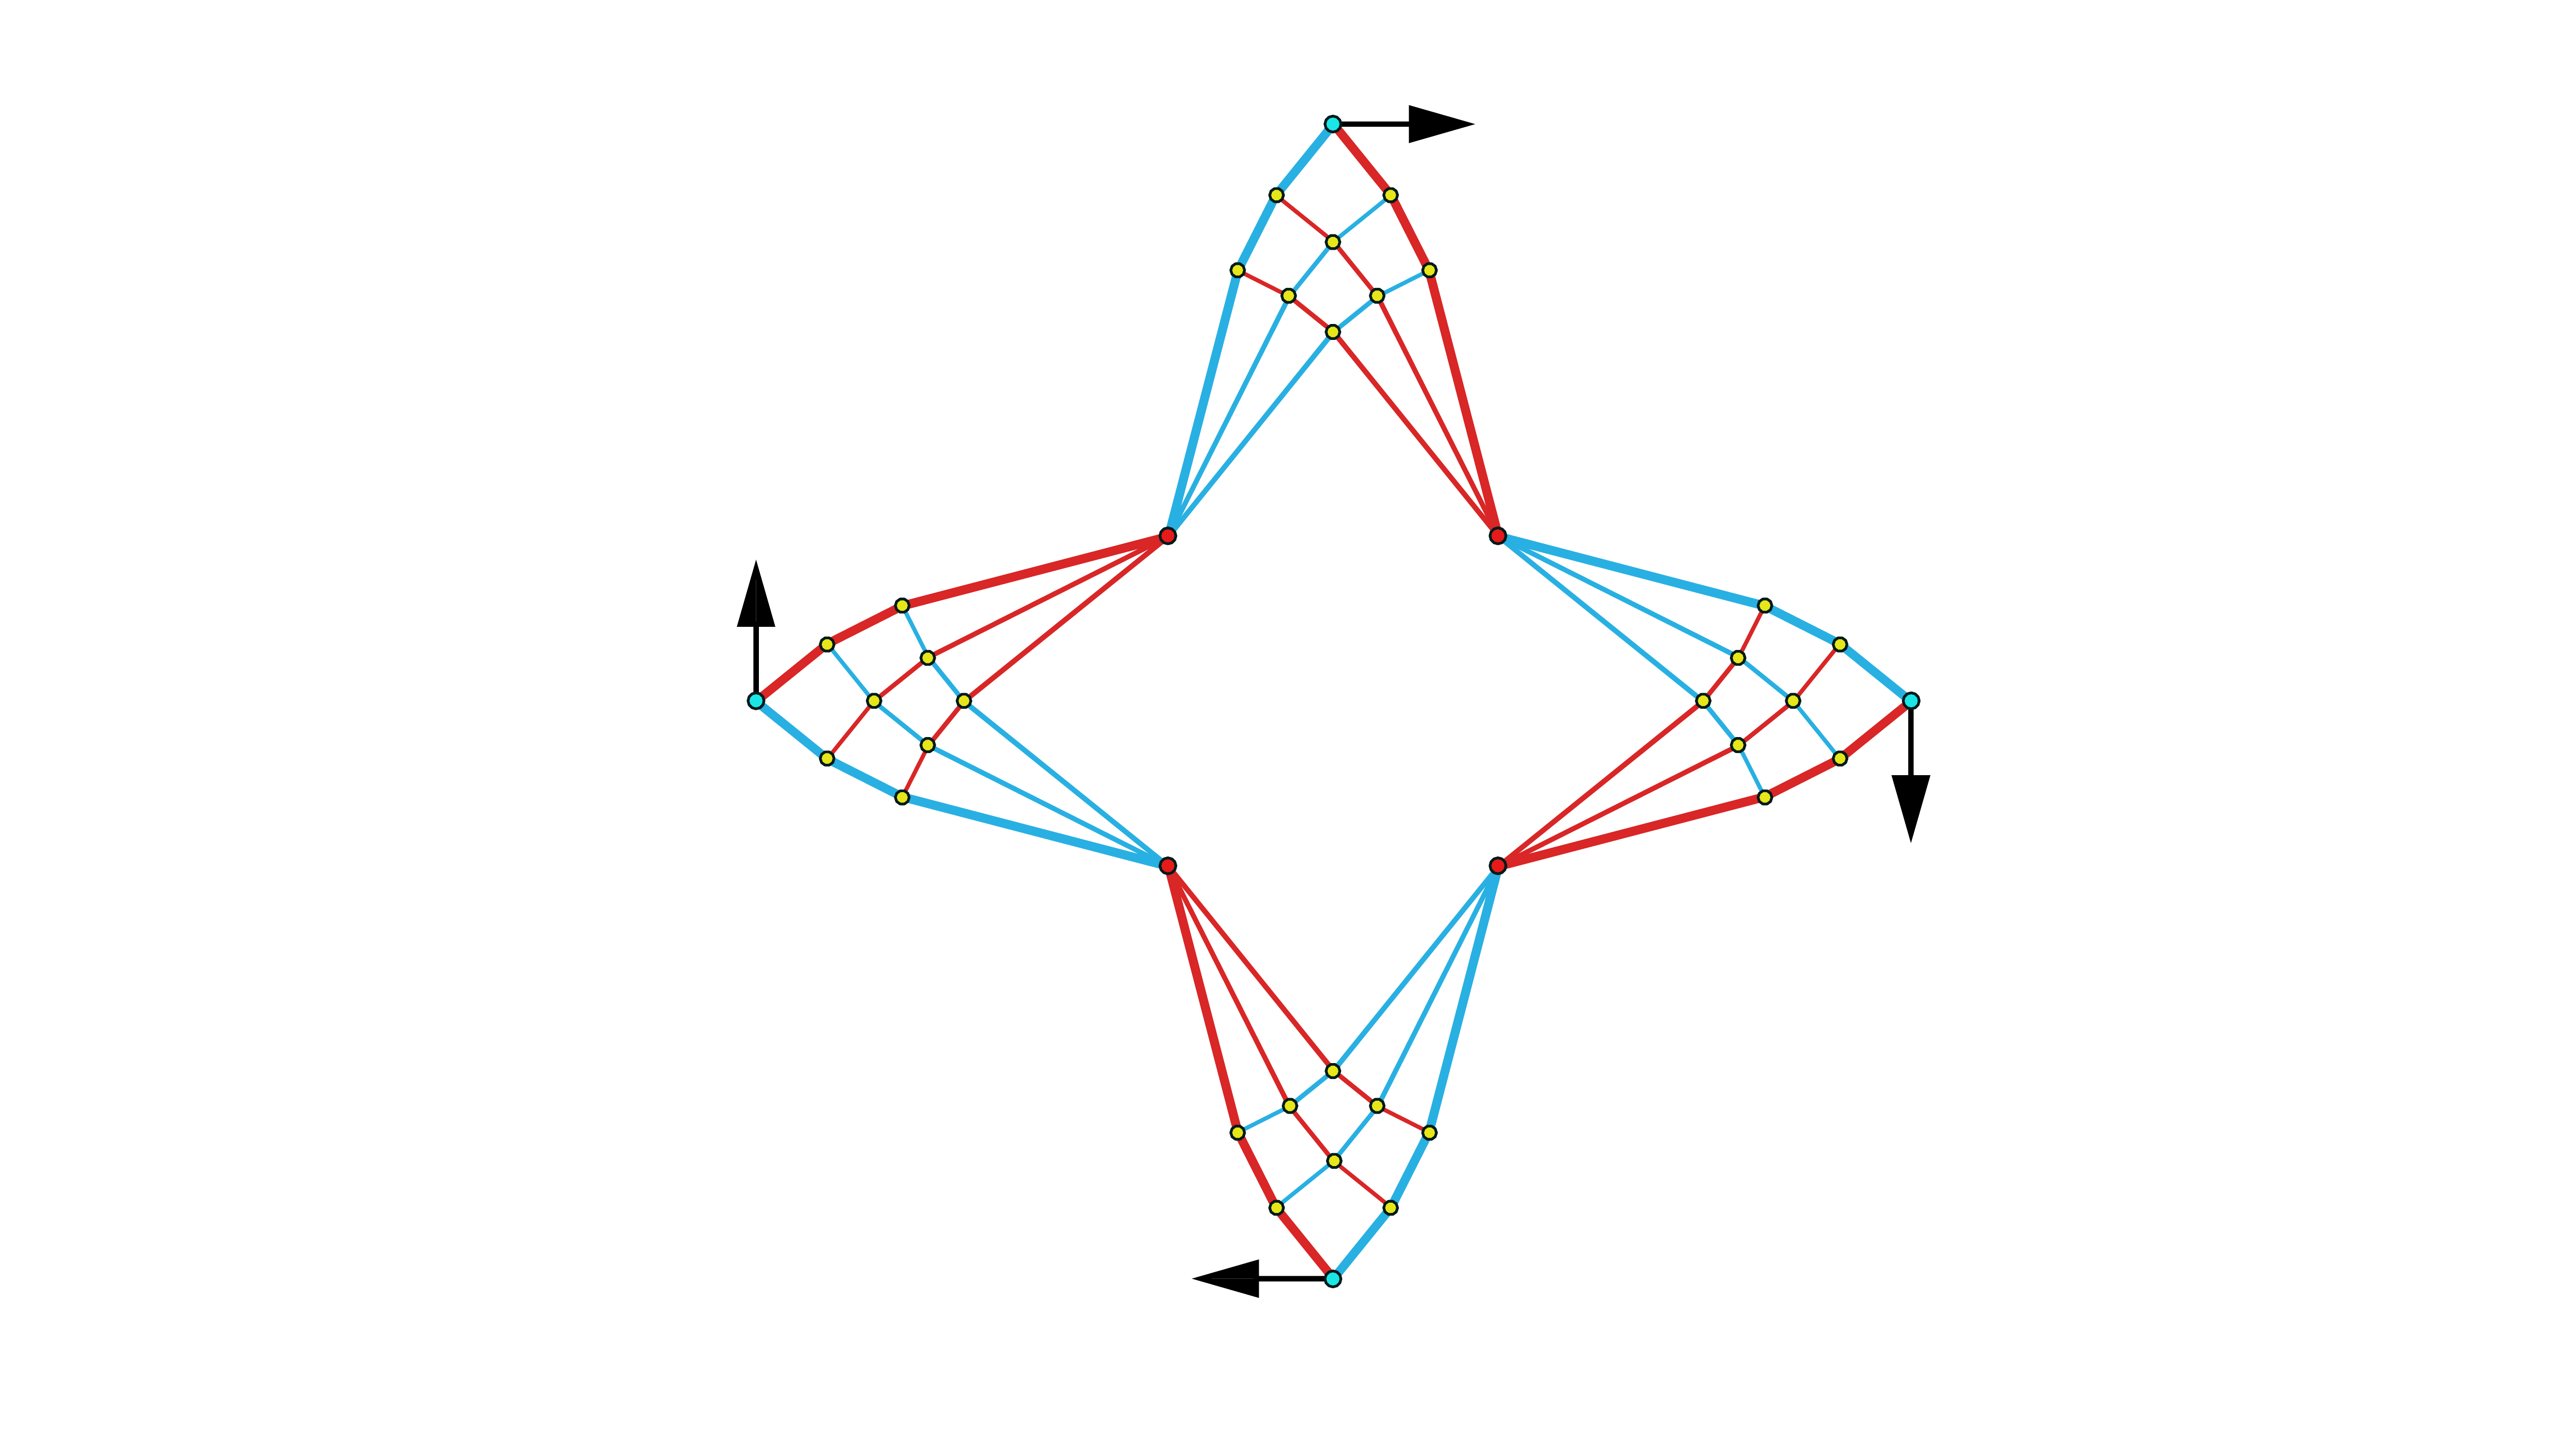}	
			\cput(50,2){\contour{white}{$(c)$}}	
		\end{overpic}
		\begin{overpic}			
			[width=0.8\columnwidth,trim={12cm 2cm 12cm 2cm},clip]{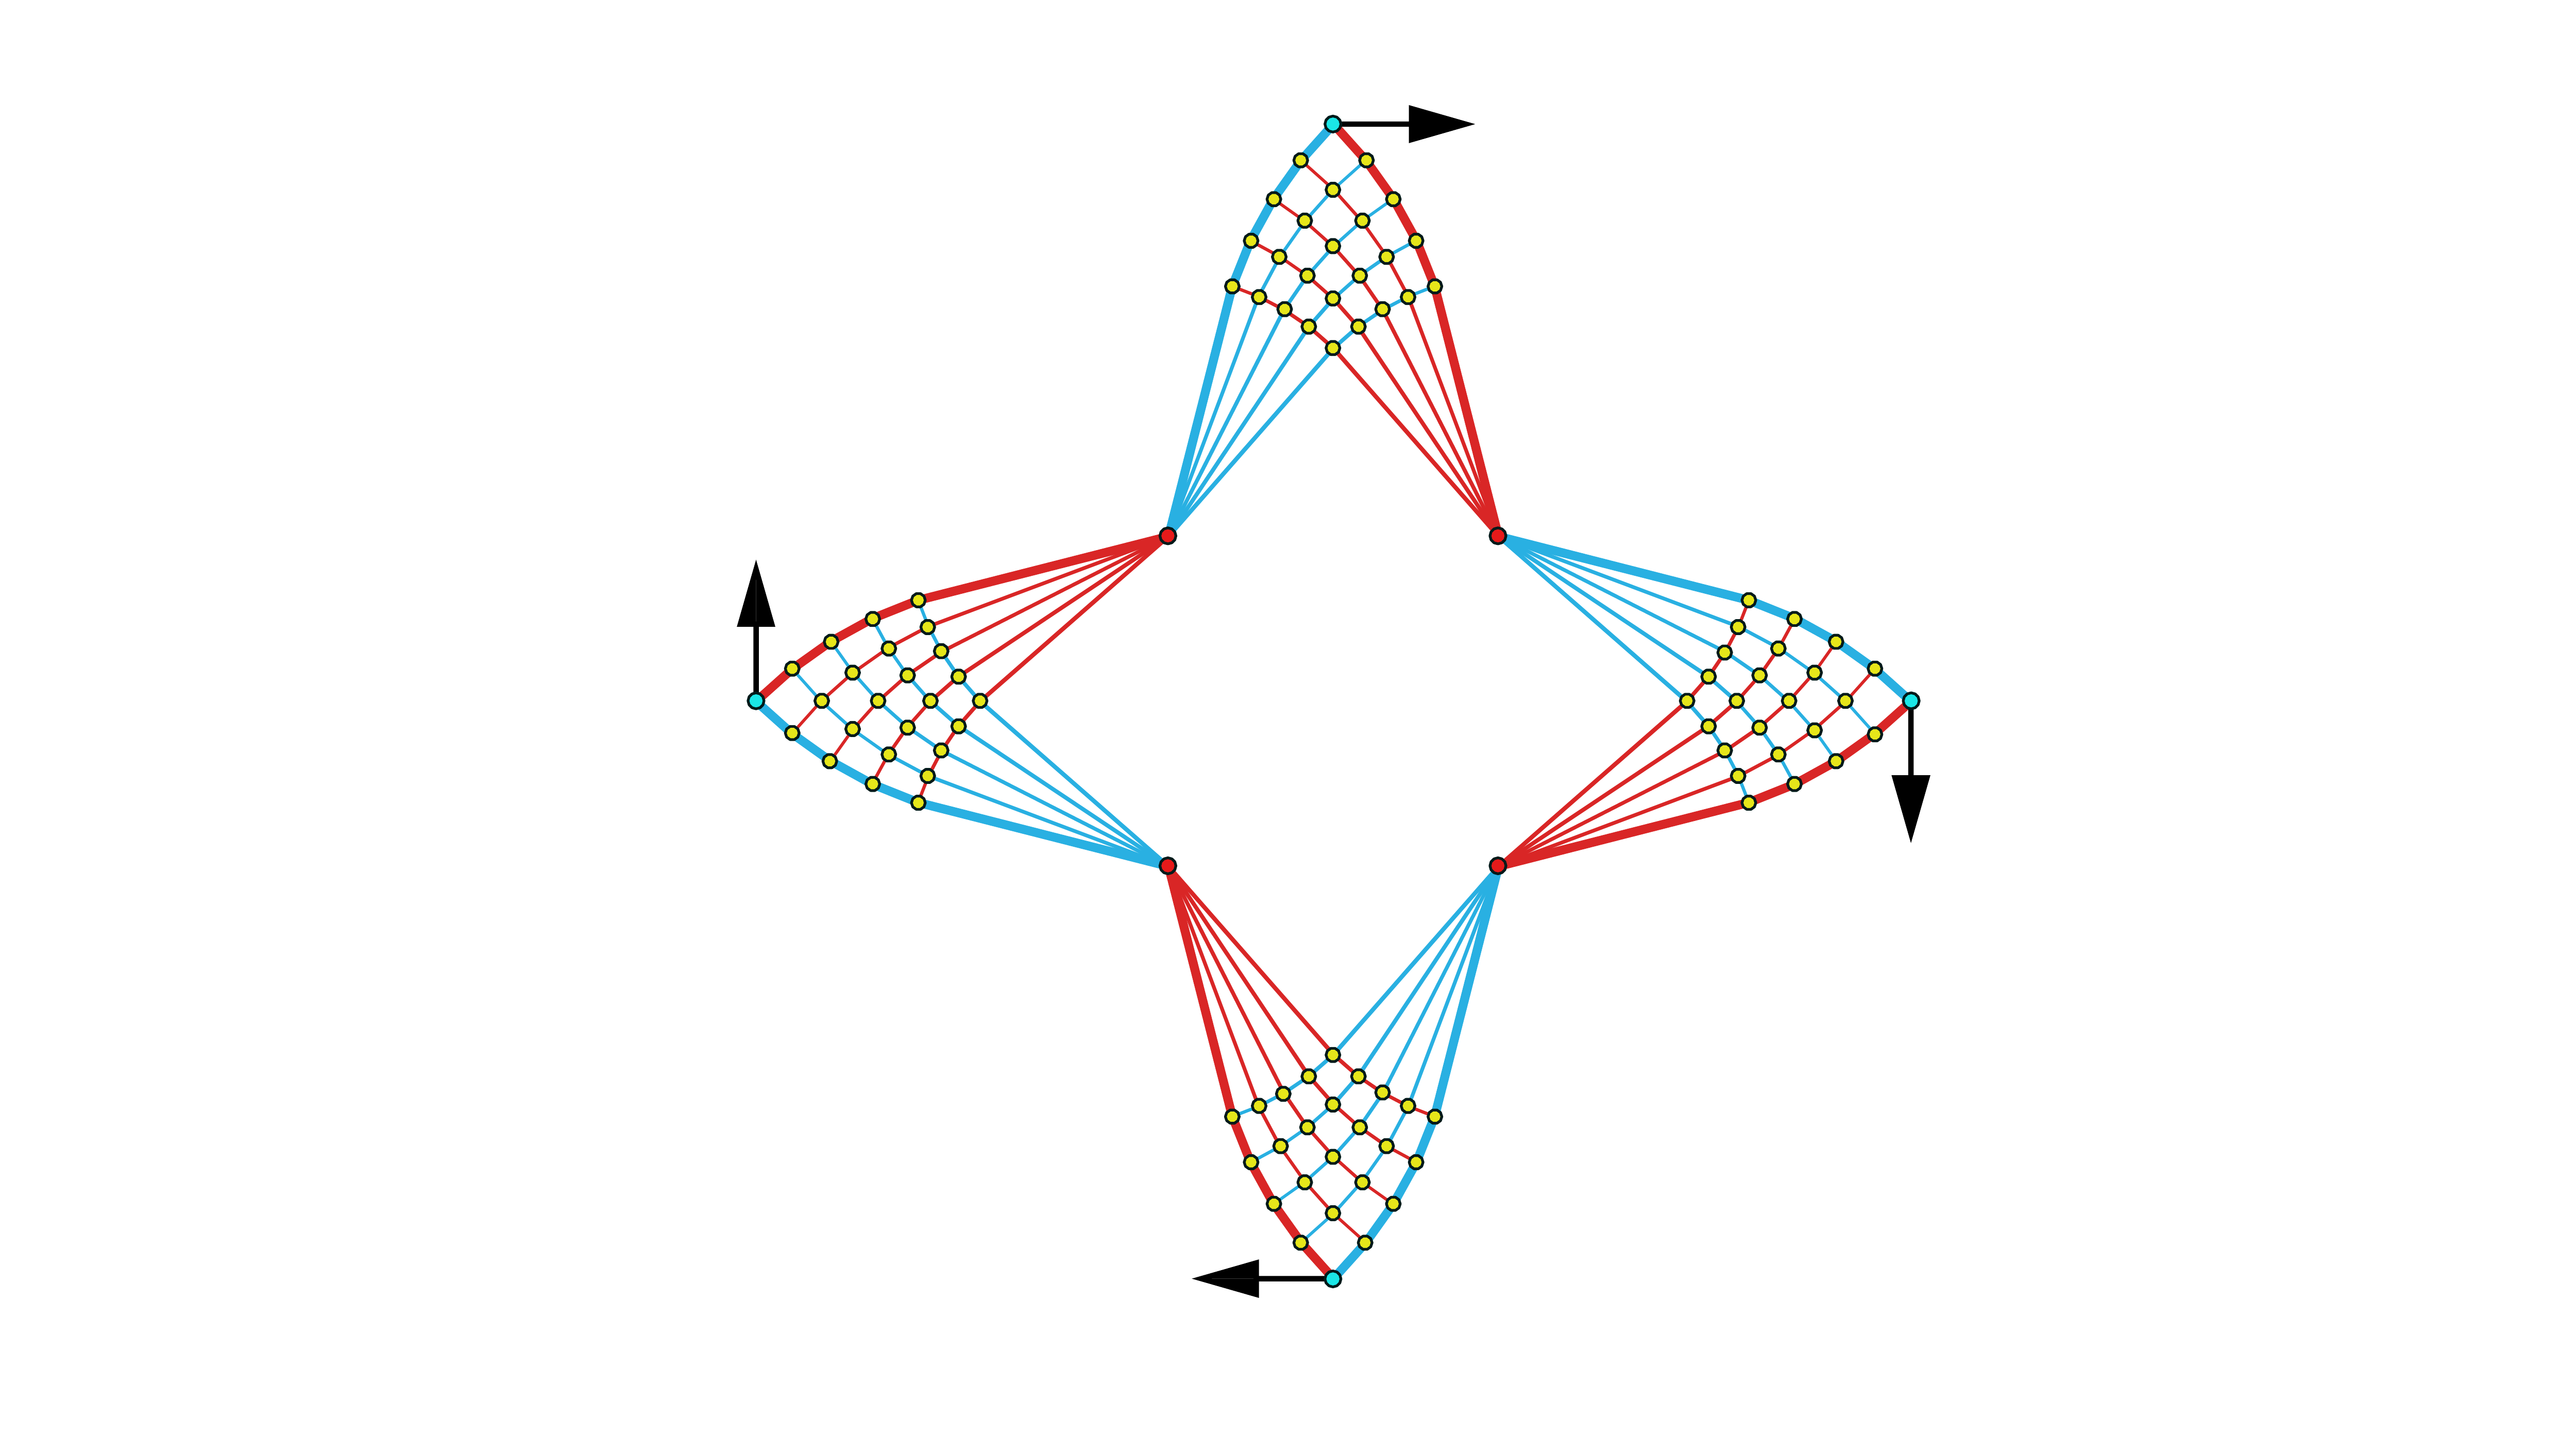}	
			\cput(50,2){\contour{white}{$(d)$}}	
		\end{overpic}
		\begin{overpic}			
			[width=0.8\columnwidth,trim={12cm 2cm 12cm 2cm},clip]{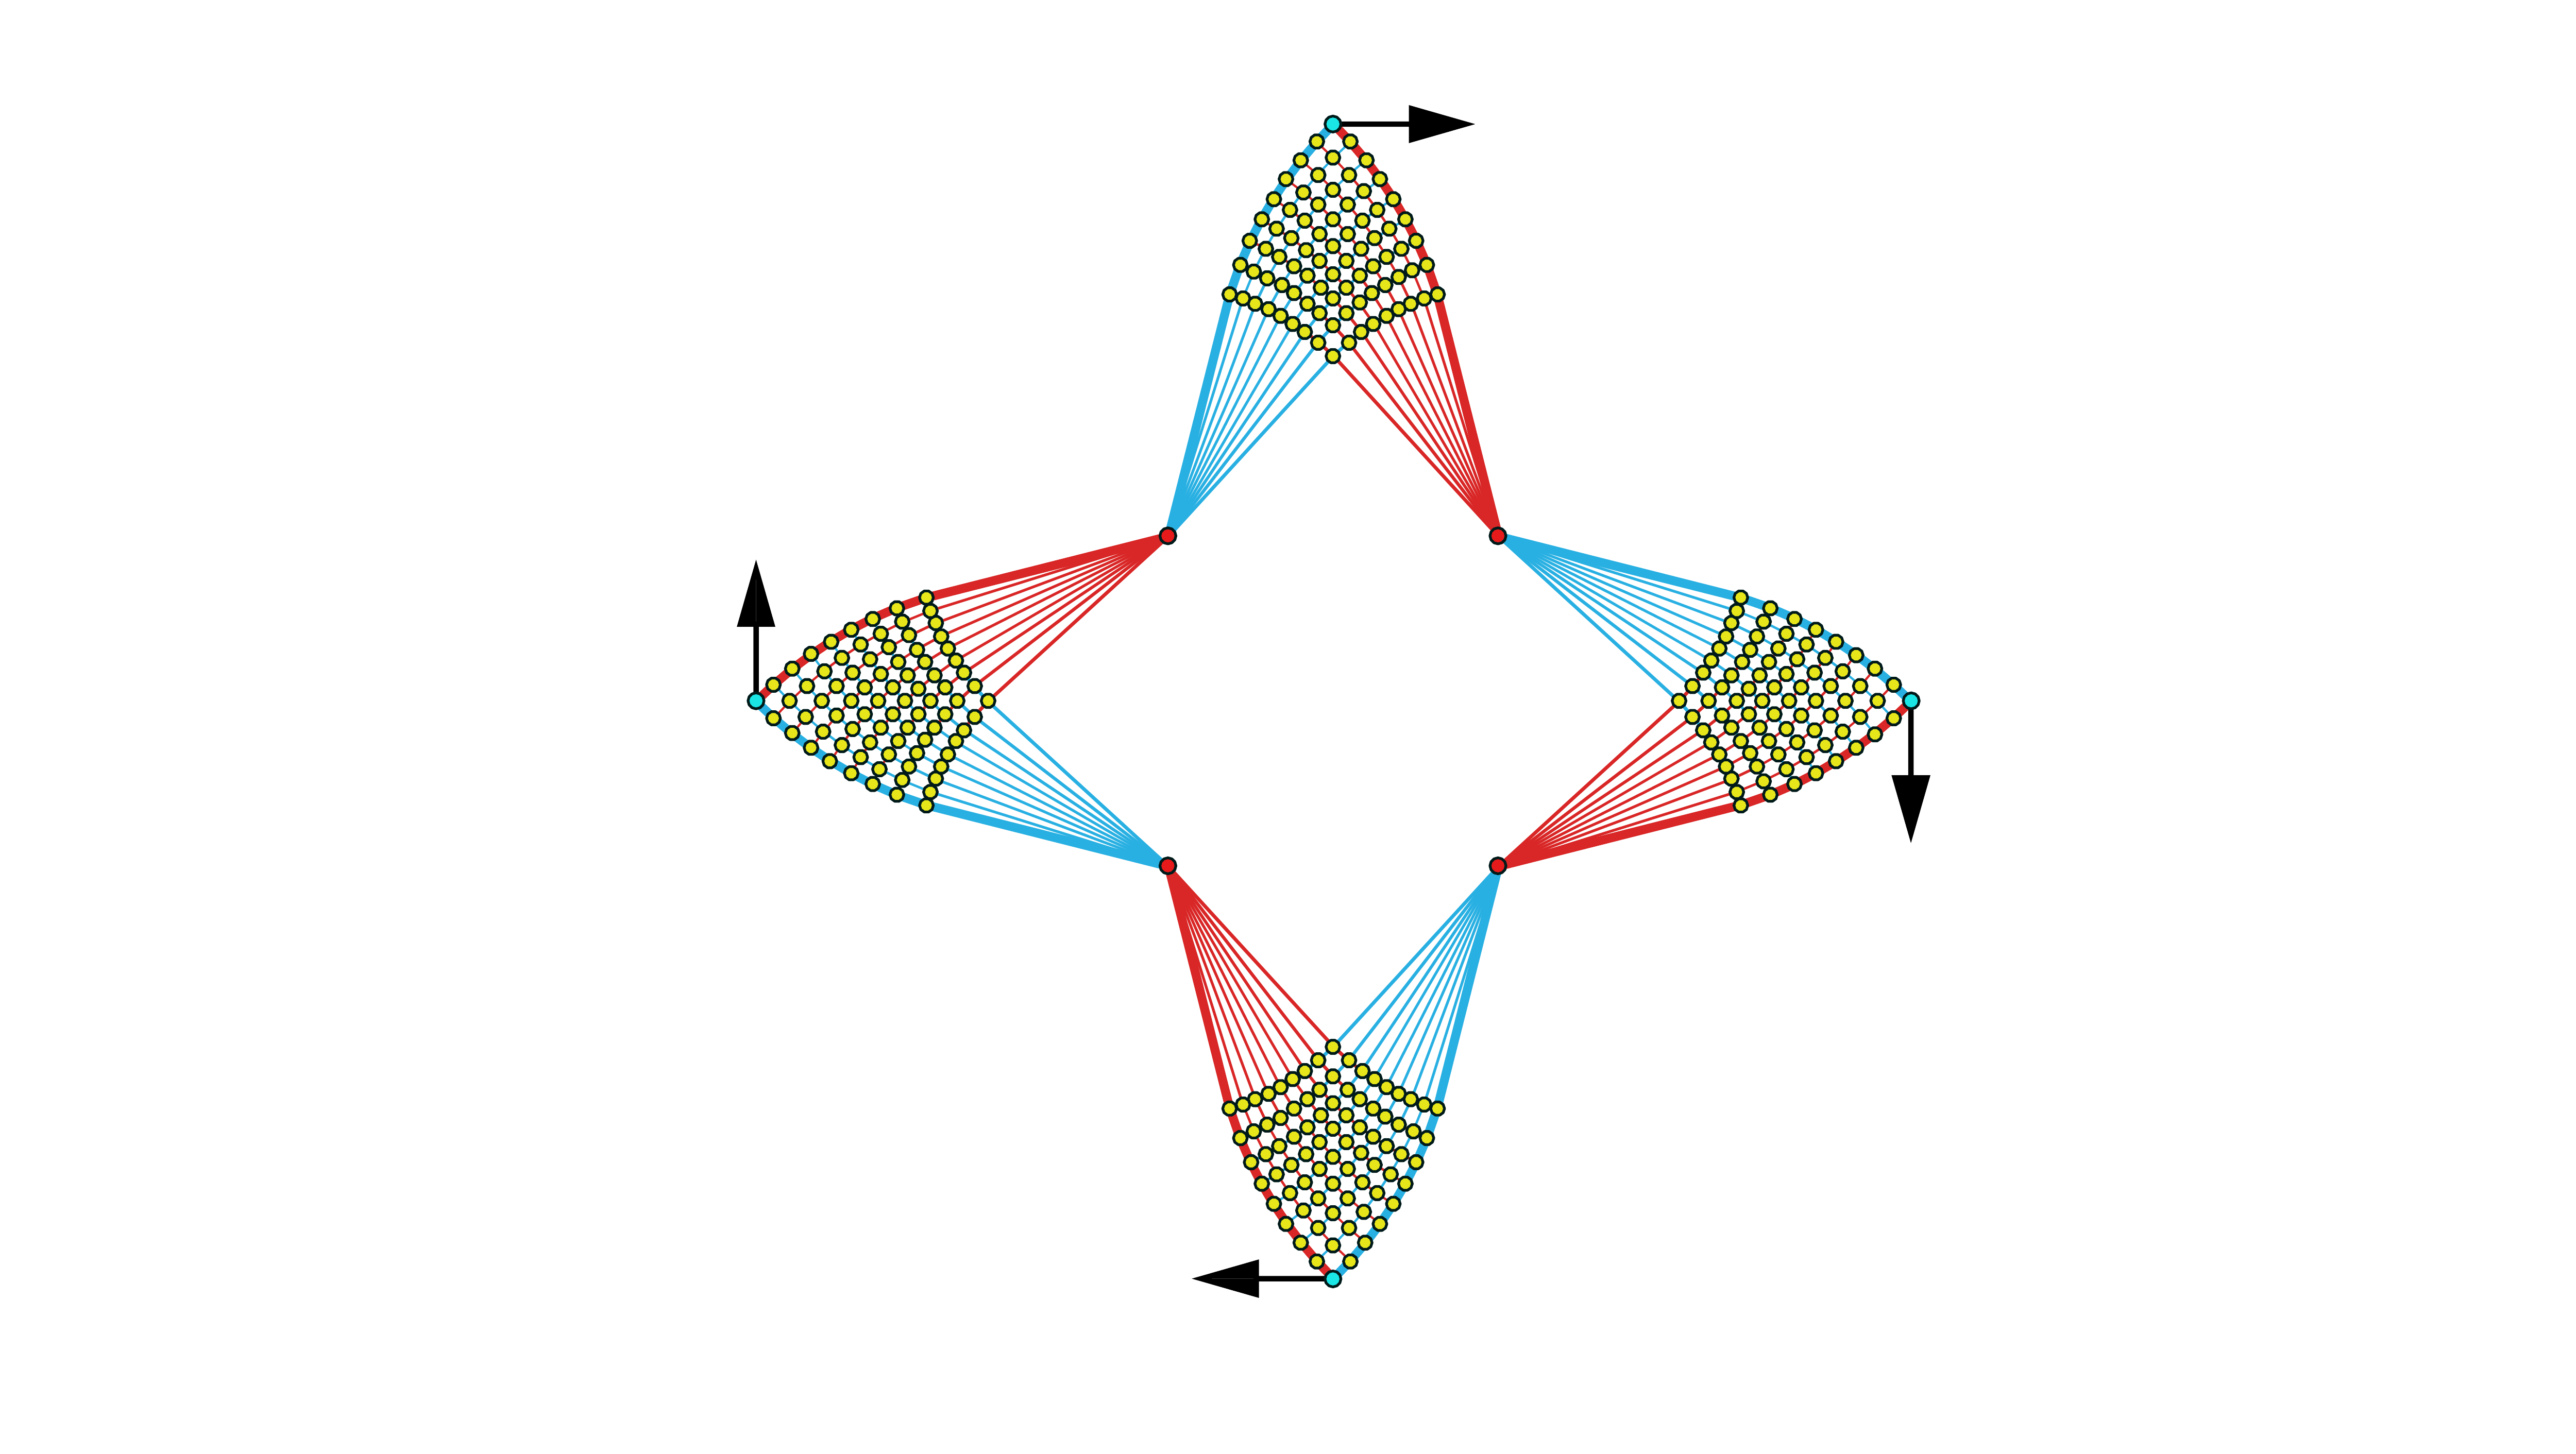}	
			\cput(50,2){\contour{white}{$(e)$}}	
		\end{overpic}
	}	
	\caption{
		\label{fig:2D008}
		Input functional specification has four supporting joints and four external forces applied outside of the bounding box of the supporting joints.}
\end{figure*}
\clearpage

\clearpage
\begin{figure*}[tb]\centering{
		\begin{overpic}			
			[width=1.3\columnwidth,trim={2cm 8cm 2cm 8cm},clip]{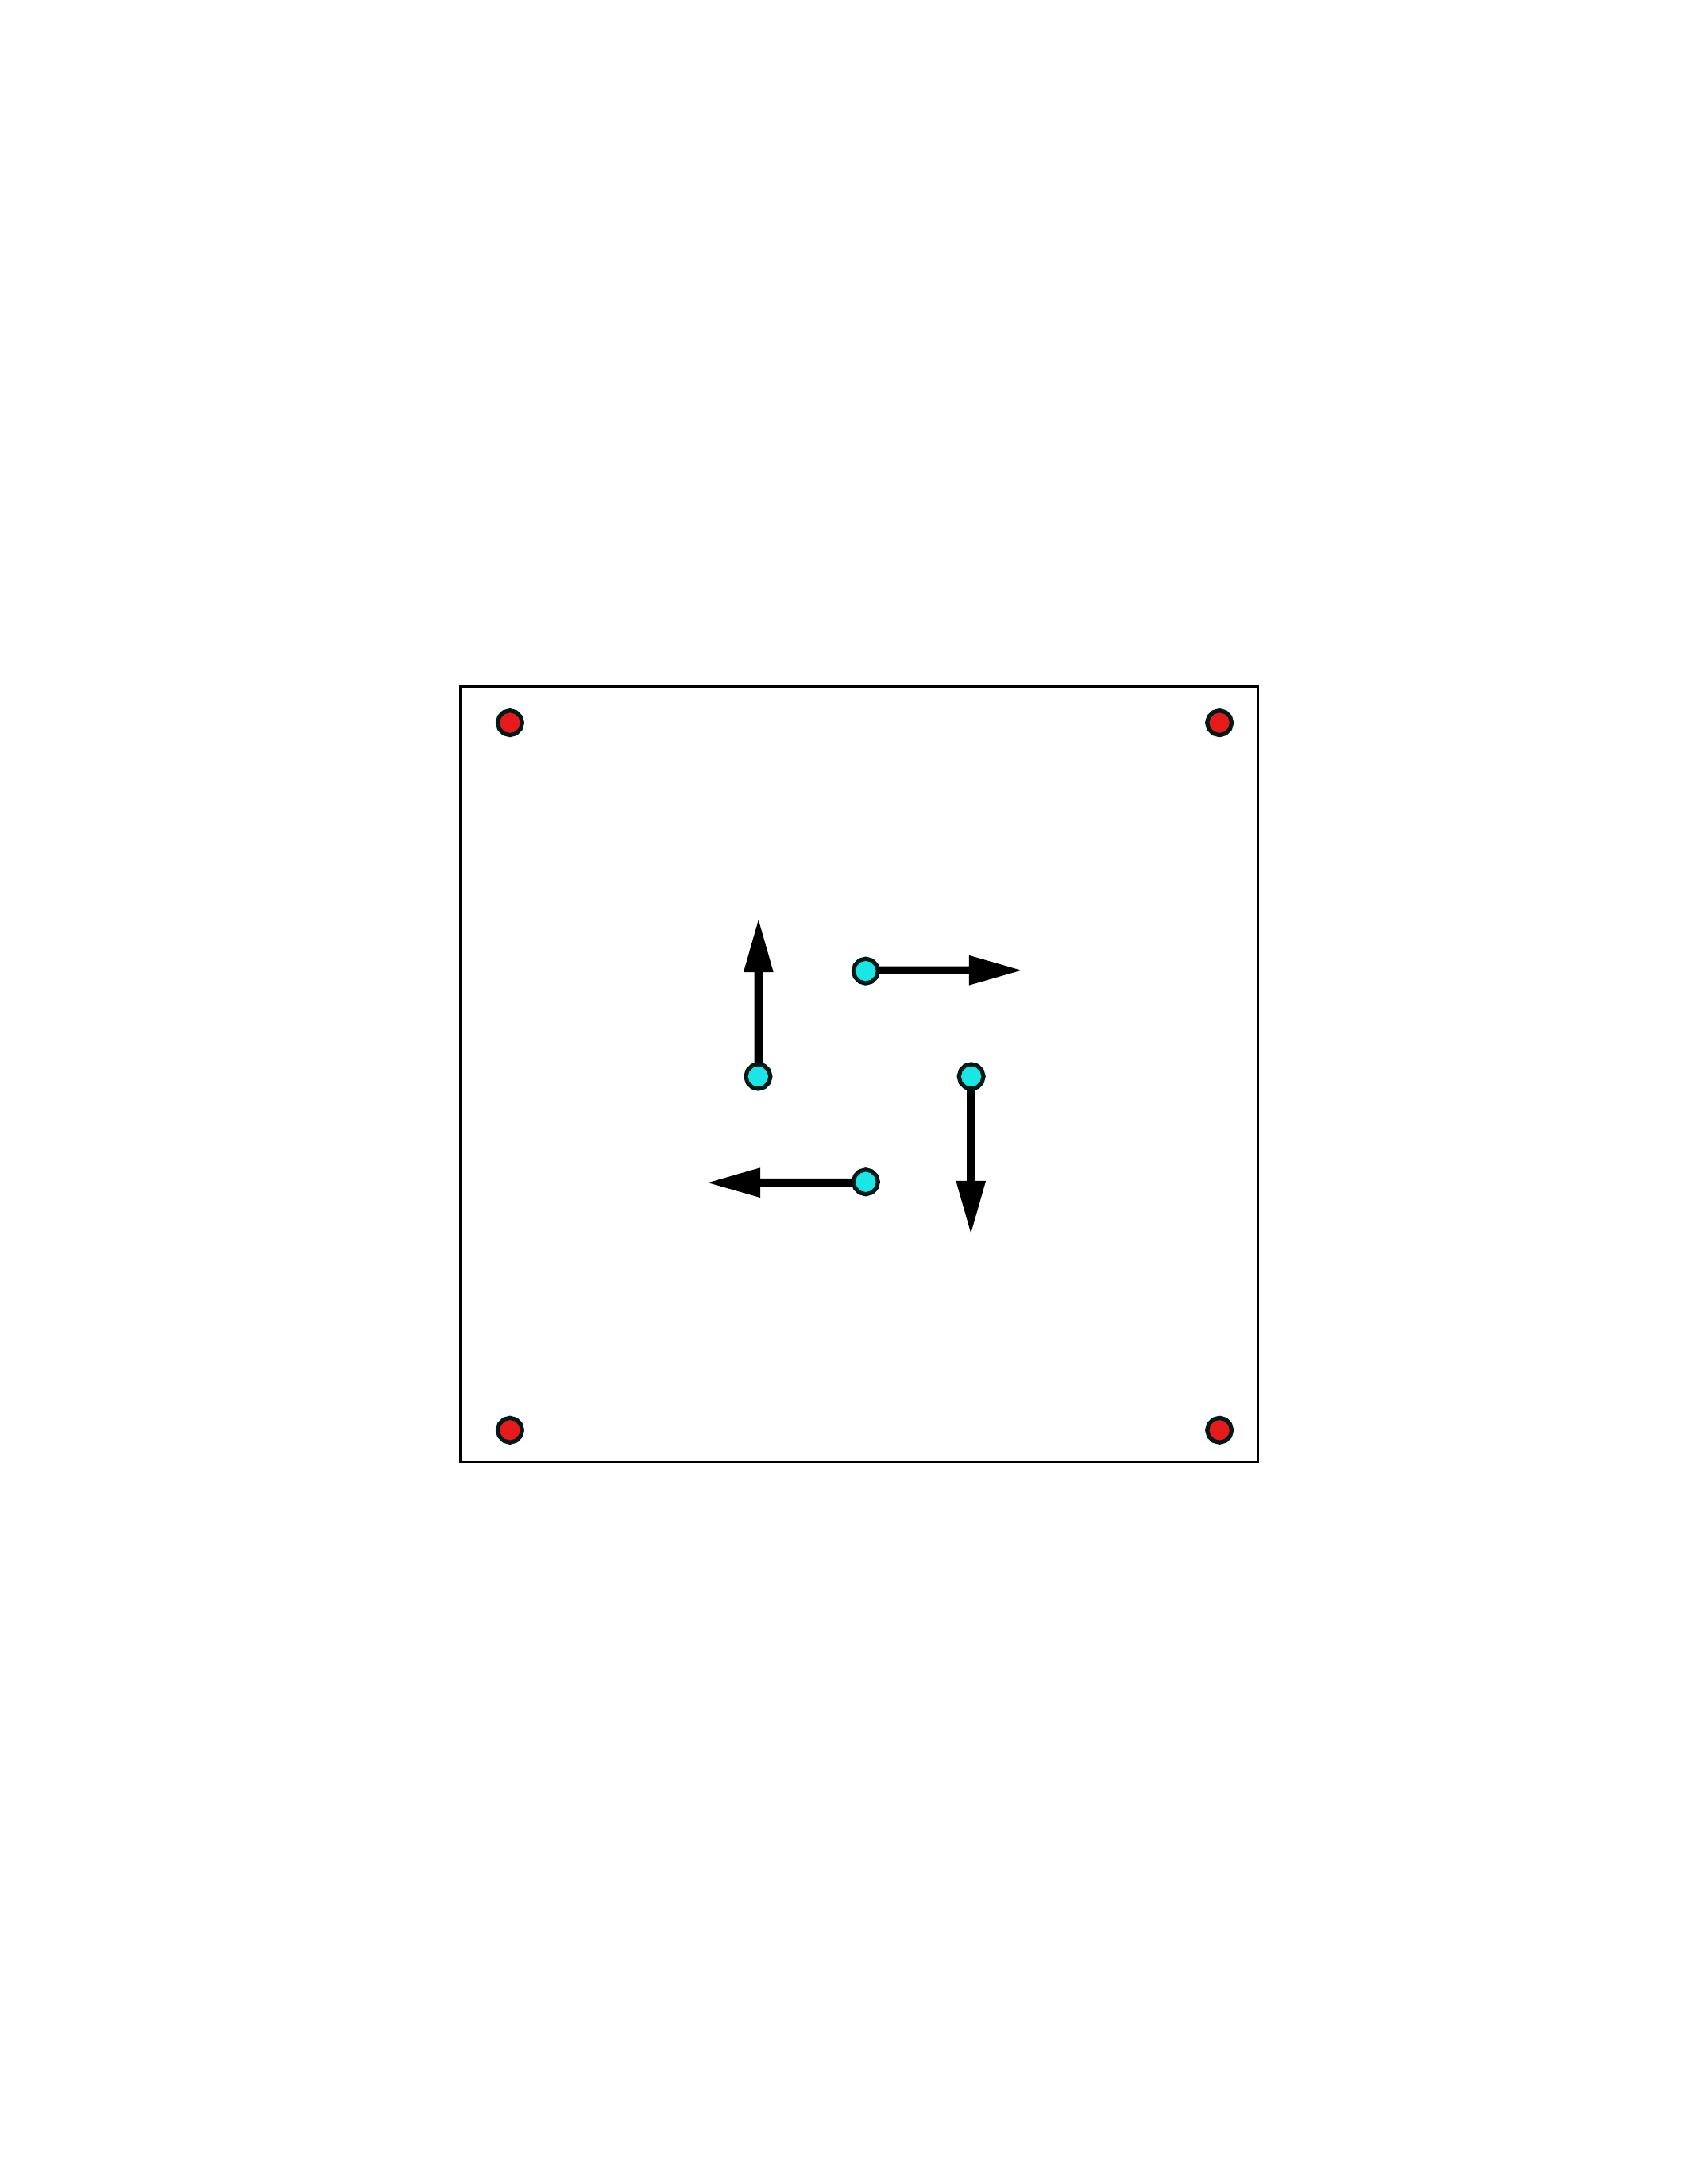}	
			\cput(50,2){\contour{white}{$(a)$}}		
		\end{overpic}
		\begin{overpic}			
			[width=0.8\columnwidth,trim={12cm 2cm 12cm 2cm},clip]{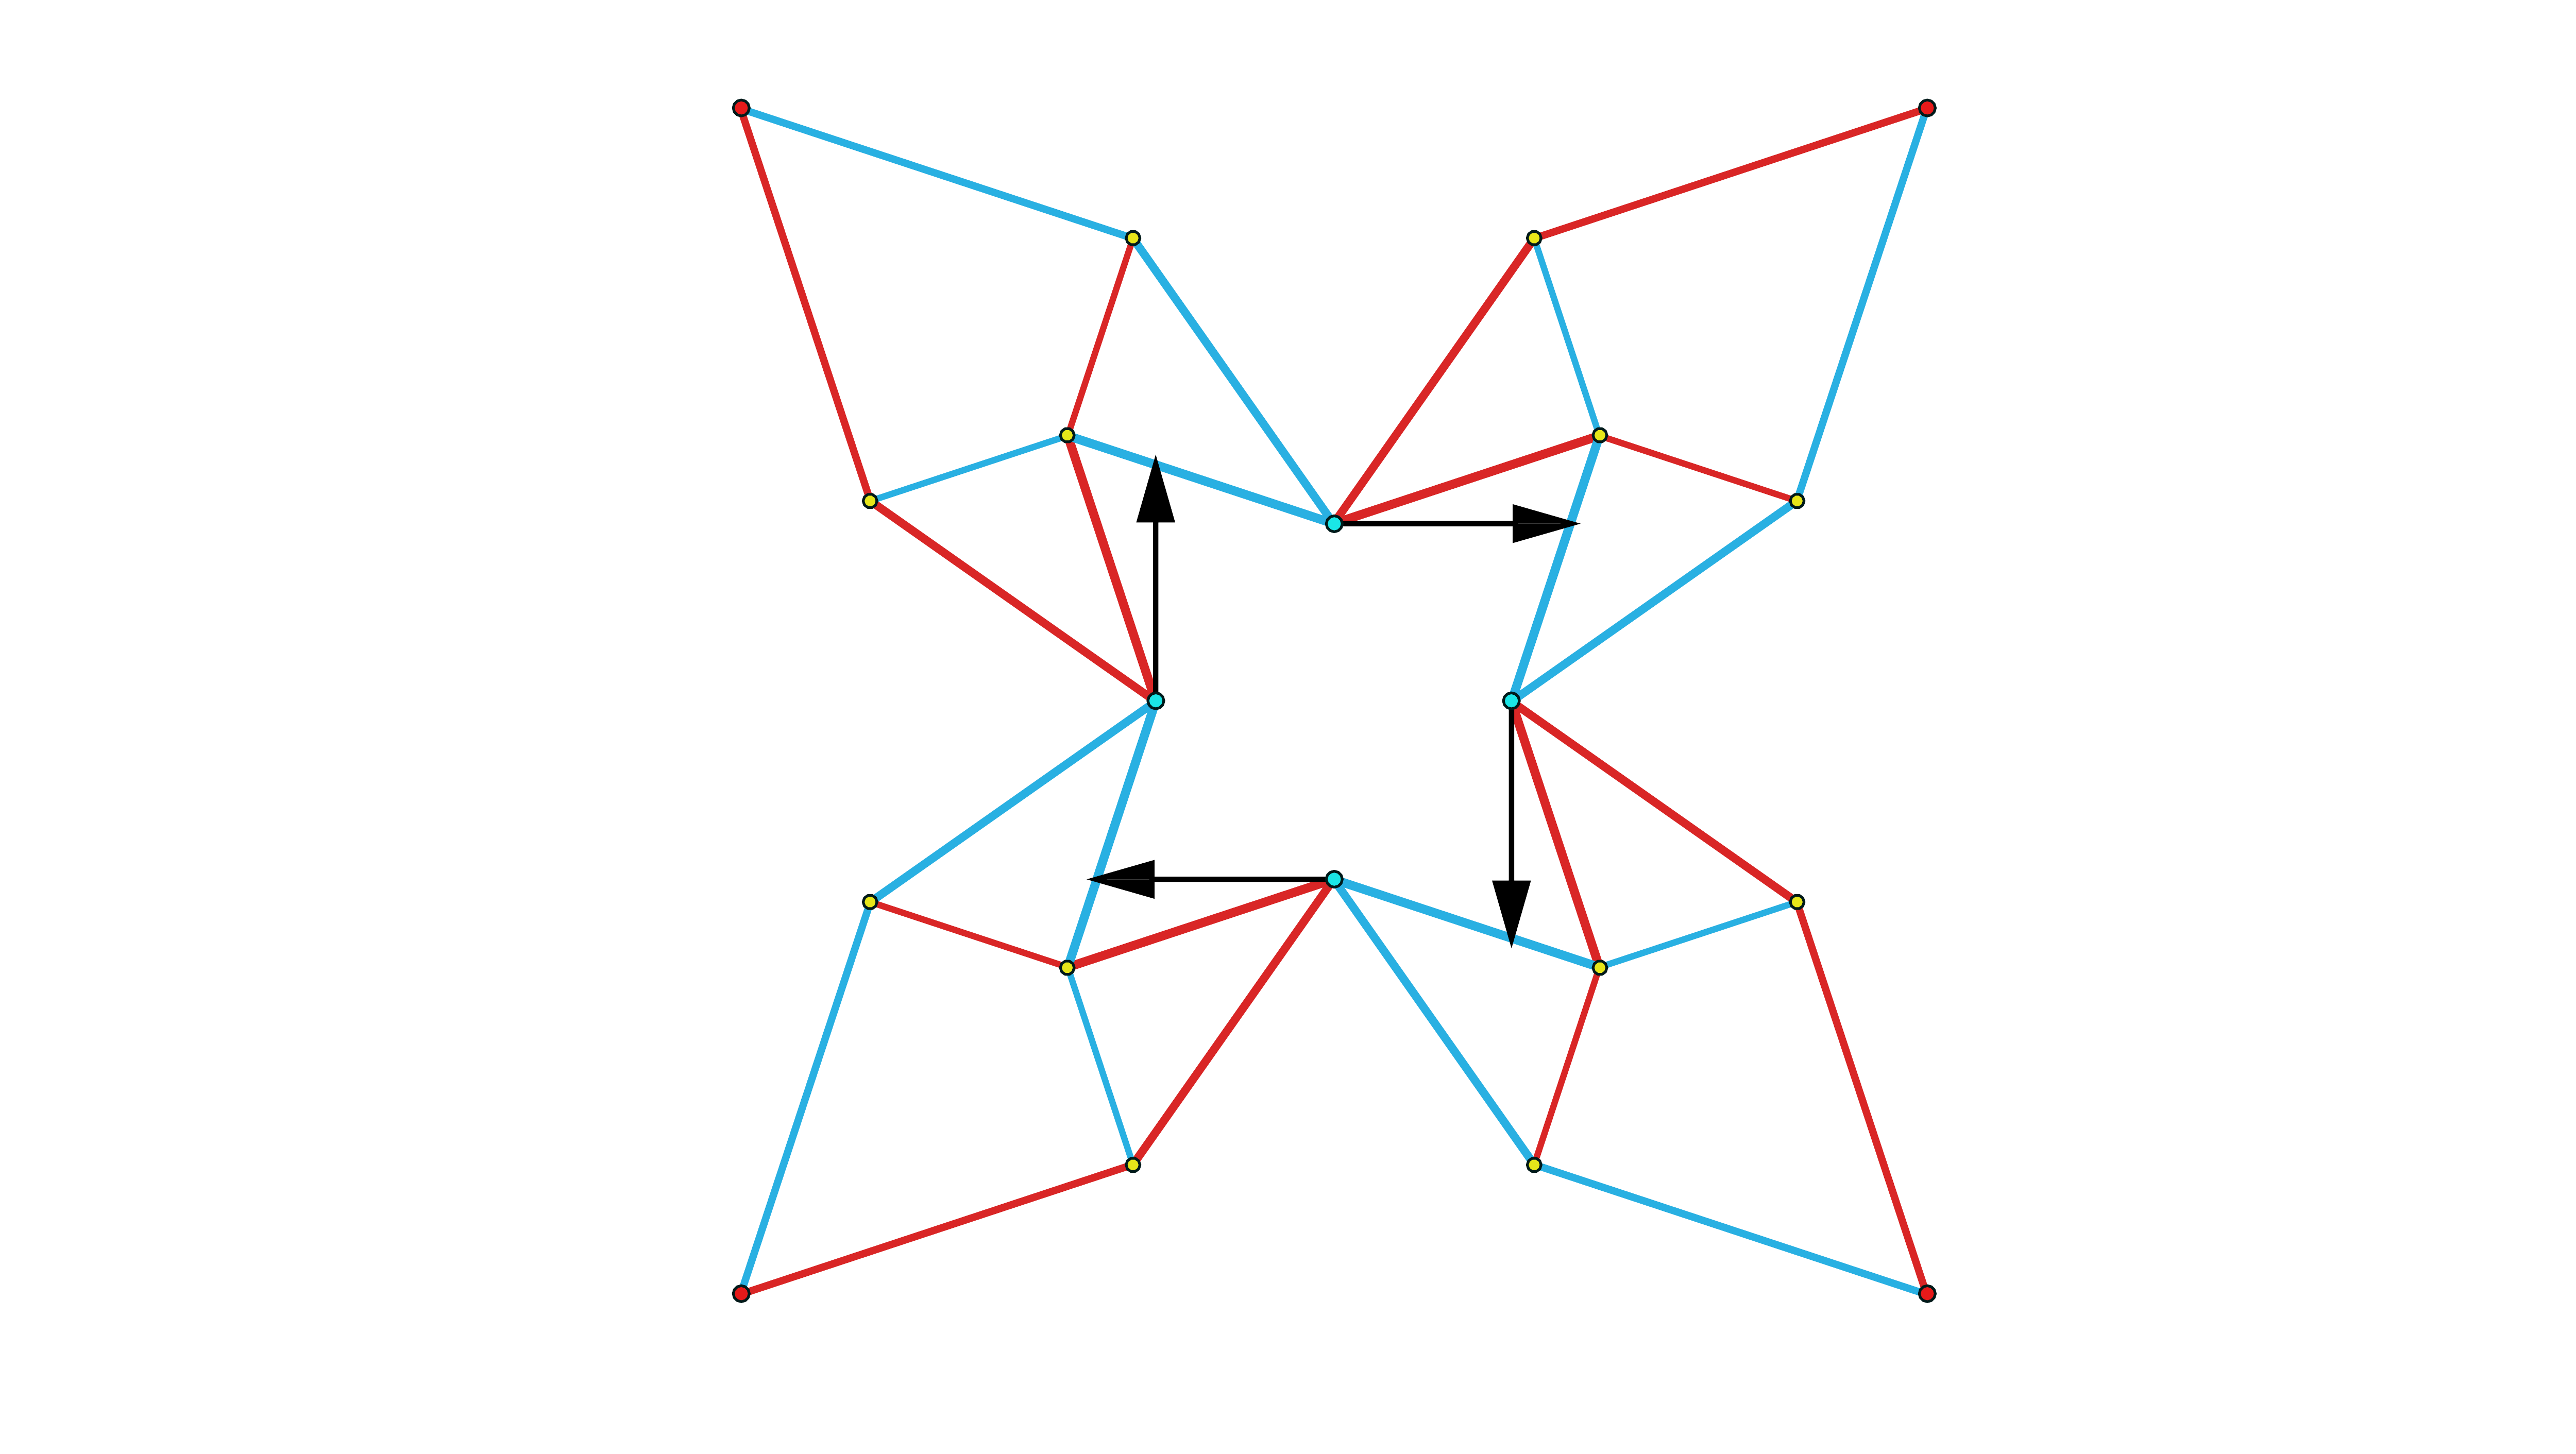}	
			\cput(50,2){\contour{white}{$(b)$}}	
		\end{overpic}
		\begin{overpic}			
			[width=0.8\columnwidth,trim={12cm 2cm 12cm 2cm},clip]{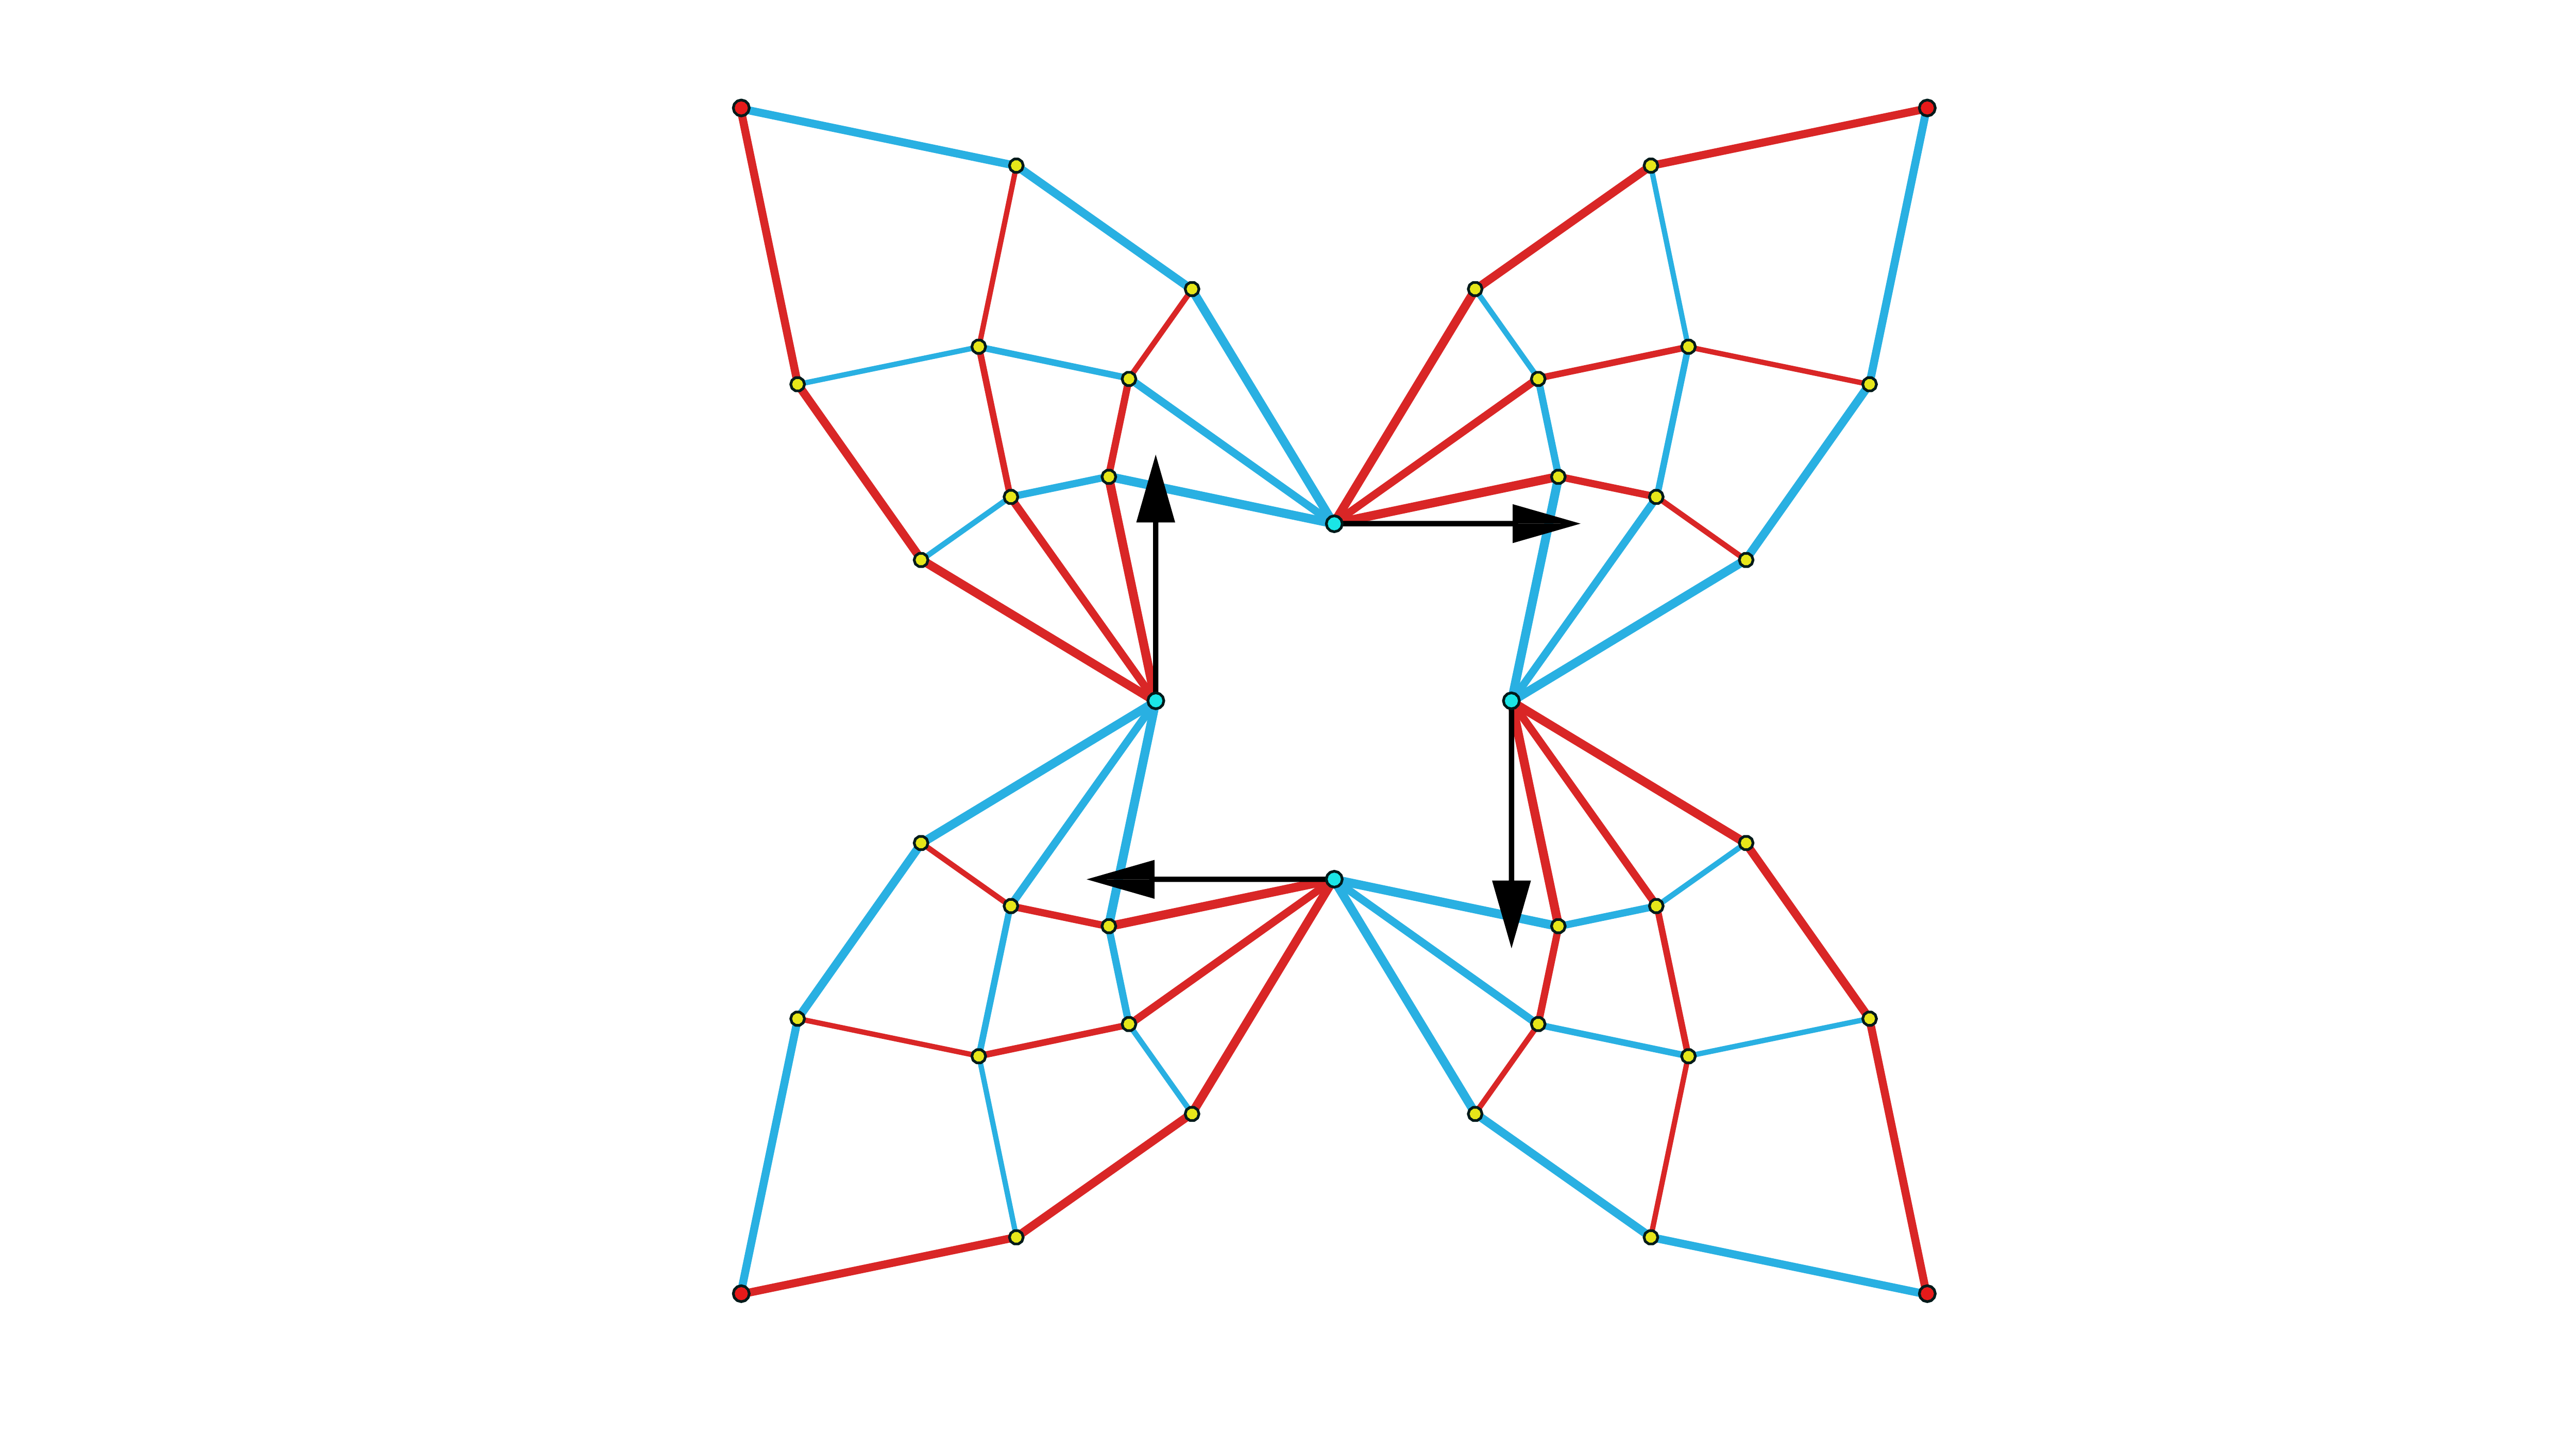}	
			\cput(50,2){\contour{white}{$(c)$}}	
		\end{overpic}
		\begin{overpic}			
			[width=0.8\columnwidth,trim={12cm 2cm 12cm 2cm},clip]{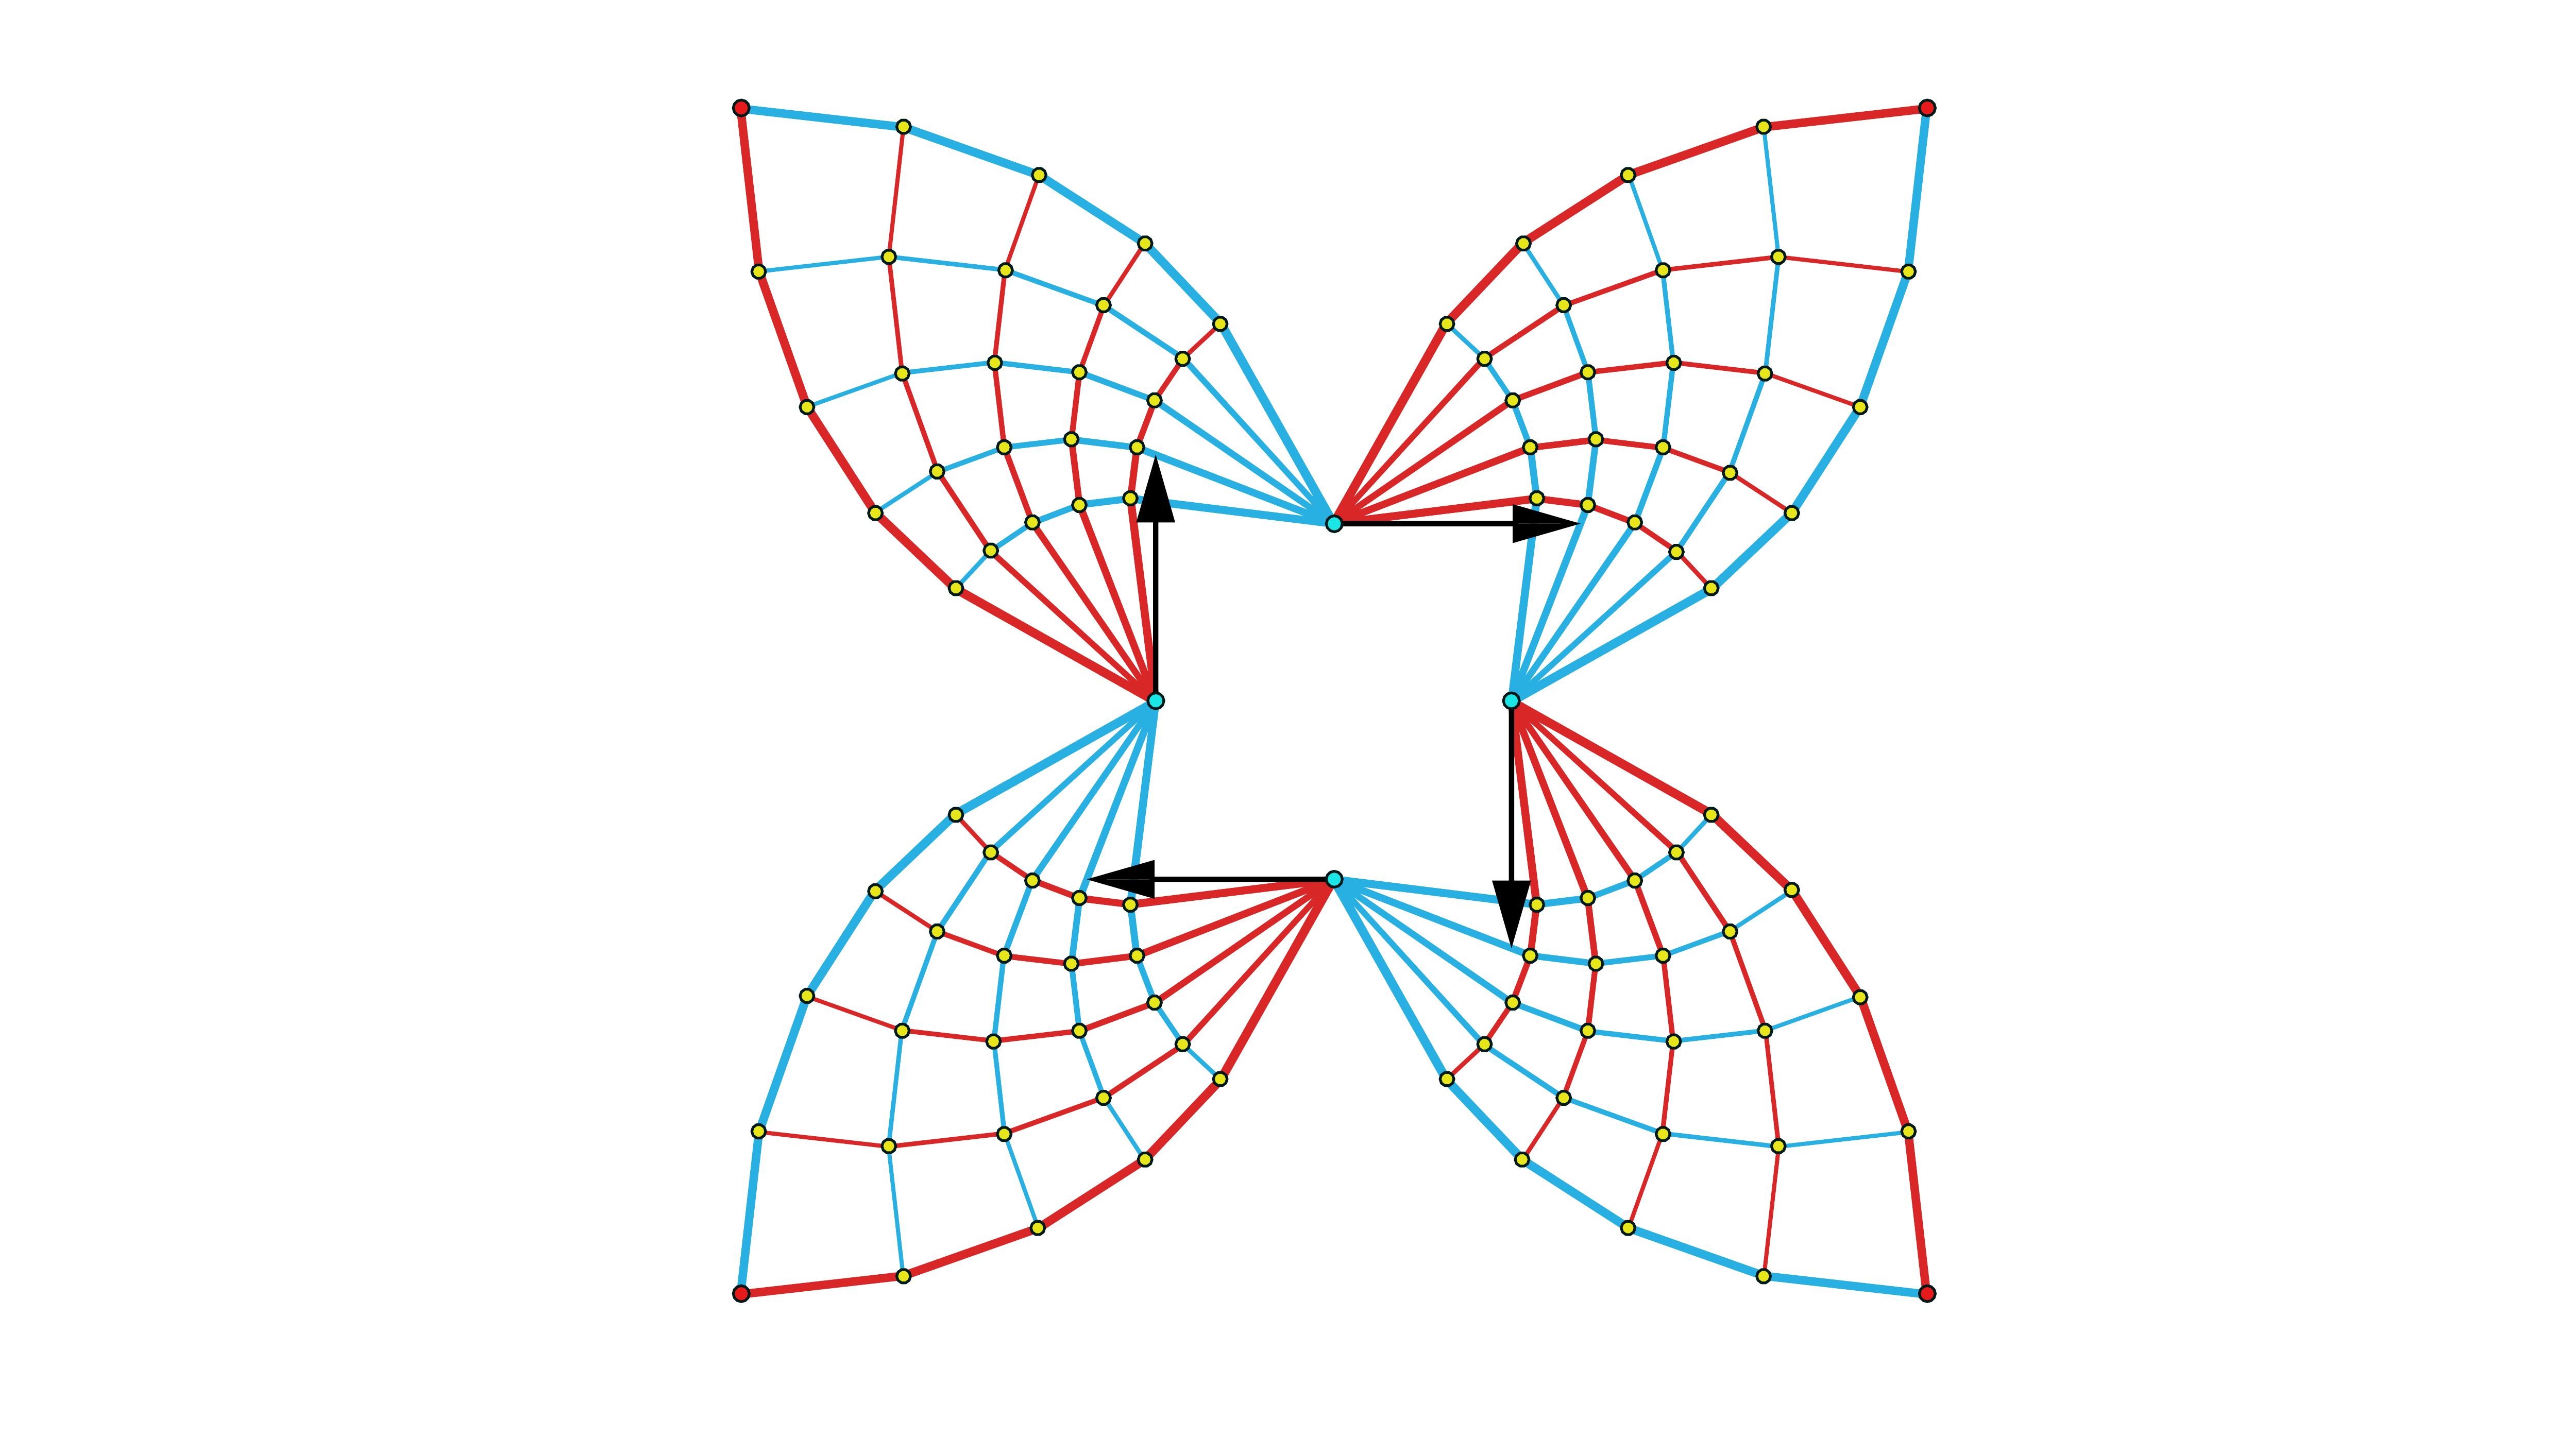}	
			\cput(50,2){\contour{white}{$(d)$}}	
		\end{overpic}
		\begin{overpic}			
			[width=0.8\columnwidth,trim={12cm 2cm 12cm 2cm},clip]{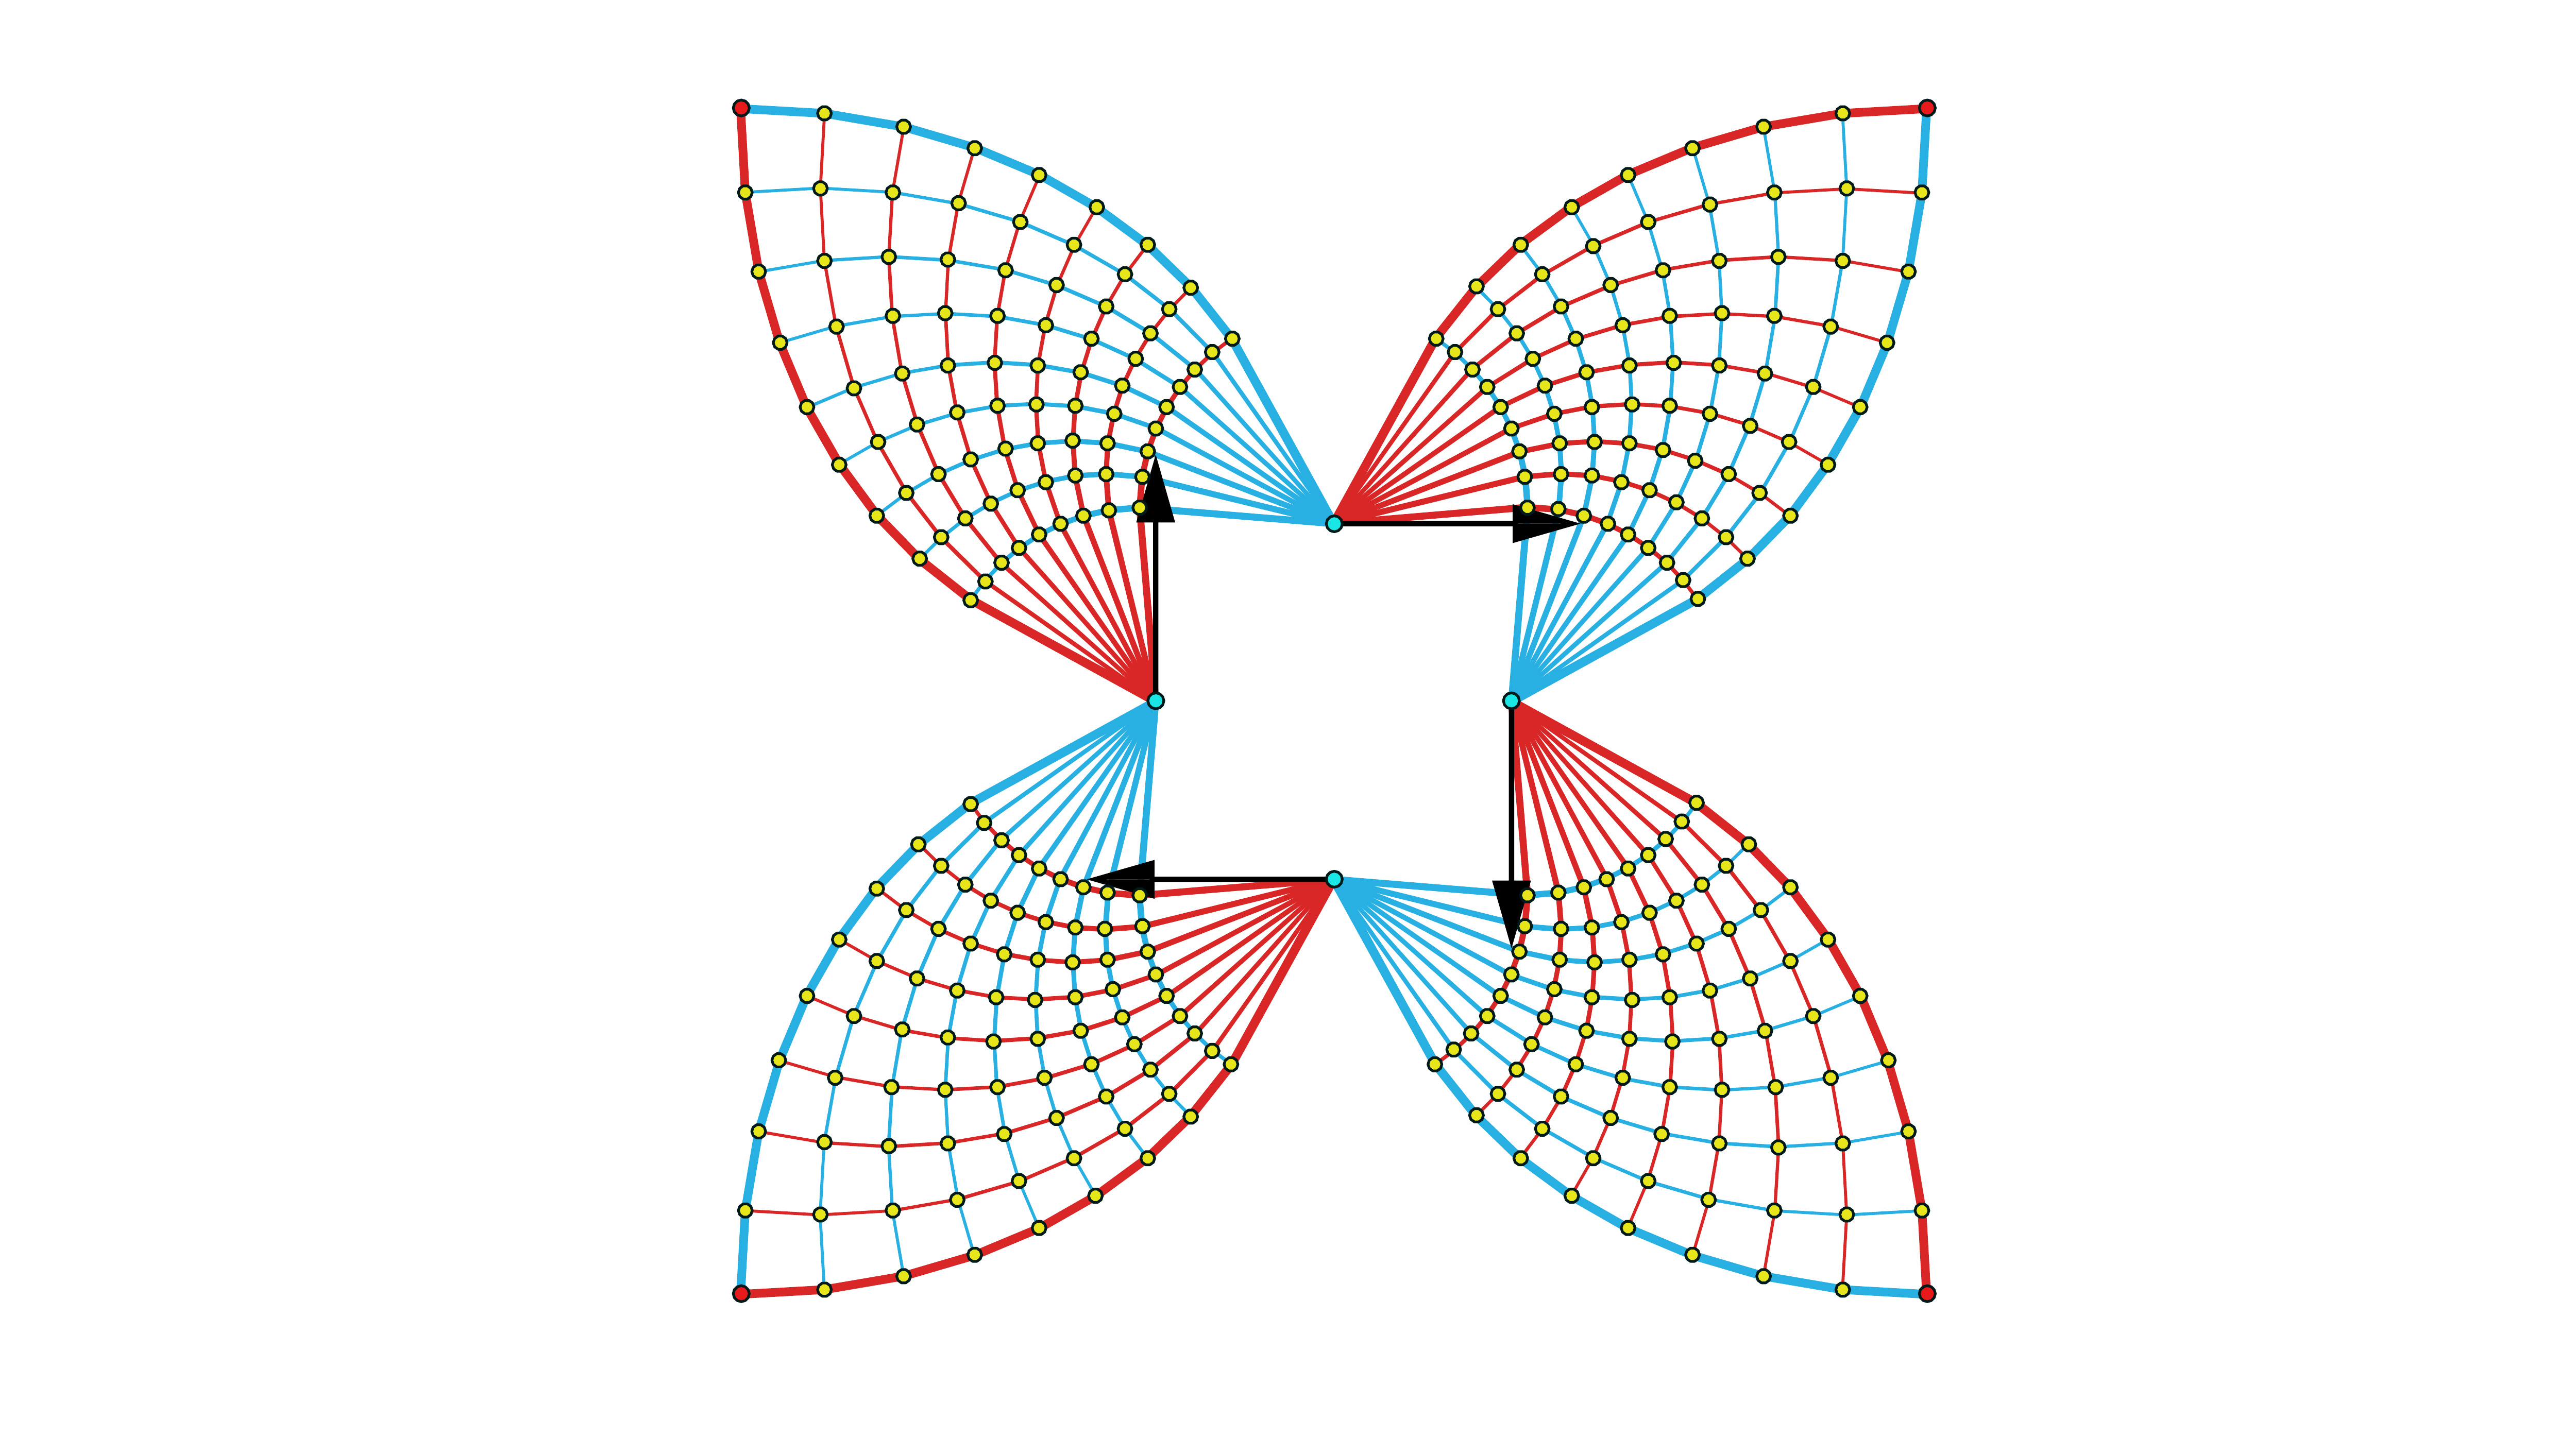}	
			\cput(50,2){\contour{white}{$(e)$}}	
		\end{overpic}
	}	
	\caption{
		\label{fig:2D009_1}
			Input functional specification has four supporting points and four external forces applied within the bounding box of the supporting points.}
\end{figure*}
\clearpage
\clearpage
\begin{figure*}[tb]\centering{
		\begin{overpic}			
			[width=1.3\columnwidth,trim={2cm 8cm 2cm 8cm},clip]{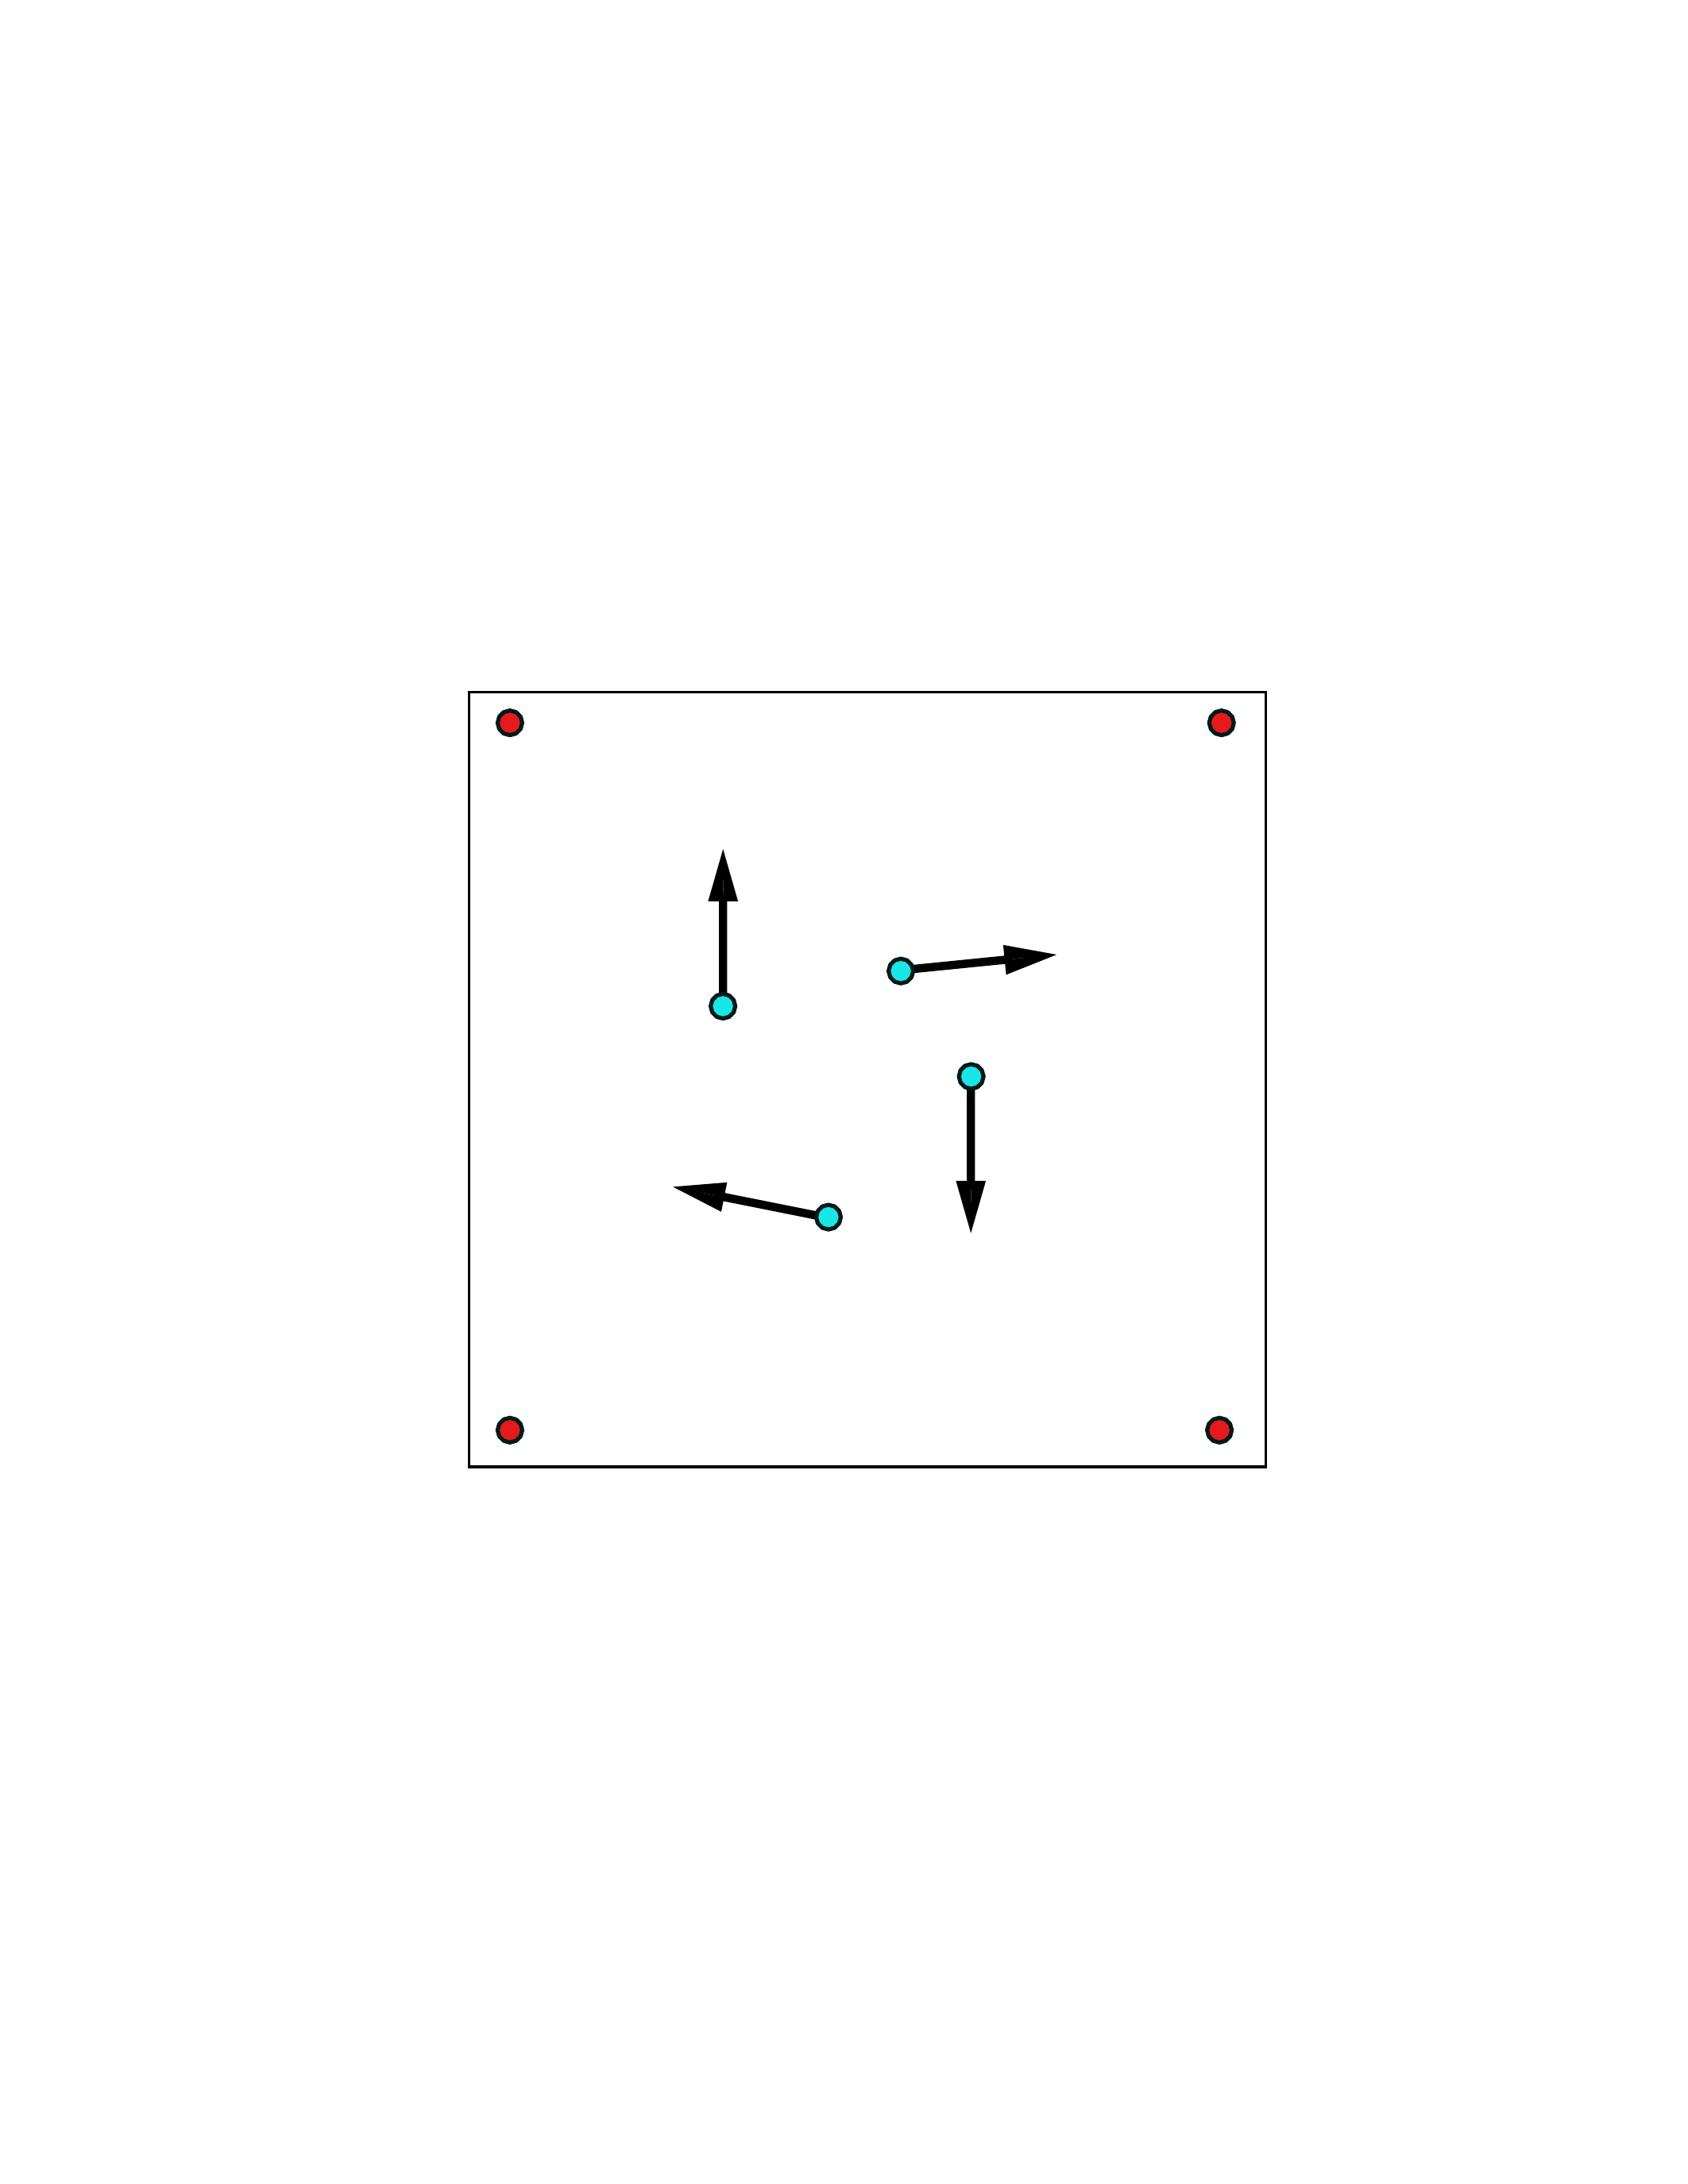}	
			\cput(50,2){\contour{white}{$(a)$}}		
		\end{overpic}
		\begin{overpic}			
			[width=0.8\columnwidth,trim={12cm 2cm 12cm 2cm},clip]{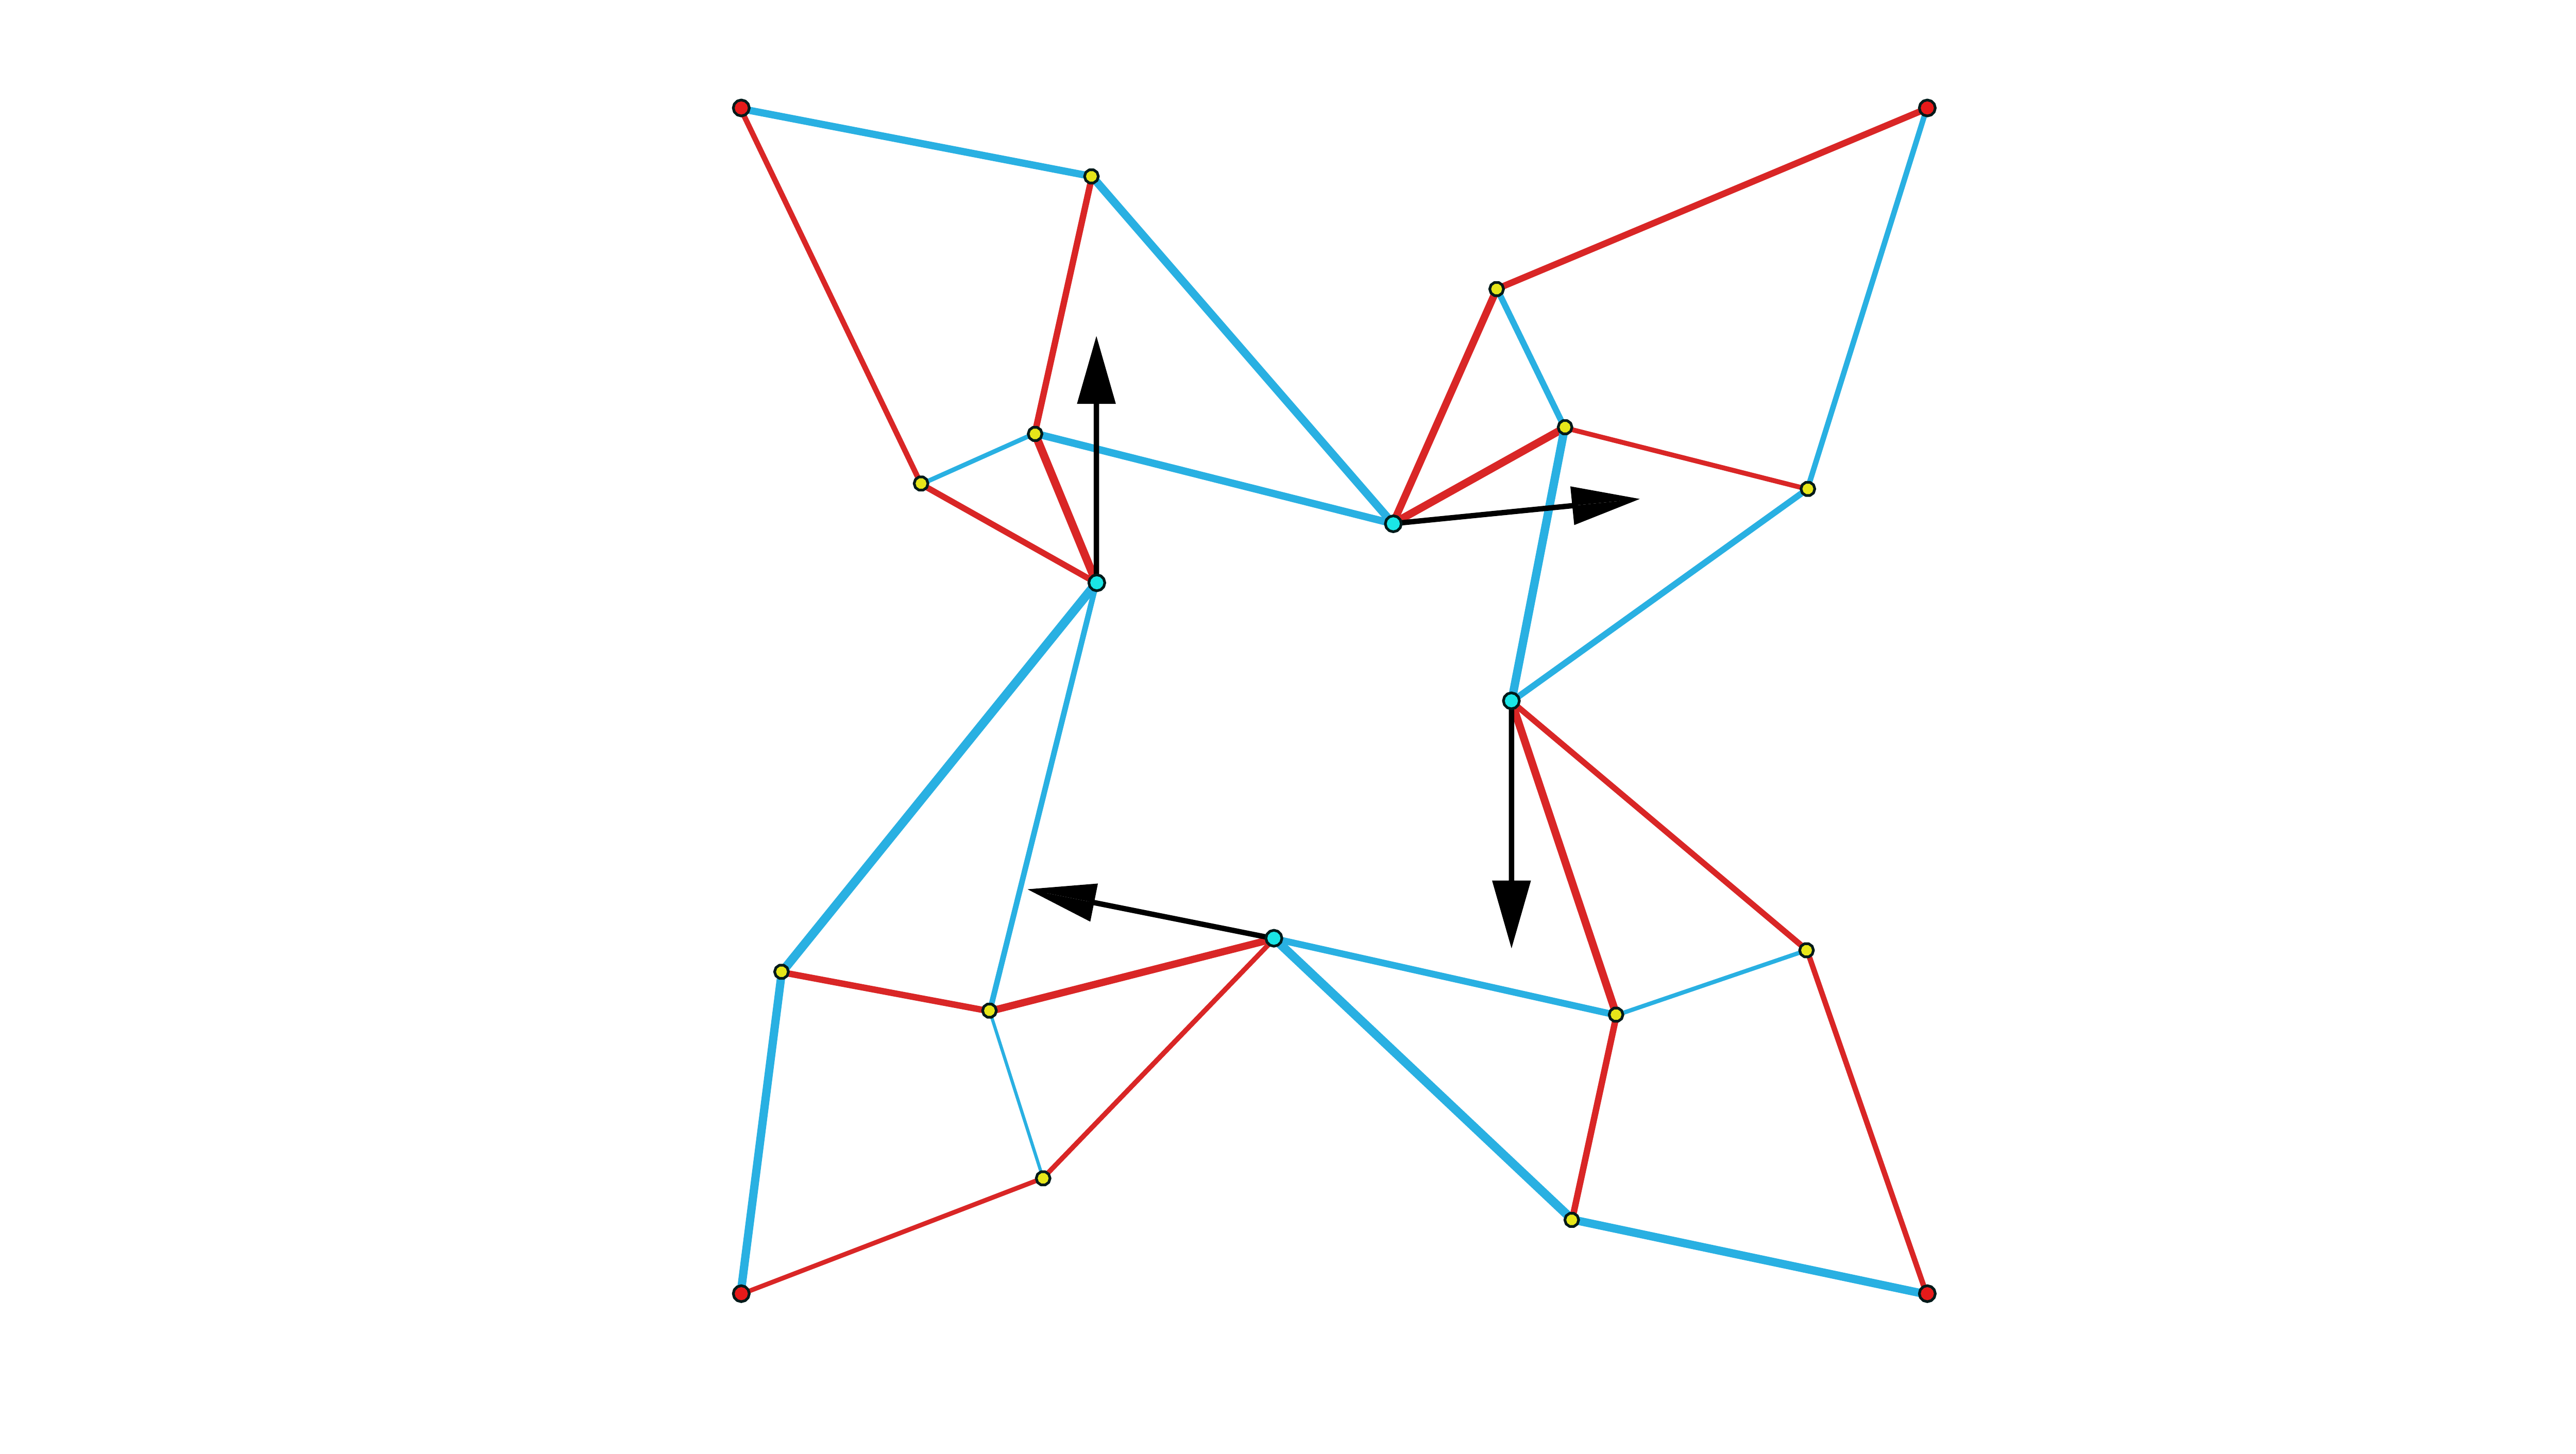}	
			\cput(50,2){\contour{white}{$(b)$}}	
		\end{overpic}
		\begin{overpic}			
			[width=0.8\columnwidth,trim={12cm 2cm 12cm 2cm},clip]{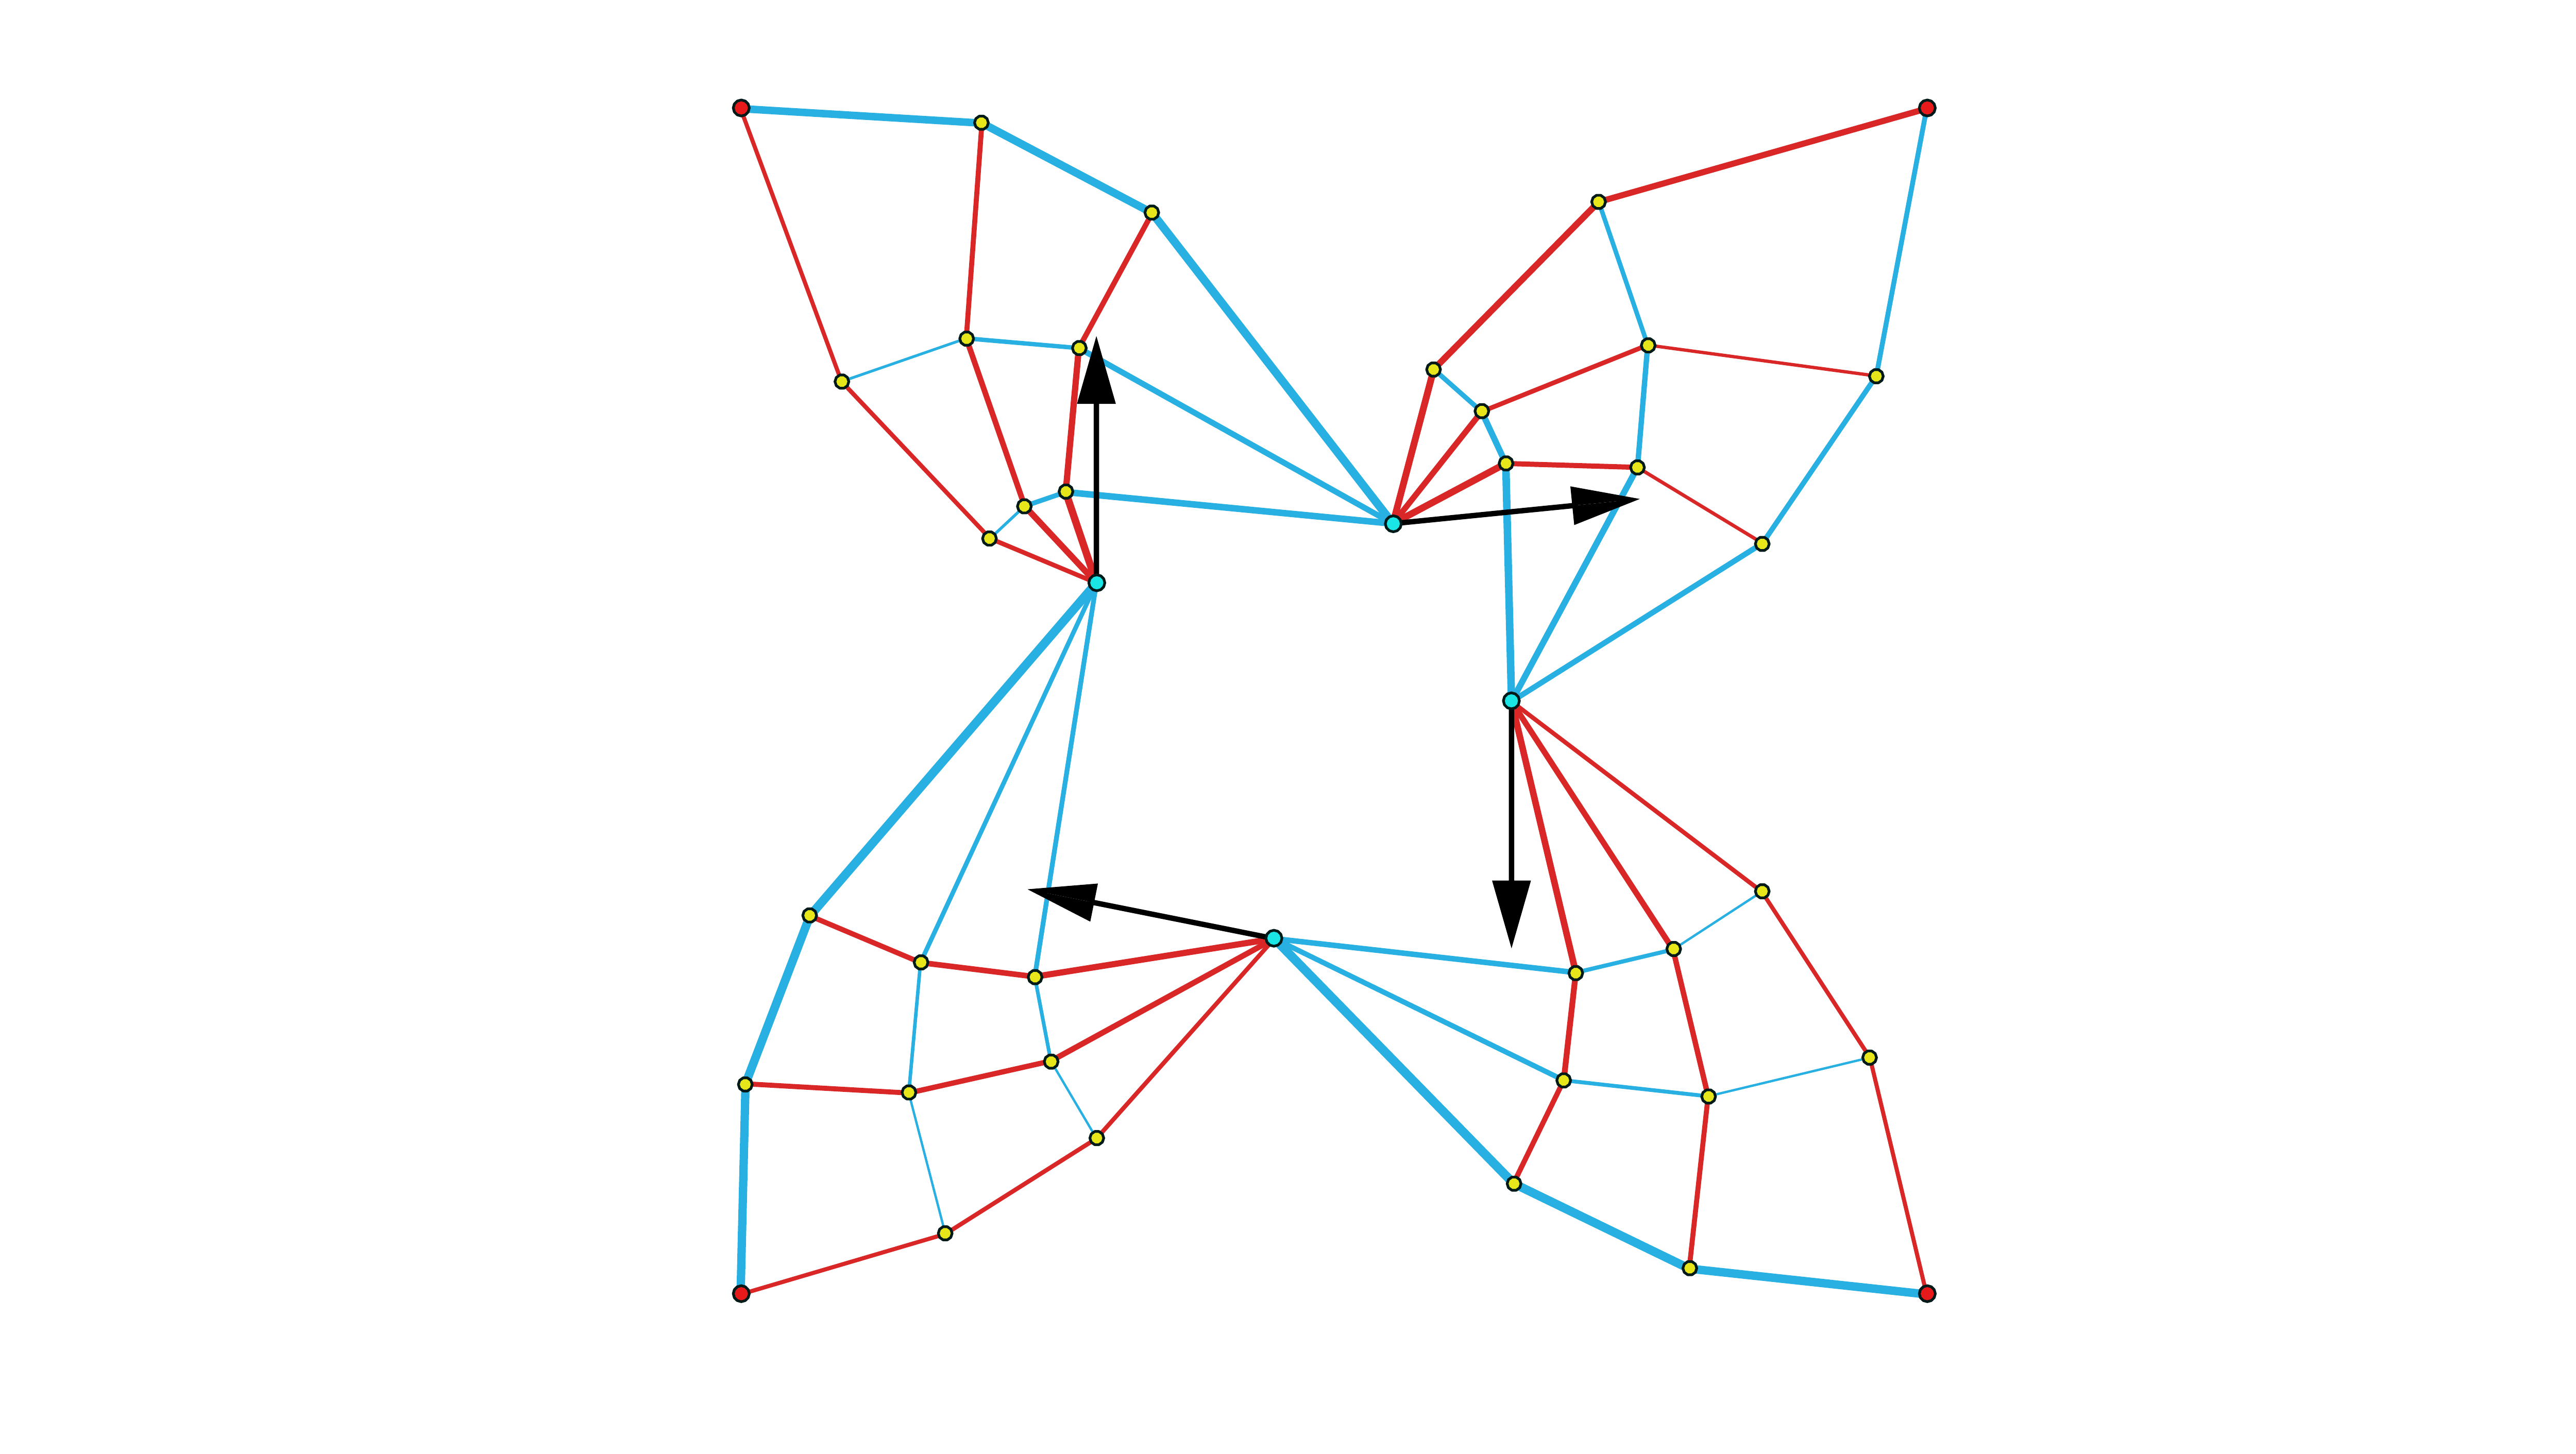}	
			\cput(50,2){\contour{white}{$(c)$}}	
		\end{overpic}
		\begin{overpic}			
			[width=0.8\columnwidth,trim={12cm 2cm 12cm 2cm},clip]{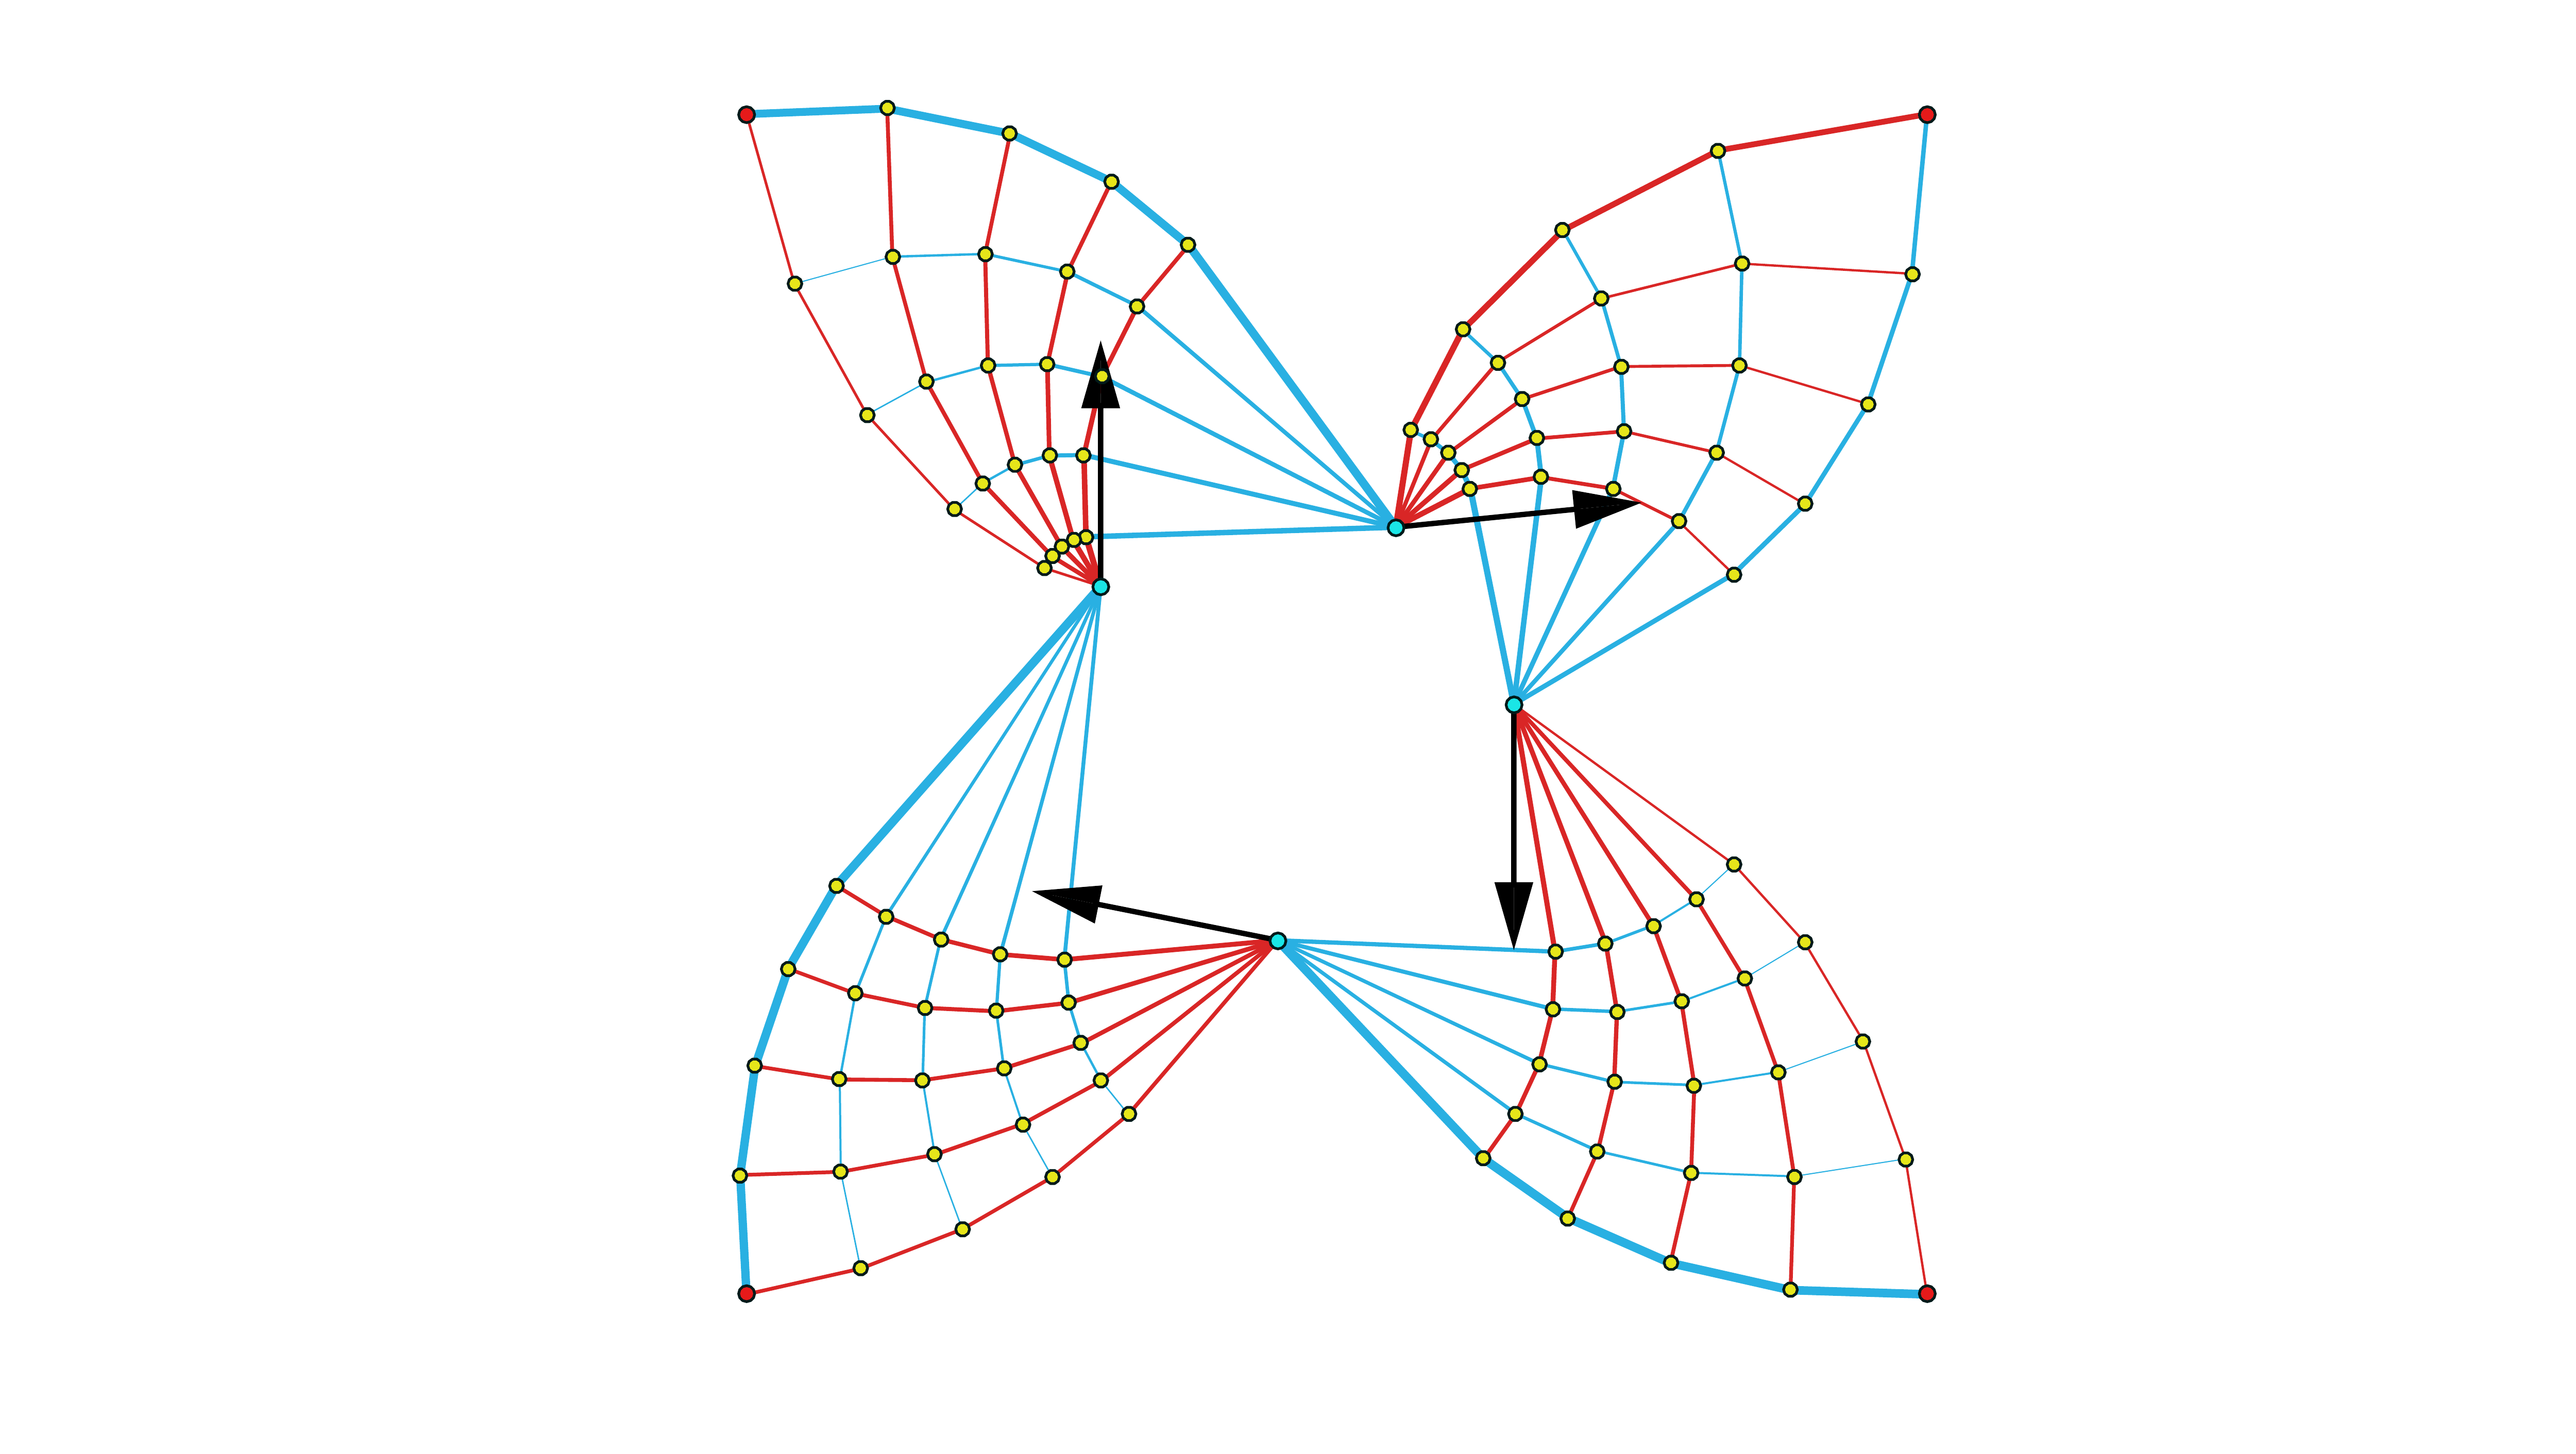}	
			\cput(50,2){\contour{white}{$(d)$}}	
		\end{overpic}
		\begin{overpic}			
			[width=0.8\columnwidth,trim={12cm 2cm 12cm 2cm},clip]{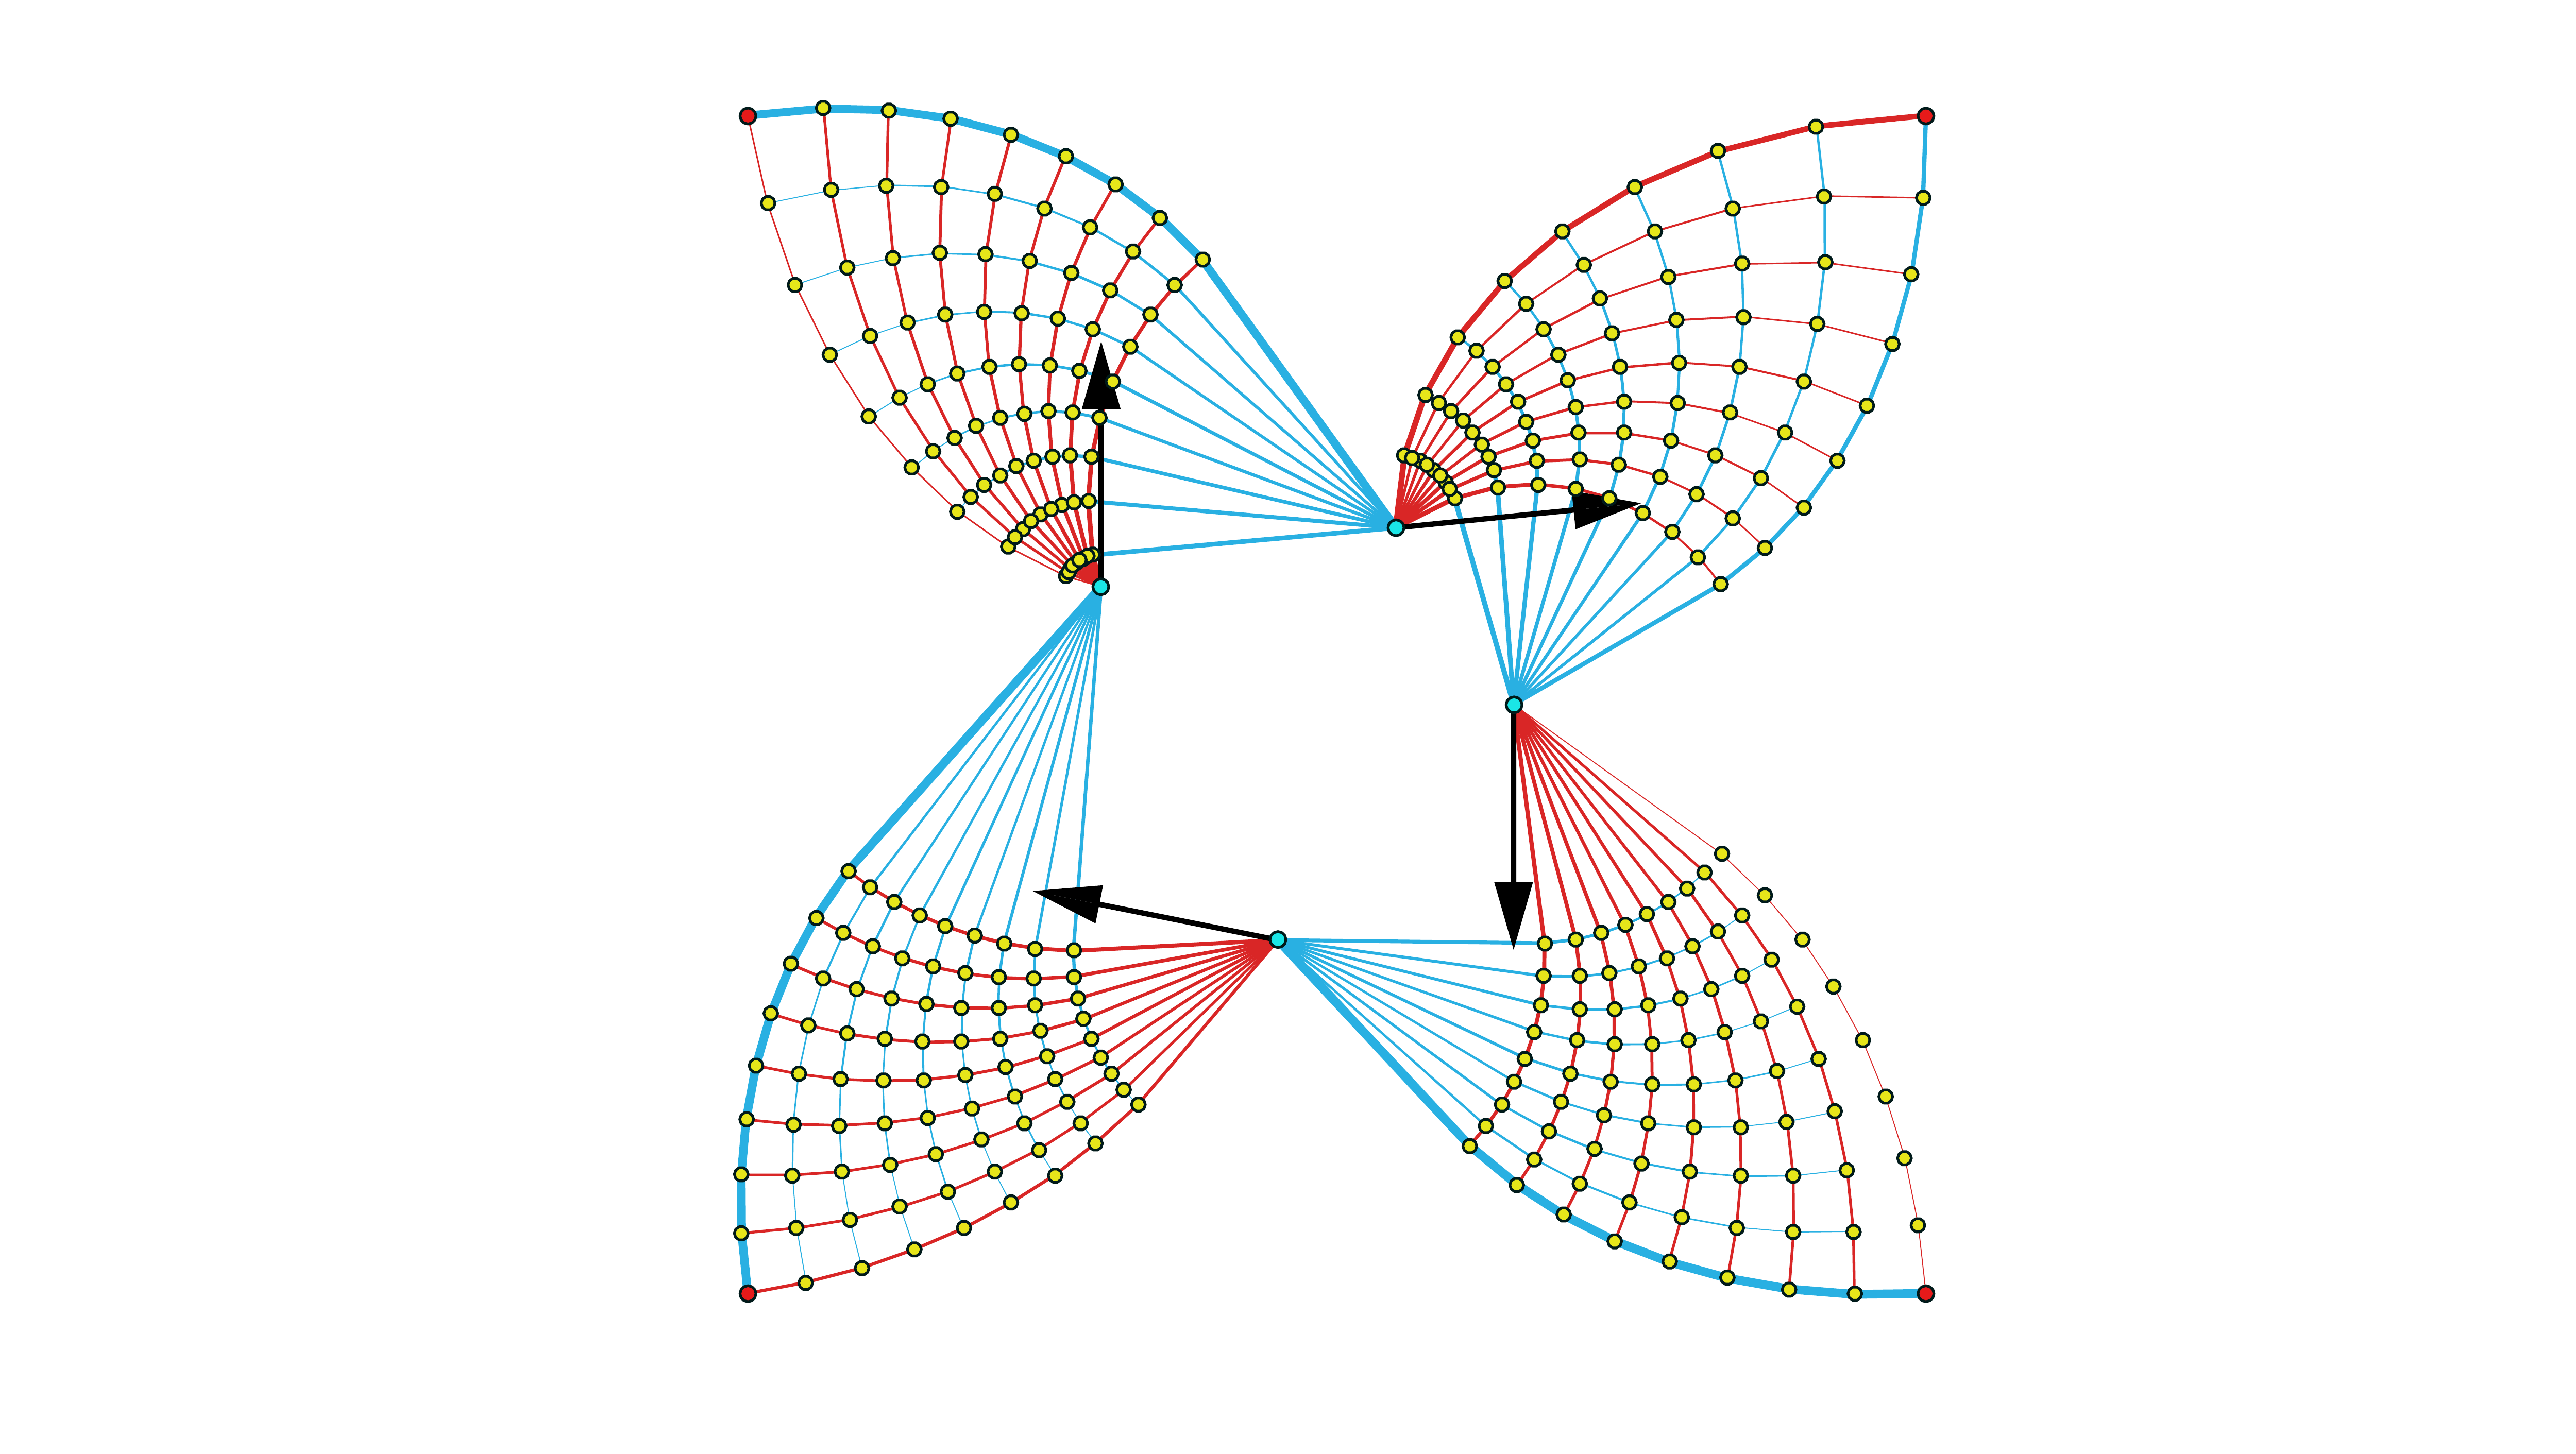}	
			\cput(50,2){\contour{white}{$(e)$}}	
		\end{overpic}
	}	
	\caption{
		\label{fig:2D009_4}
	Input functional specification has four supporting points and four external forces applied within the bounding box of the supporting points.}
\end{figure*}
\clearpage

%\clearpage
%\begin{figure*}[tb]\centering{
%		\begin{overpic}			
%			[width=1\columnwidth,trim={4cm 10cm 4cm 10cm},clip]{figure/2D005_0}	
%			\cput(50,2){\contour{white}{$(a)$}}		
%		\end{overpic}
%			\begin{overpic}			
%				[width=1\columnwidth,trim={4cm 10cm 4cm 10cm},clip]{figure/2D005_1_0}	
%				\cput(50,2){\contour{white}{$(a)$}}		
%			\end{overpic}
%		\begin{overpic}			
%			[width=1\columnwidth,trim={4cm 10cm 4cm 10cm},clip]{figure/2D005_1}	
%			\cput(50,2){\contour{white}{$(b)$}}	
%		\end{overpic}
%		\begin{overpic}			
%			[width=1\columnwidth,trim={4cm 10cm 4cm 10cm},clip]{figure/2D005_1_1}	
%			\cput(50,2){\contour{white}{$(c)$}}	
%		\end{overpic}
%		\begin{overpic}			
%			[width=1\columnwidth,trim={4cm 10cm 4cm 10cm},clip]{figure/2D005_2}	
%			\cput(50,2){\contour{white}{$(d)$}}	
%		\end{overpic}
%		\begin{overpic}			
%			[width=1\columnwidth,trim={4cm 10cm 4cm 10cm},clip]{figure/2D005_1_2}	
%			\cput(50,2){\contour{white}{$(e)$}}	
%		\end{overpic}
%				\begin{overpic}			
%					[width=1\columnwidth,trim={4cm 10cm 4cm 10cm},clip]{figure/2D005_3}	
%					\cput(50,2){\contour{white}{$(d)$}}	
%				\end{overpic}
%				\begin{overpic}			
%					[width=1\columnwidth,trim={4cm 10cm 4cm 10cm},clip]{figure/2D005_1_3}	
%					\cput(50,2){\contour{white}{$(e)$}}	
%				\end{overpic}
%	}	
%	\caption{
%		\label{fig:2D005ad} The design region on the left is the whole plane. The design region on the right is the upper half plane.}
%\end{figure*}
%\clearpage

\clearpage
\begin{figure*}[tb]\centering{
		\begin{overpic}			
			[width=0.8\columnwidth,trim={2cm 1cm 2cm 5cm},clip]{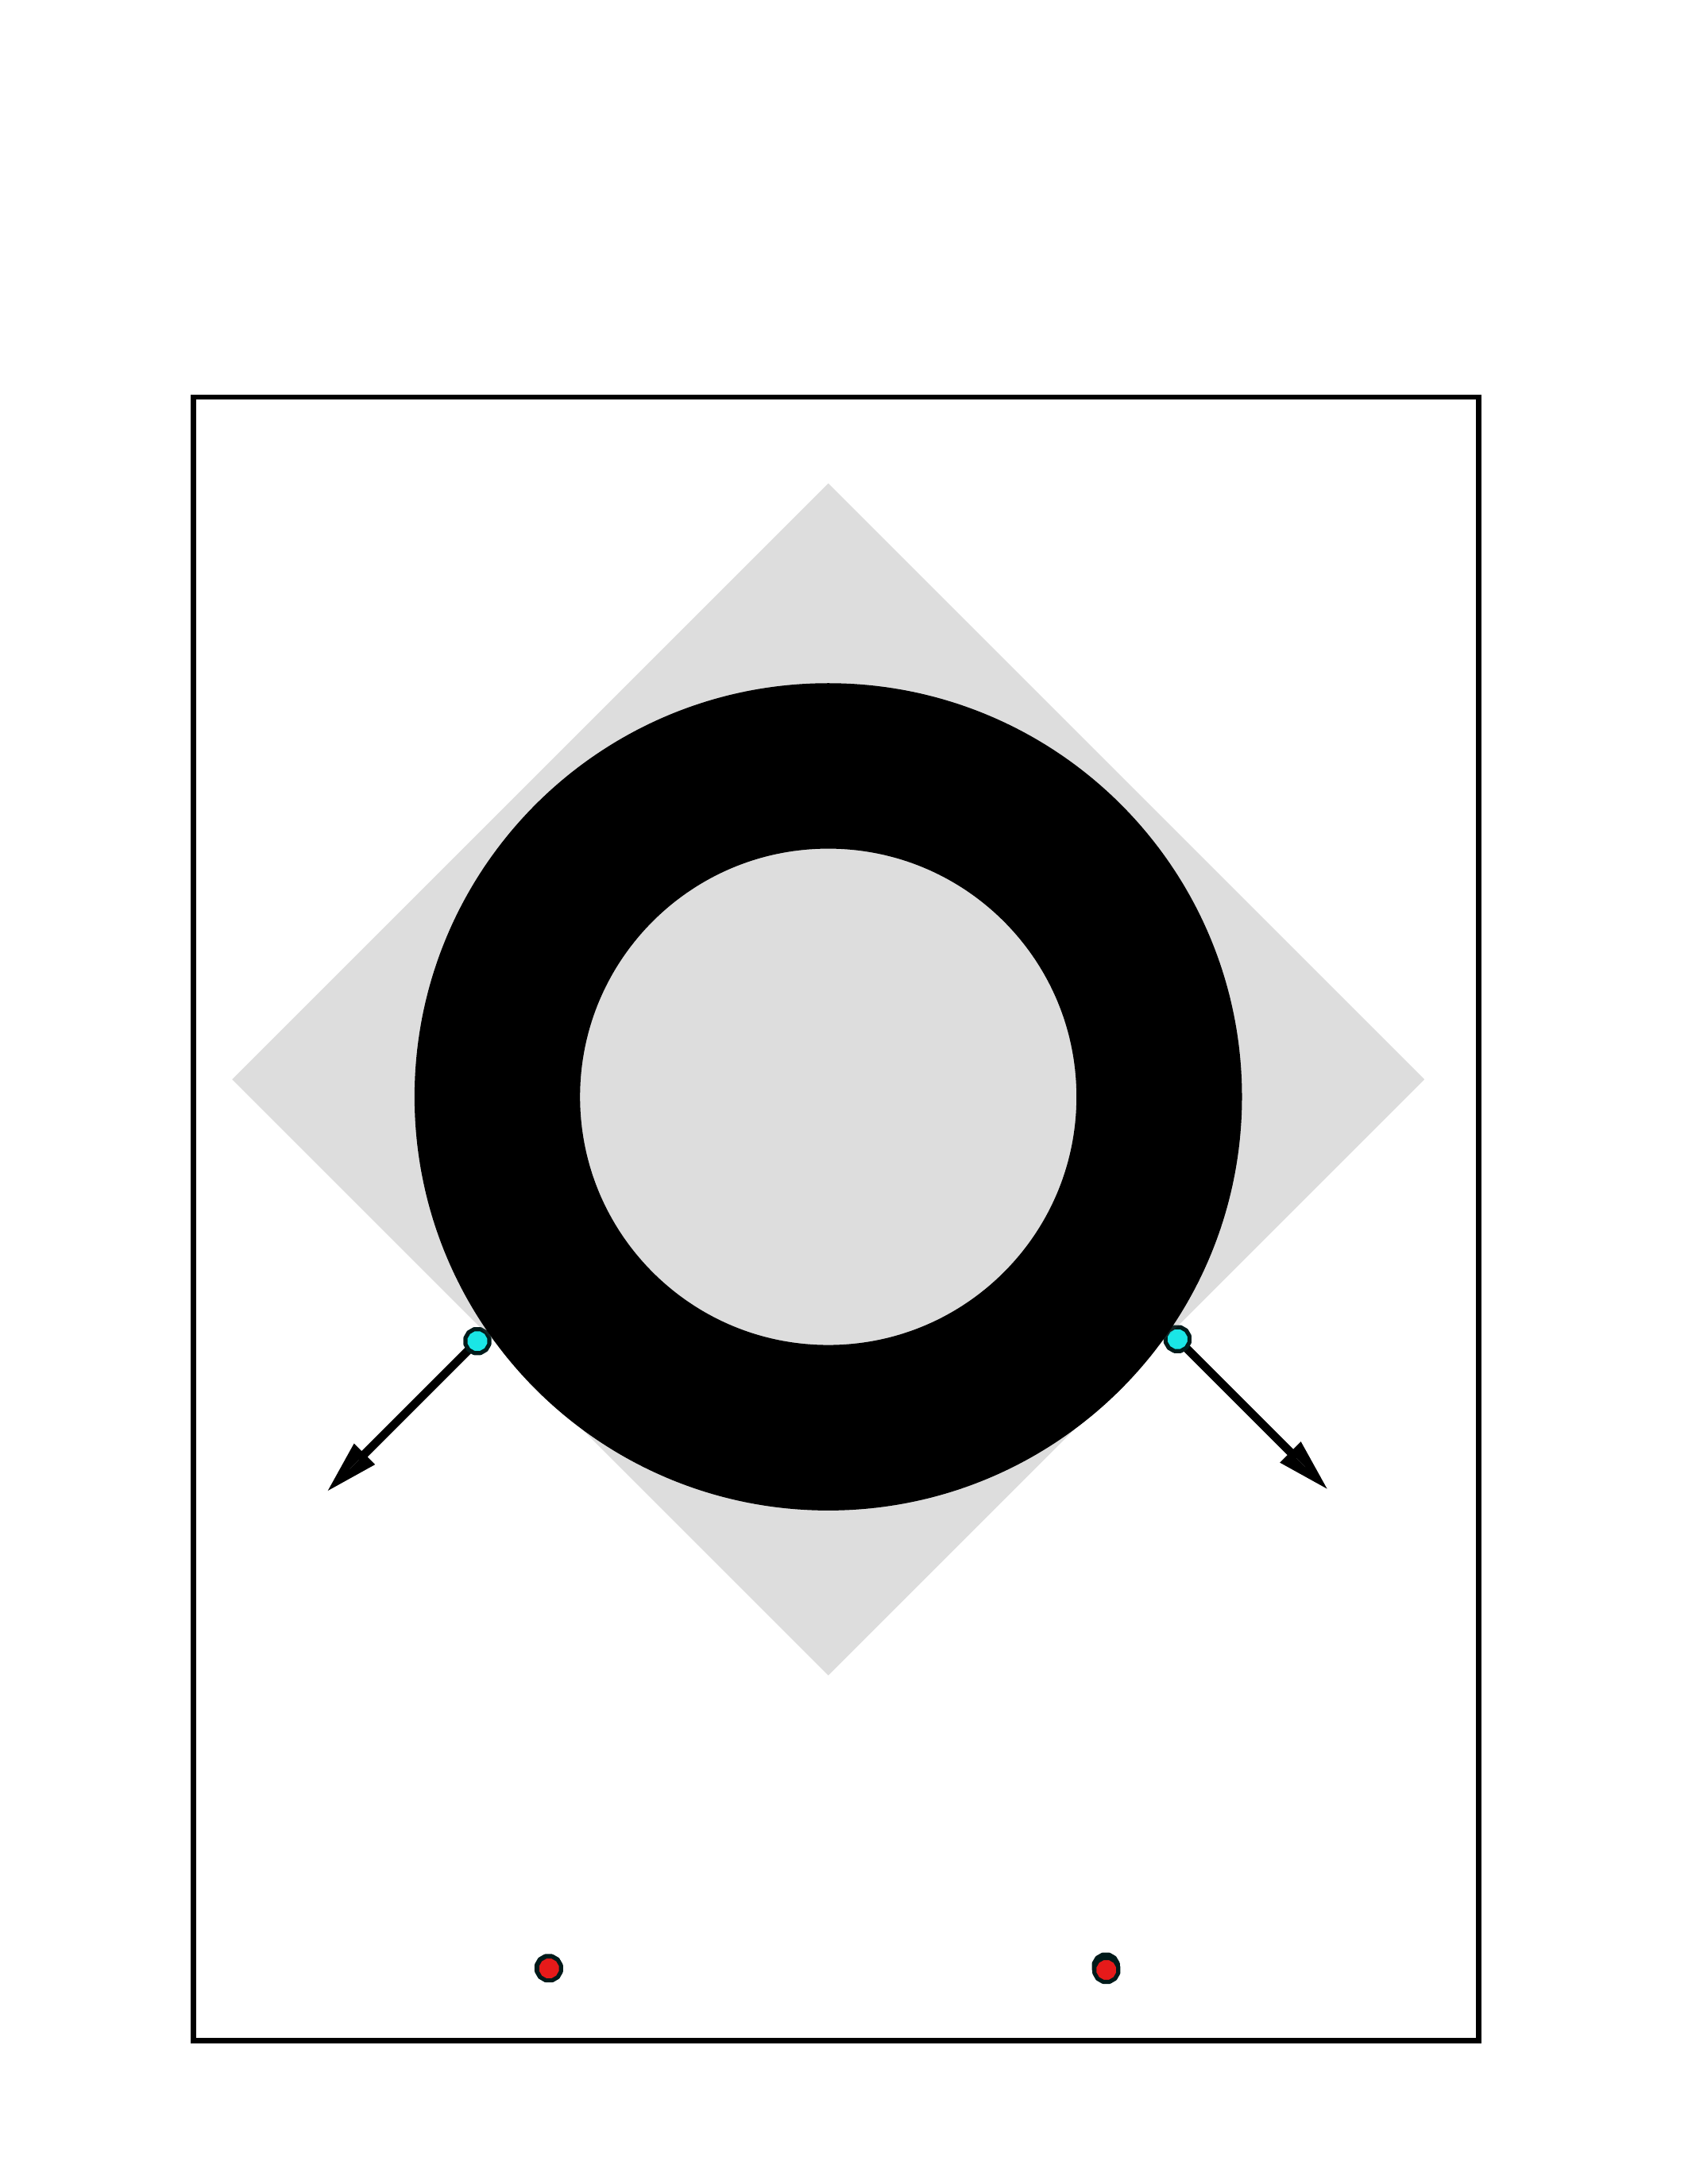}	
			\cput(50,0){\contour{white}{$(a)$}}		
		\end{overpic}
		\begin{overpic}			
			[width=0.8\columnwidth,trim={0cm 5cm 1cm 5cm},clip]{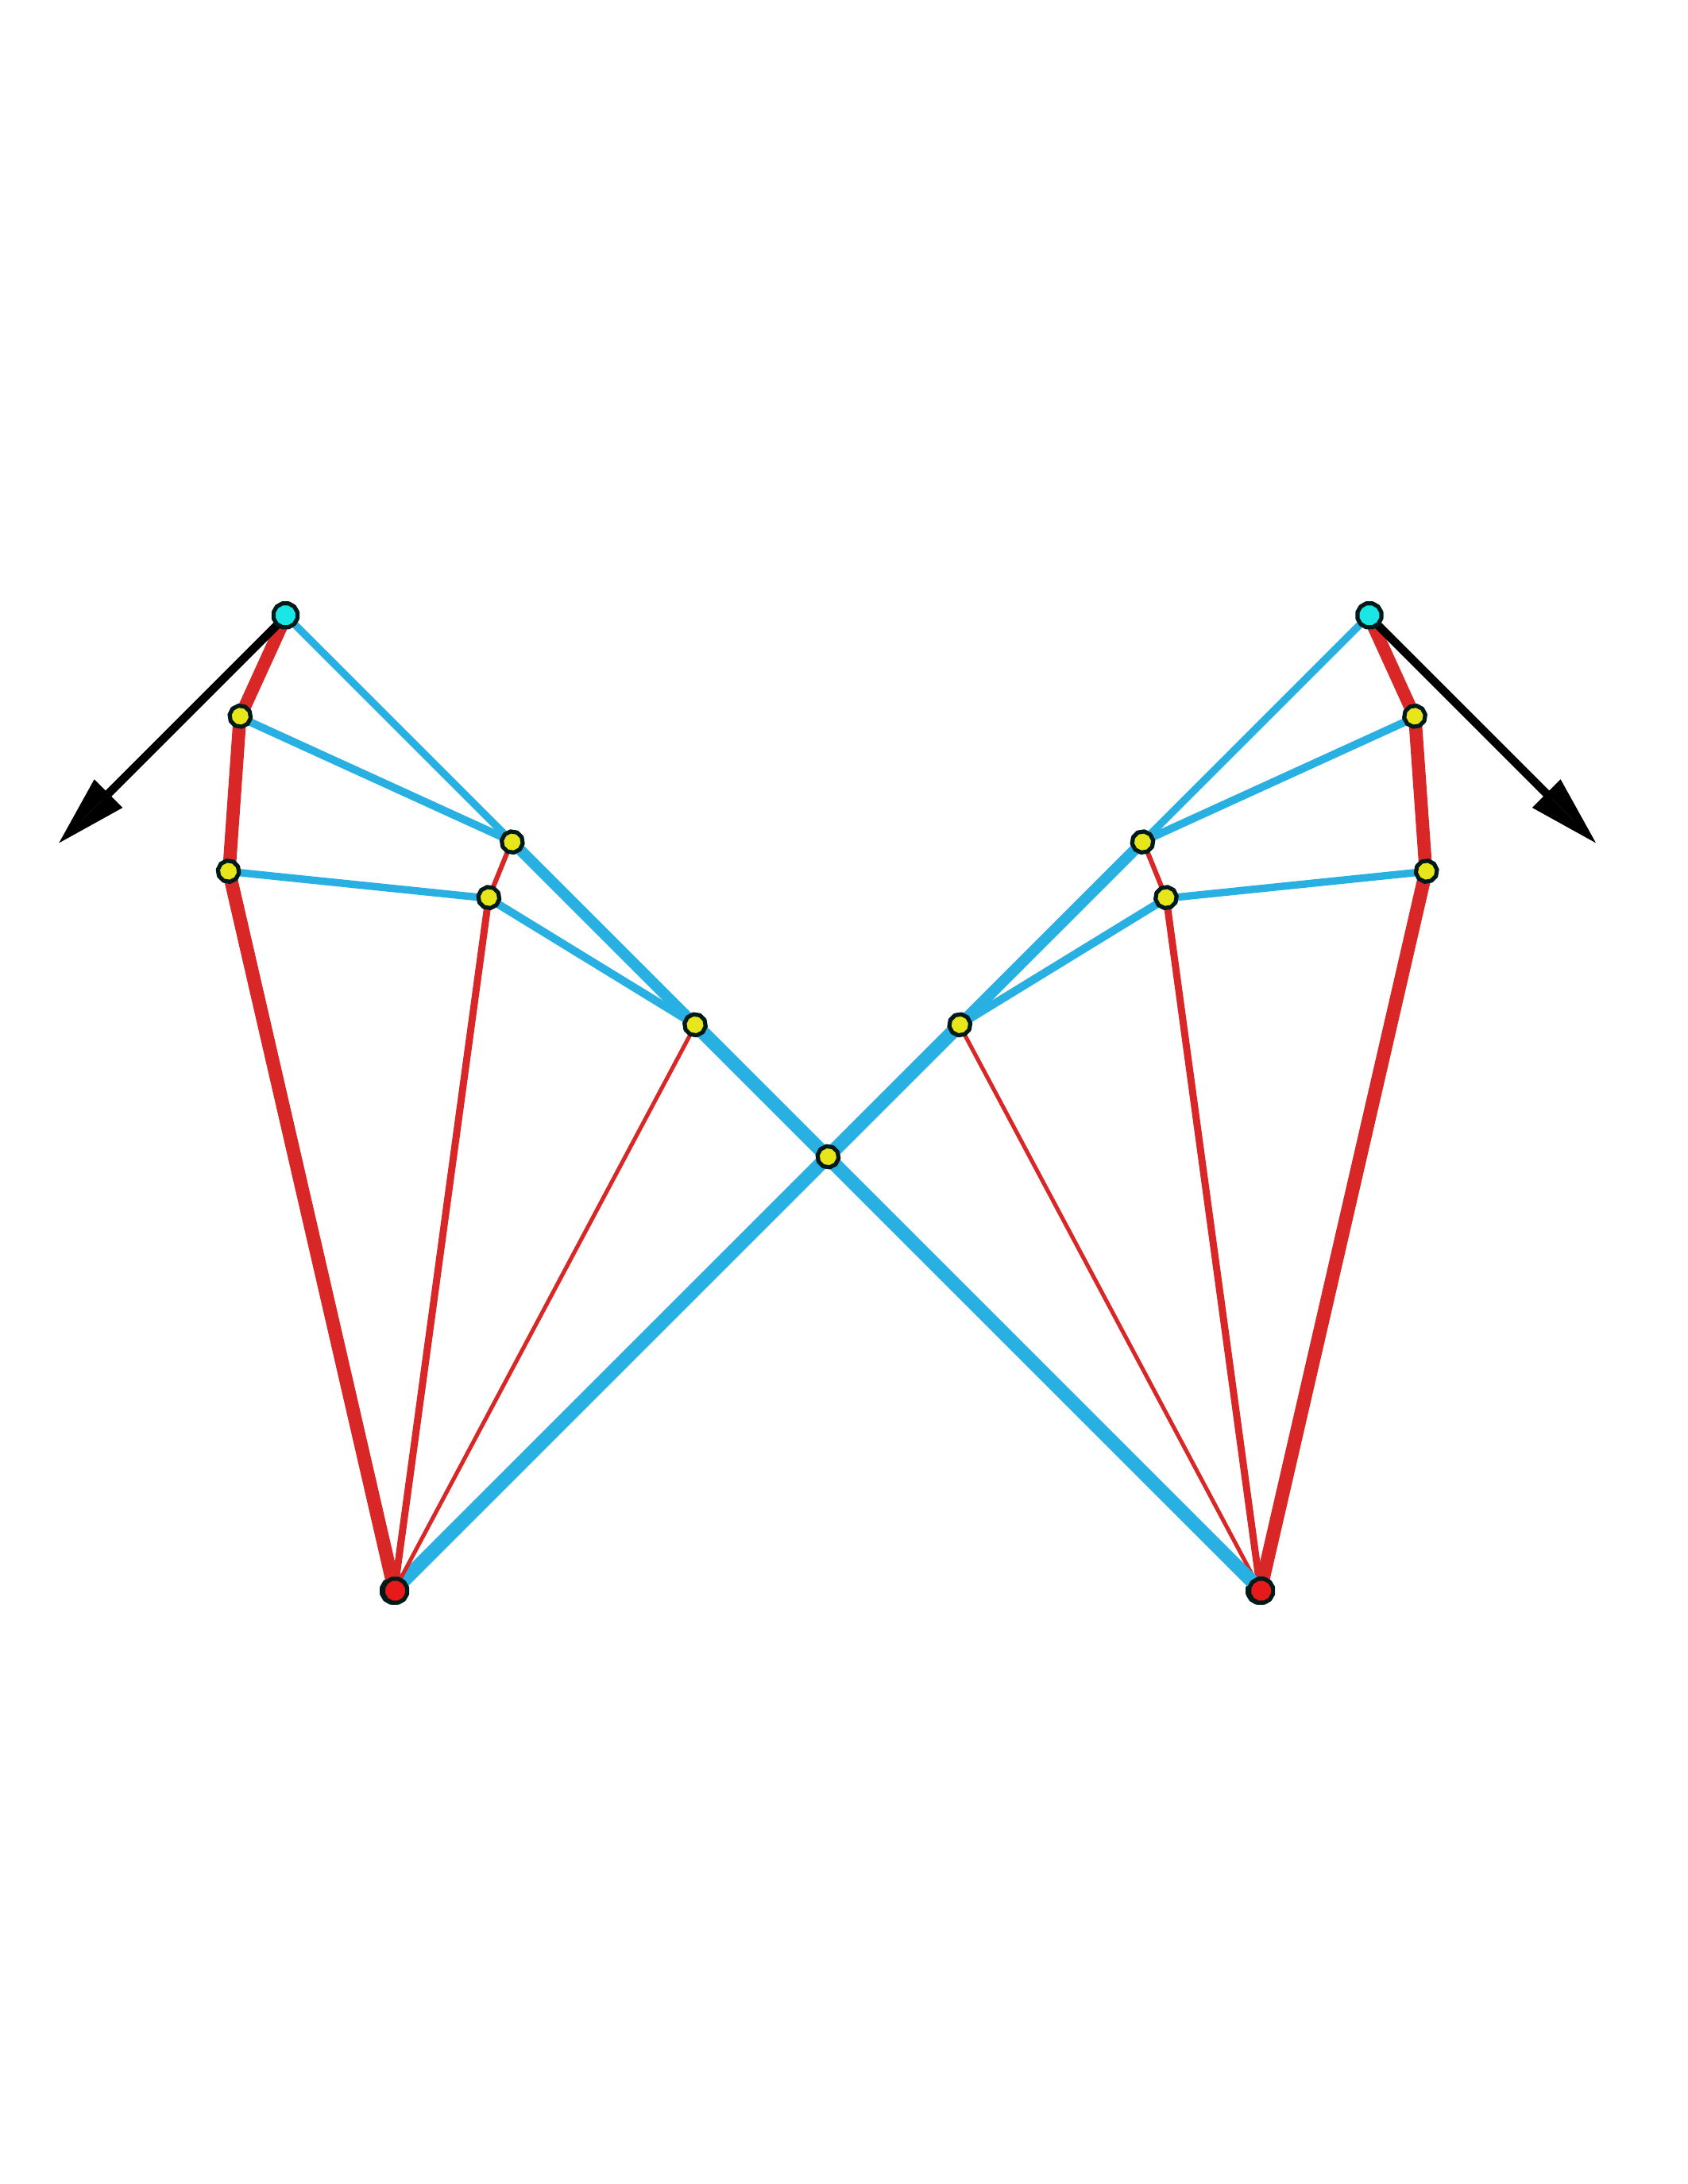}	
			\cput(50,2){\contour{white}{$(b)$}}	
		\end{overpic}
		\begin{overpic}			
			[width=0.8\columnwidth,trim={0cm 5cm 1cm 5cm},clip]{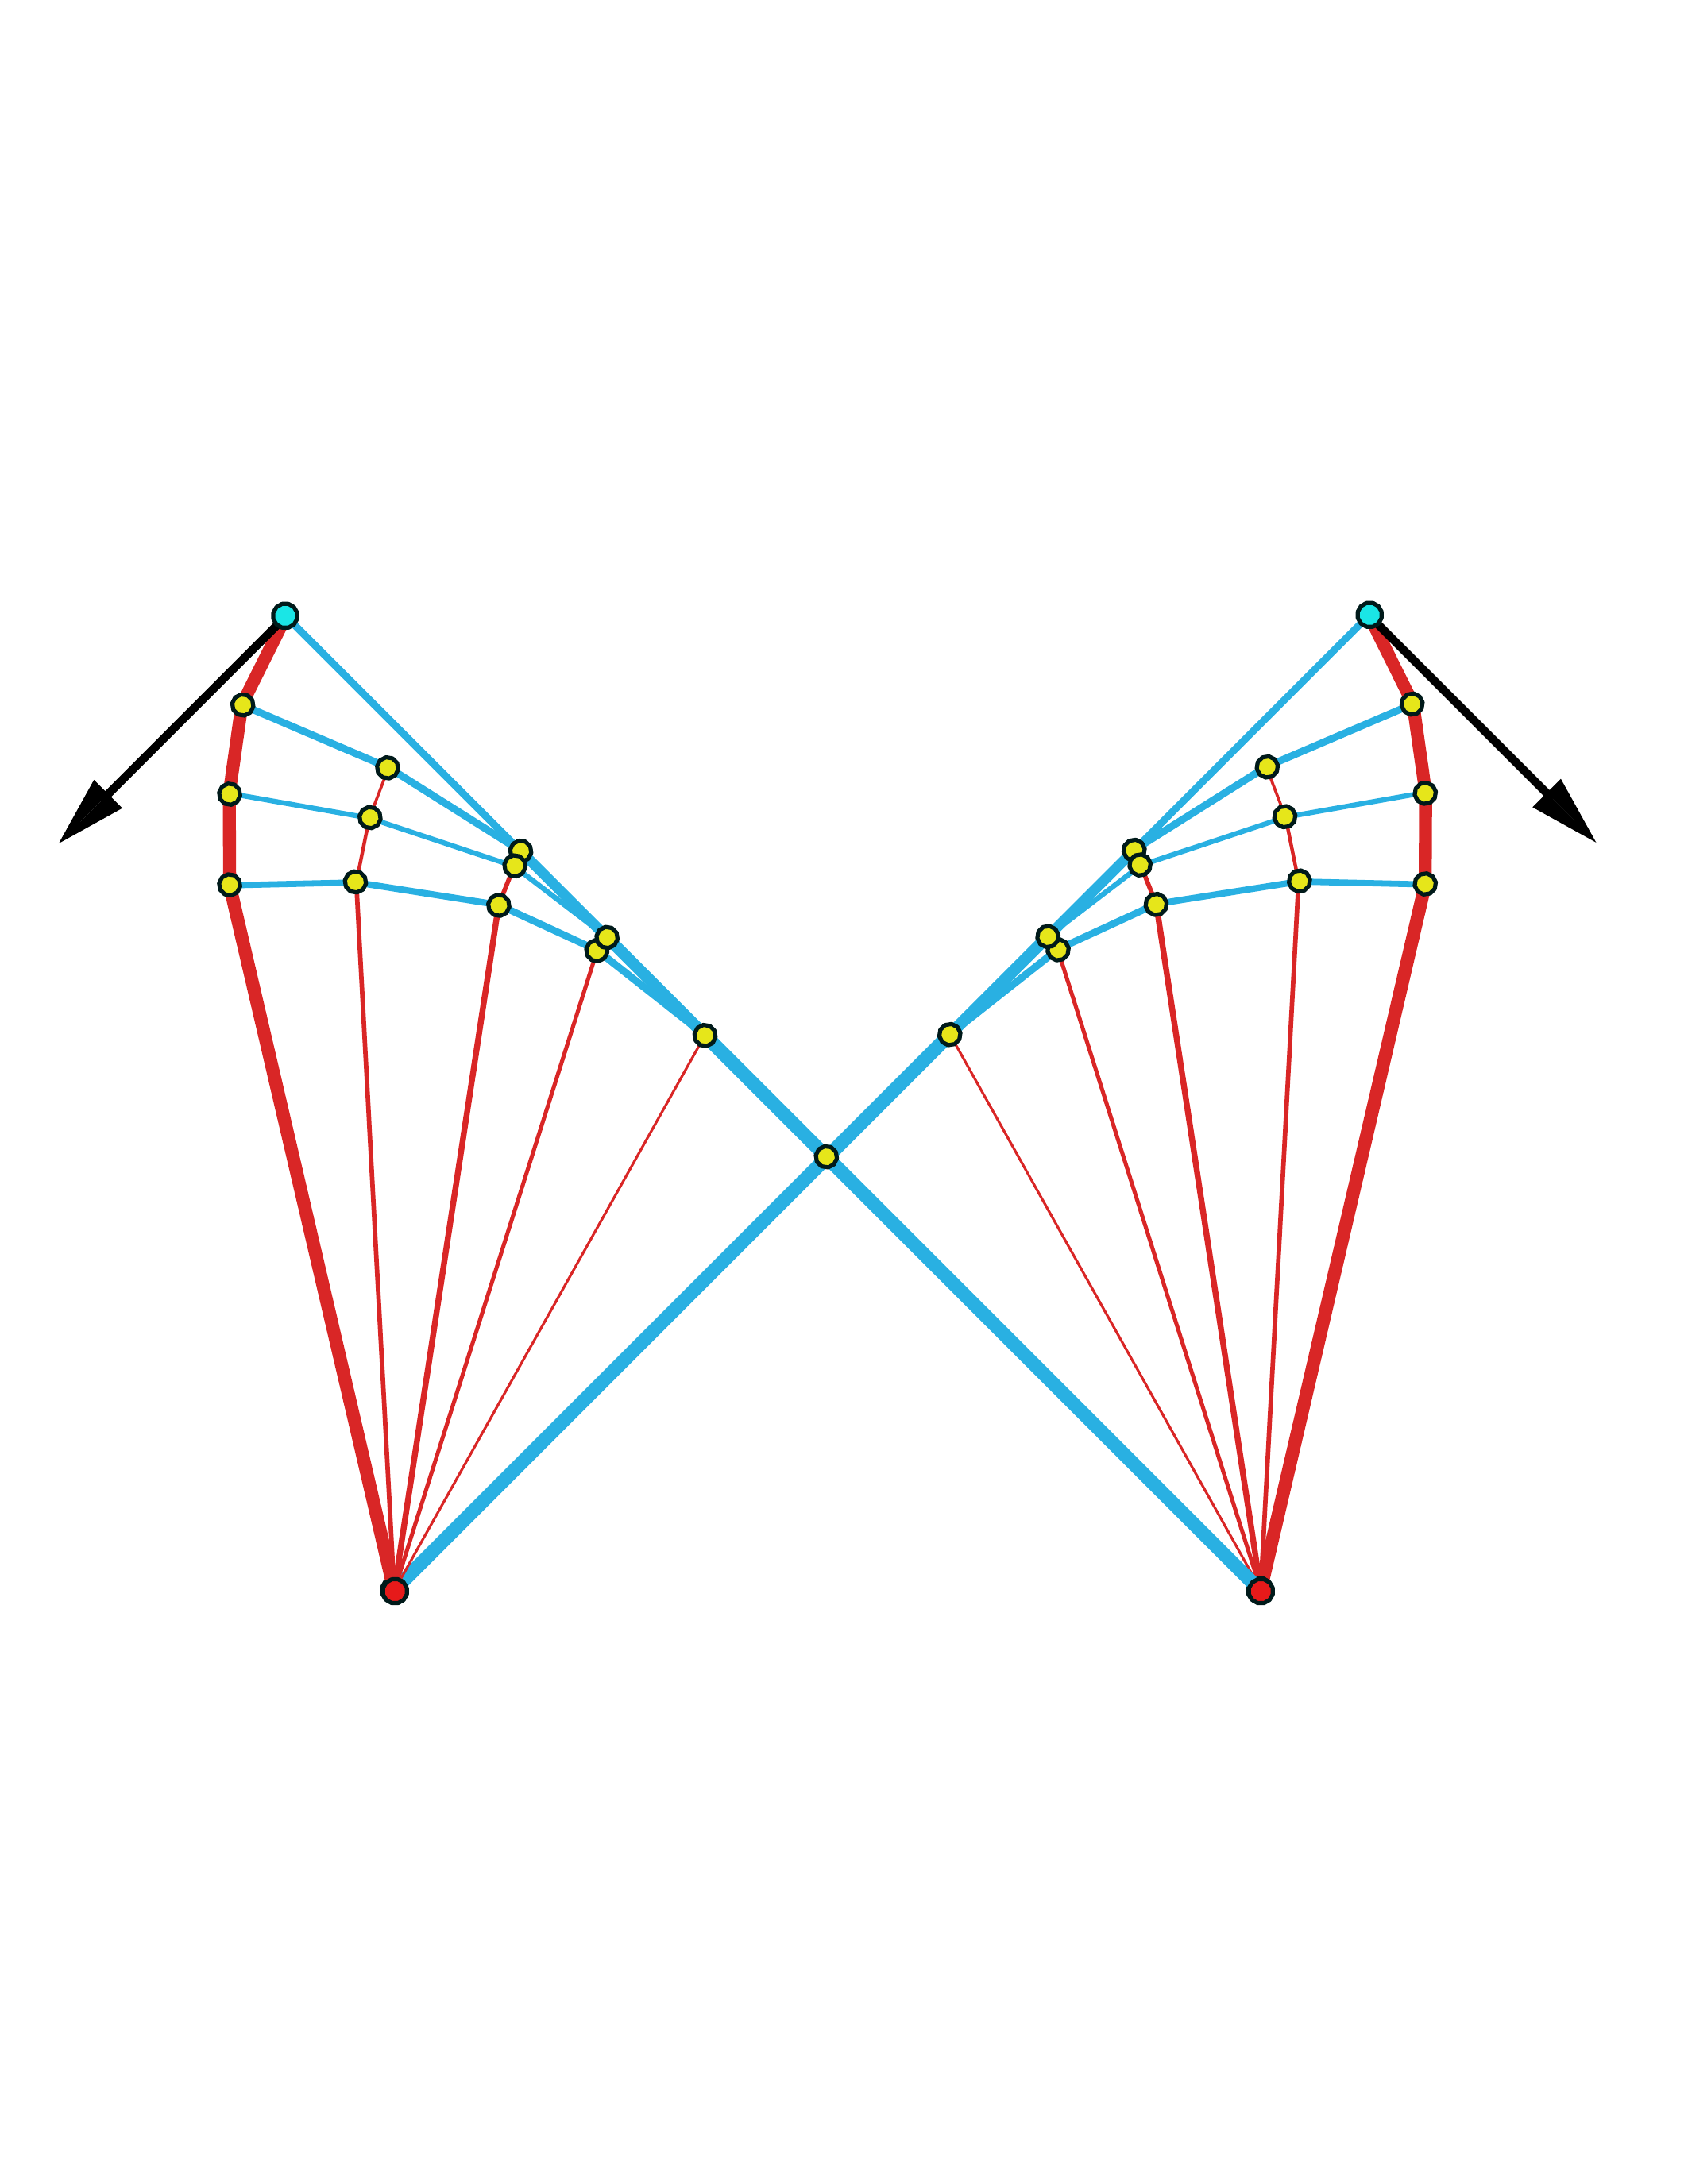}	
			\cput(50,2){\contour{white}{$(c)$}}	
		\end{overpic}
		\begin{overpic}			
			[width=0.8\columnwidth,trim={0cm 5cm 1cm 5cm},clip]{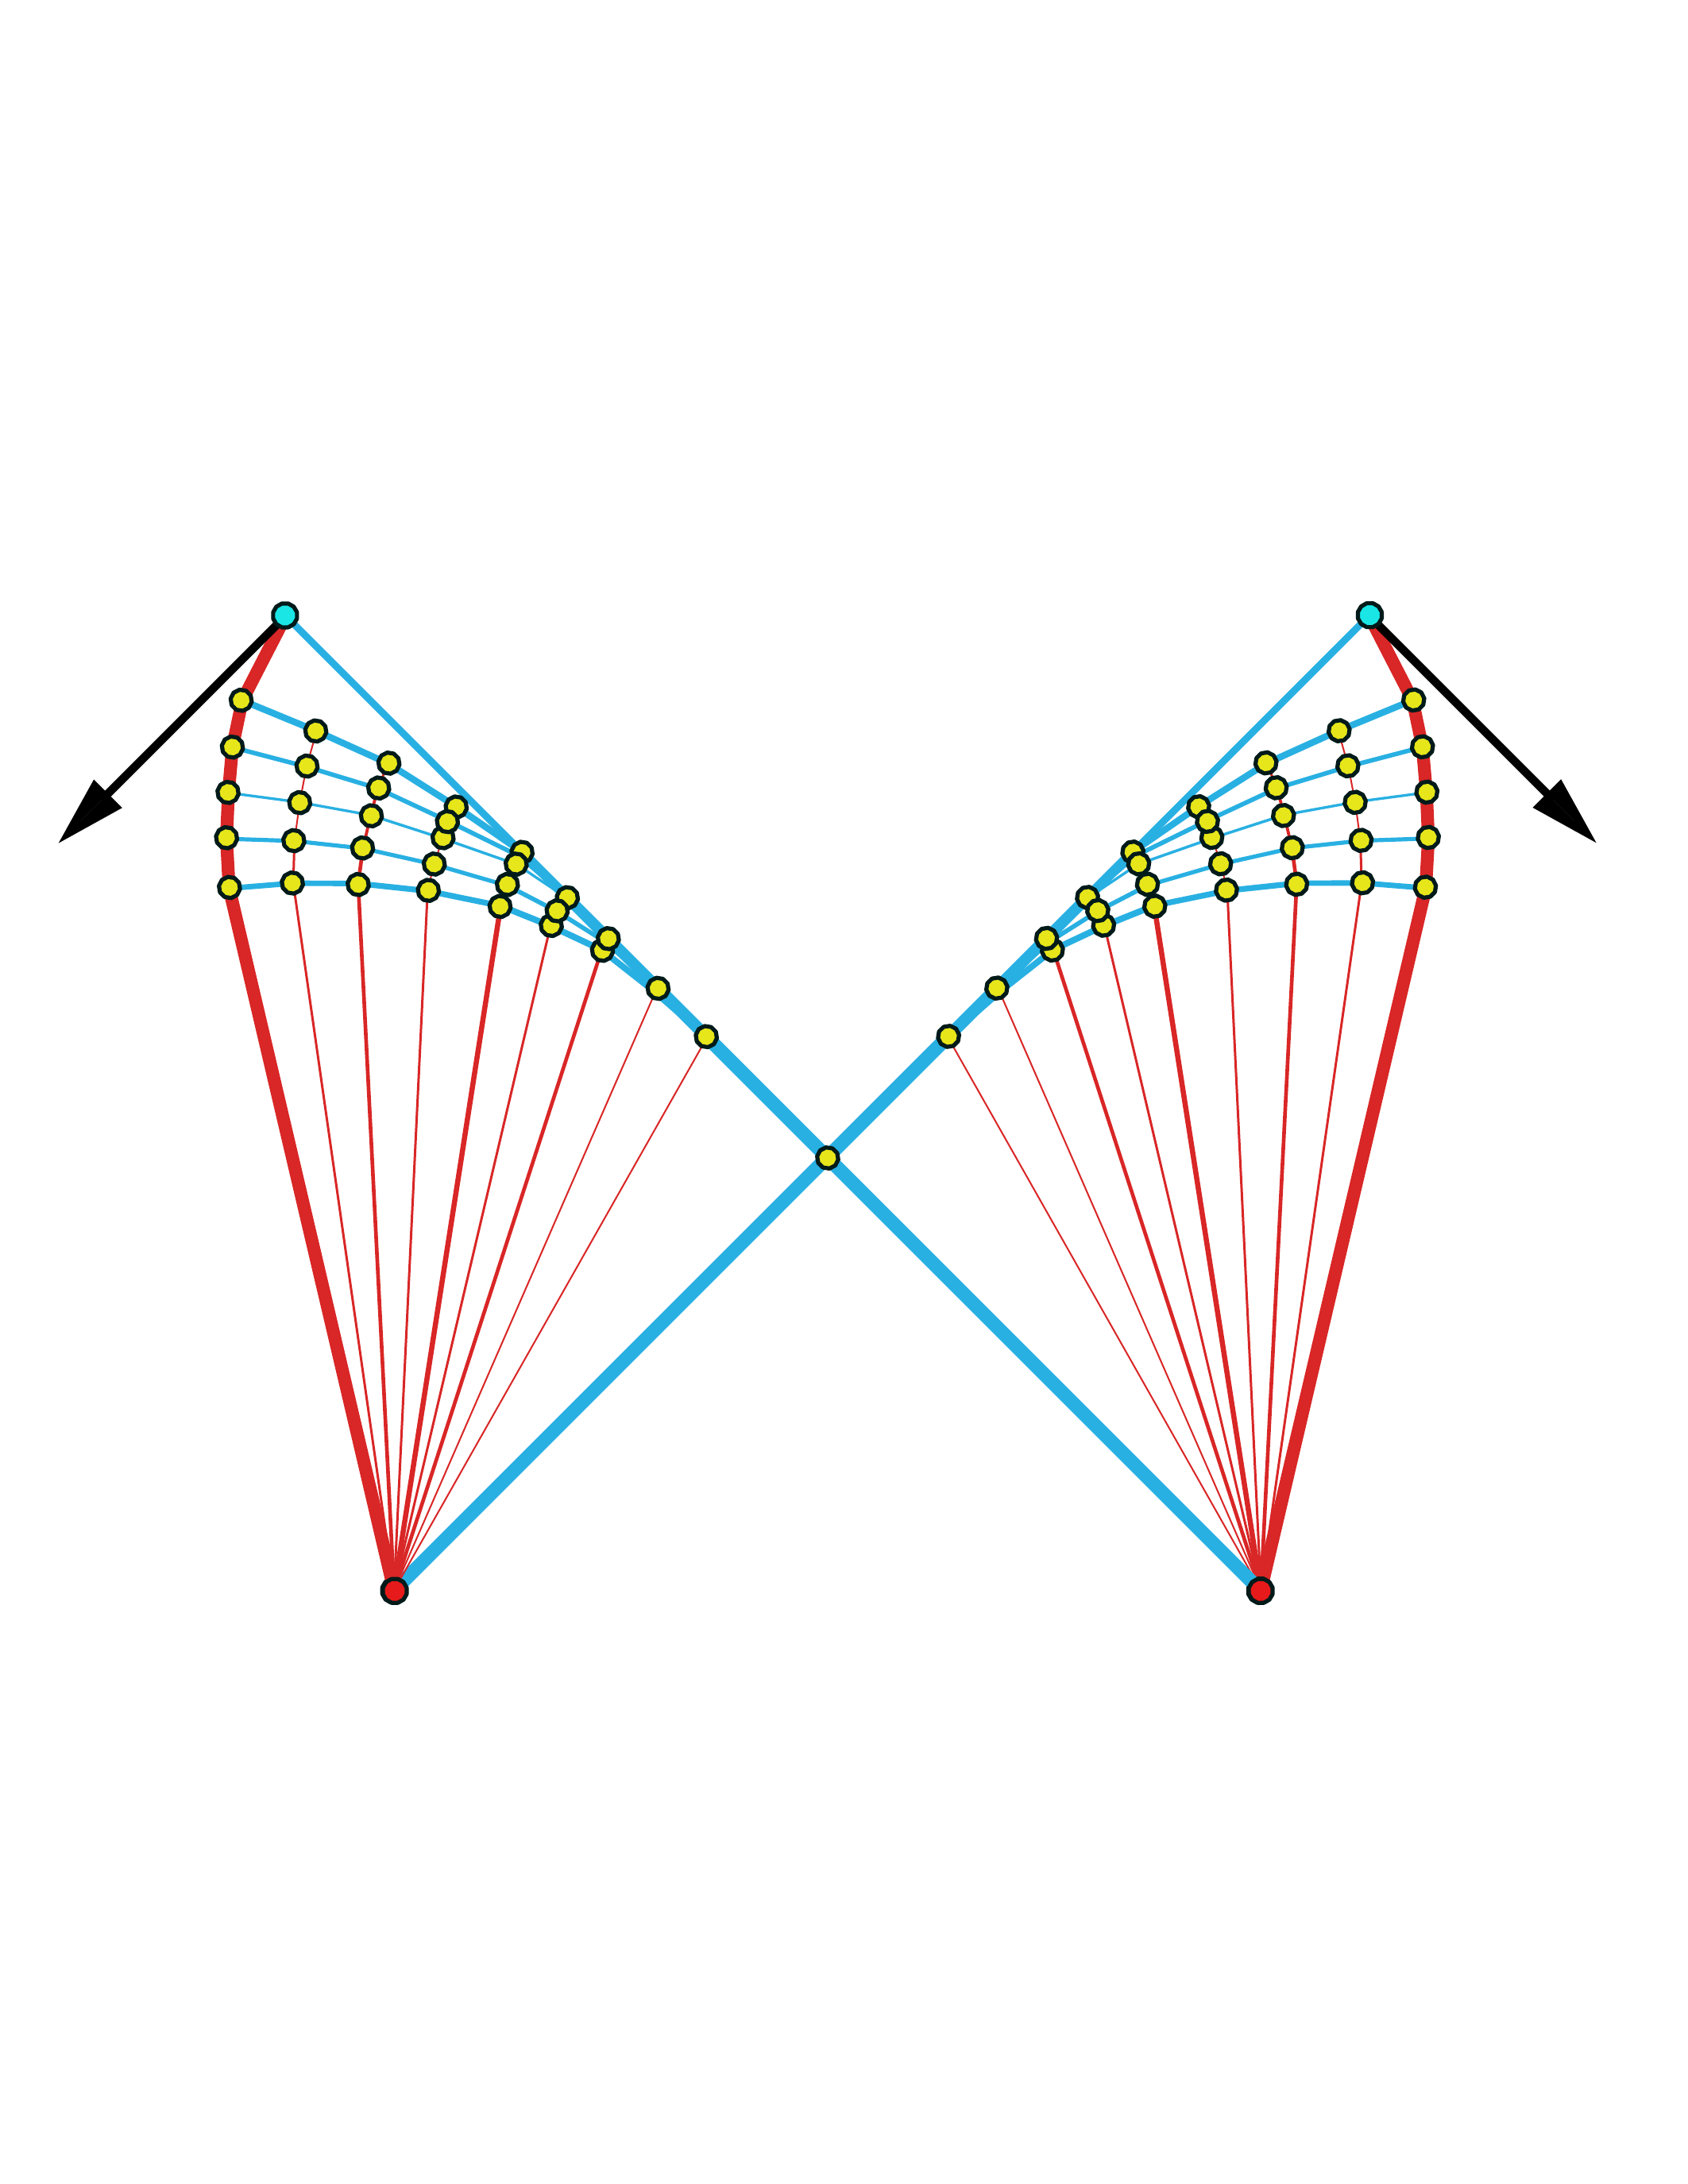}	
			\cput(50,2){\contour{white}{$(d)$}}	
		\end{overpic}
	}	
	\caption{
		\label{fig:2D0025}
	The design purpose is to find a structure to support a cylindrical object(black). The square region (grey) is a forbidden region where no joints and bars are allowed.}
\end{figure*}
\clearpage

\clearpage
\begin{figure*}[tb]	\centering{
				\begin{overpic}			
					[height=.6\columnwidth]{figure/drone}	
					%\cput(50,2){\contour{white}{$(a)$}}		
				\end{overpic}
		\begin{overpic}			
			[height=.8\columnwidth]{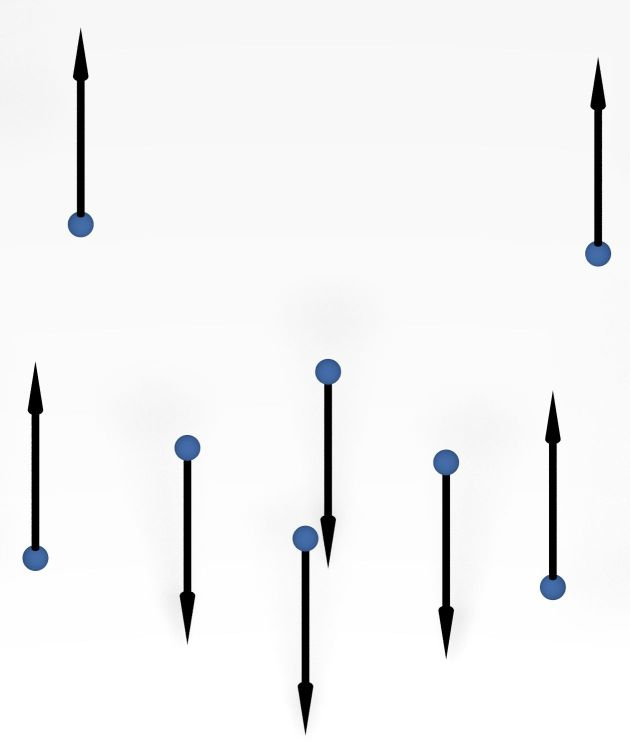}	
			%\cput(50,2){\contour{white}{$(a)$}}		
		\end{overpic}
		\begin{overpic}			
			[height=.8\columnwidth]{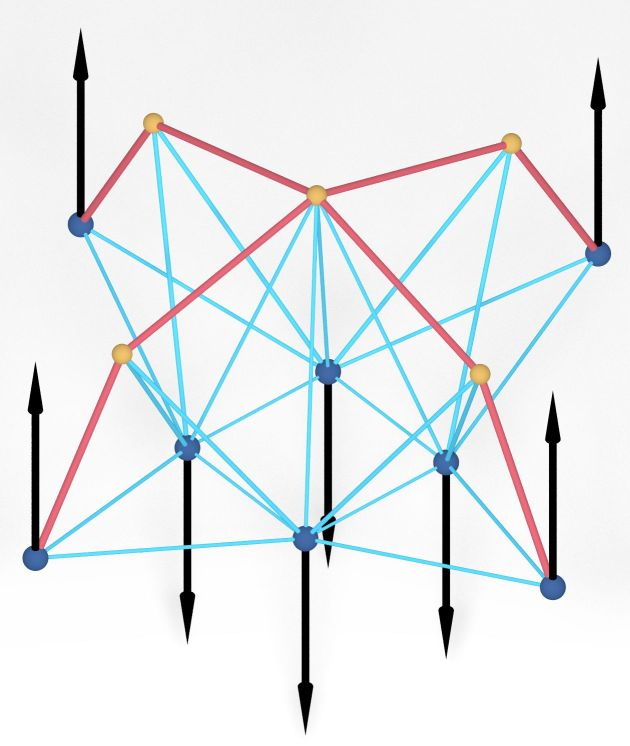}	
			\cput(20,2){\contour{white}{$(a)$}}		
		\end{overpic}
		\begin{overpic}			
			[height=.8\columnwidth]{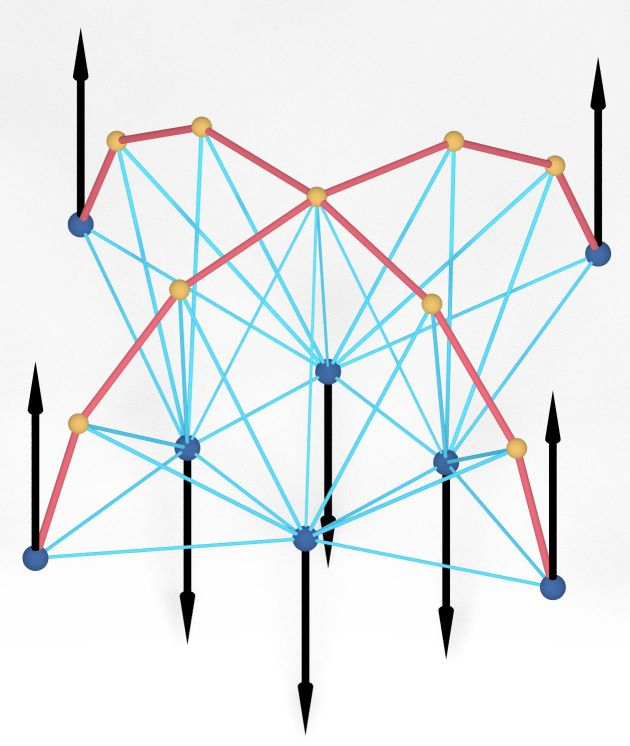}	
			\cput(20,2){\contour{white}{$(b)$}}	
		\end{overpic}
		\begin{overpic}			
			[height=.8\columnwidth]{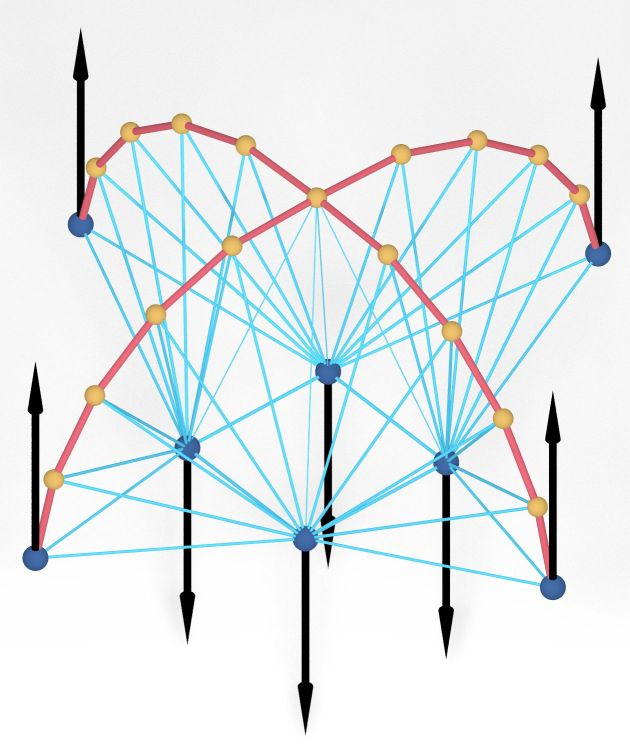}
			\cput(20,0){\contour{white}{$(c)$}}		
		\end{overpic}
		\begin{overpic}			
			[height=.8\columnwidth]{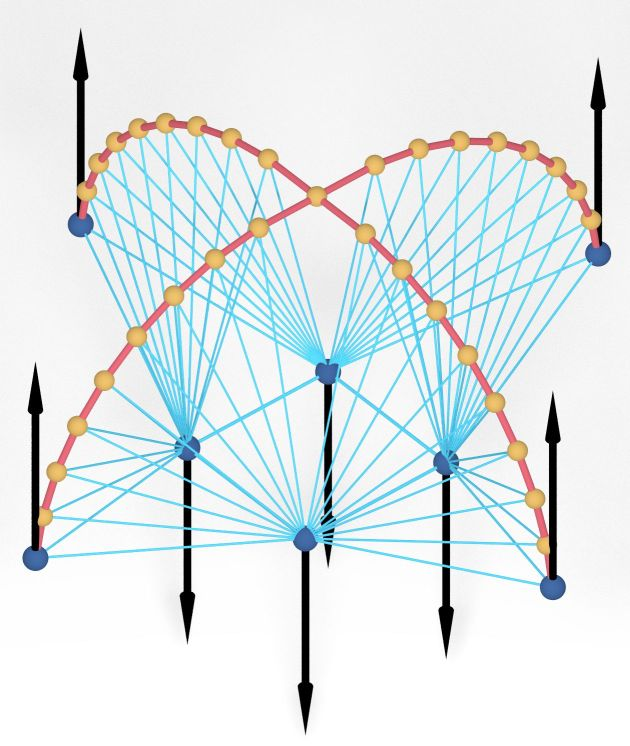}	
			\cput(20,0){\contour{white}{$(d)$}}		
		\end{overpic}
	}	
	\caption{
		\label{fig:parallelforce3D}
		Input functional specification is a 3D parallel force system}
\end{figure*}
\clearpage

\clearpage
\begin{figure*}[tb]	\centering{
		\begin{overpic}			
			[height=.75\columnwidth,trim={20cm 1cm 20cm 1cm},clip]{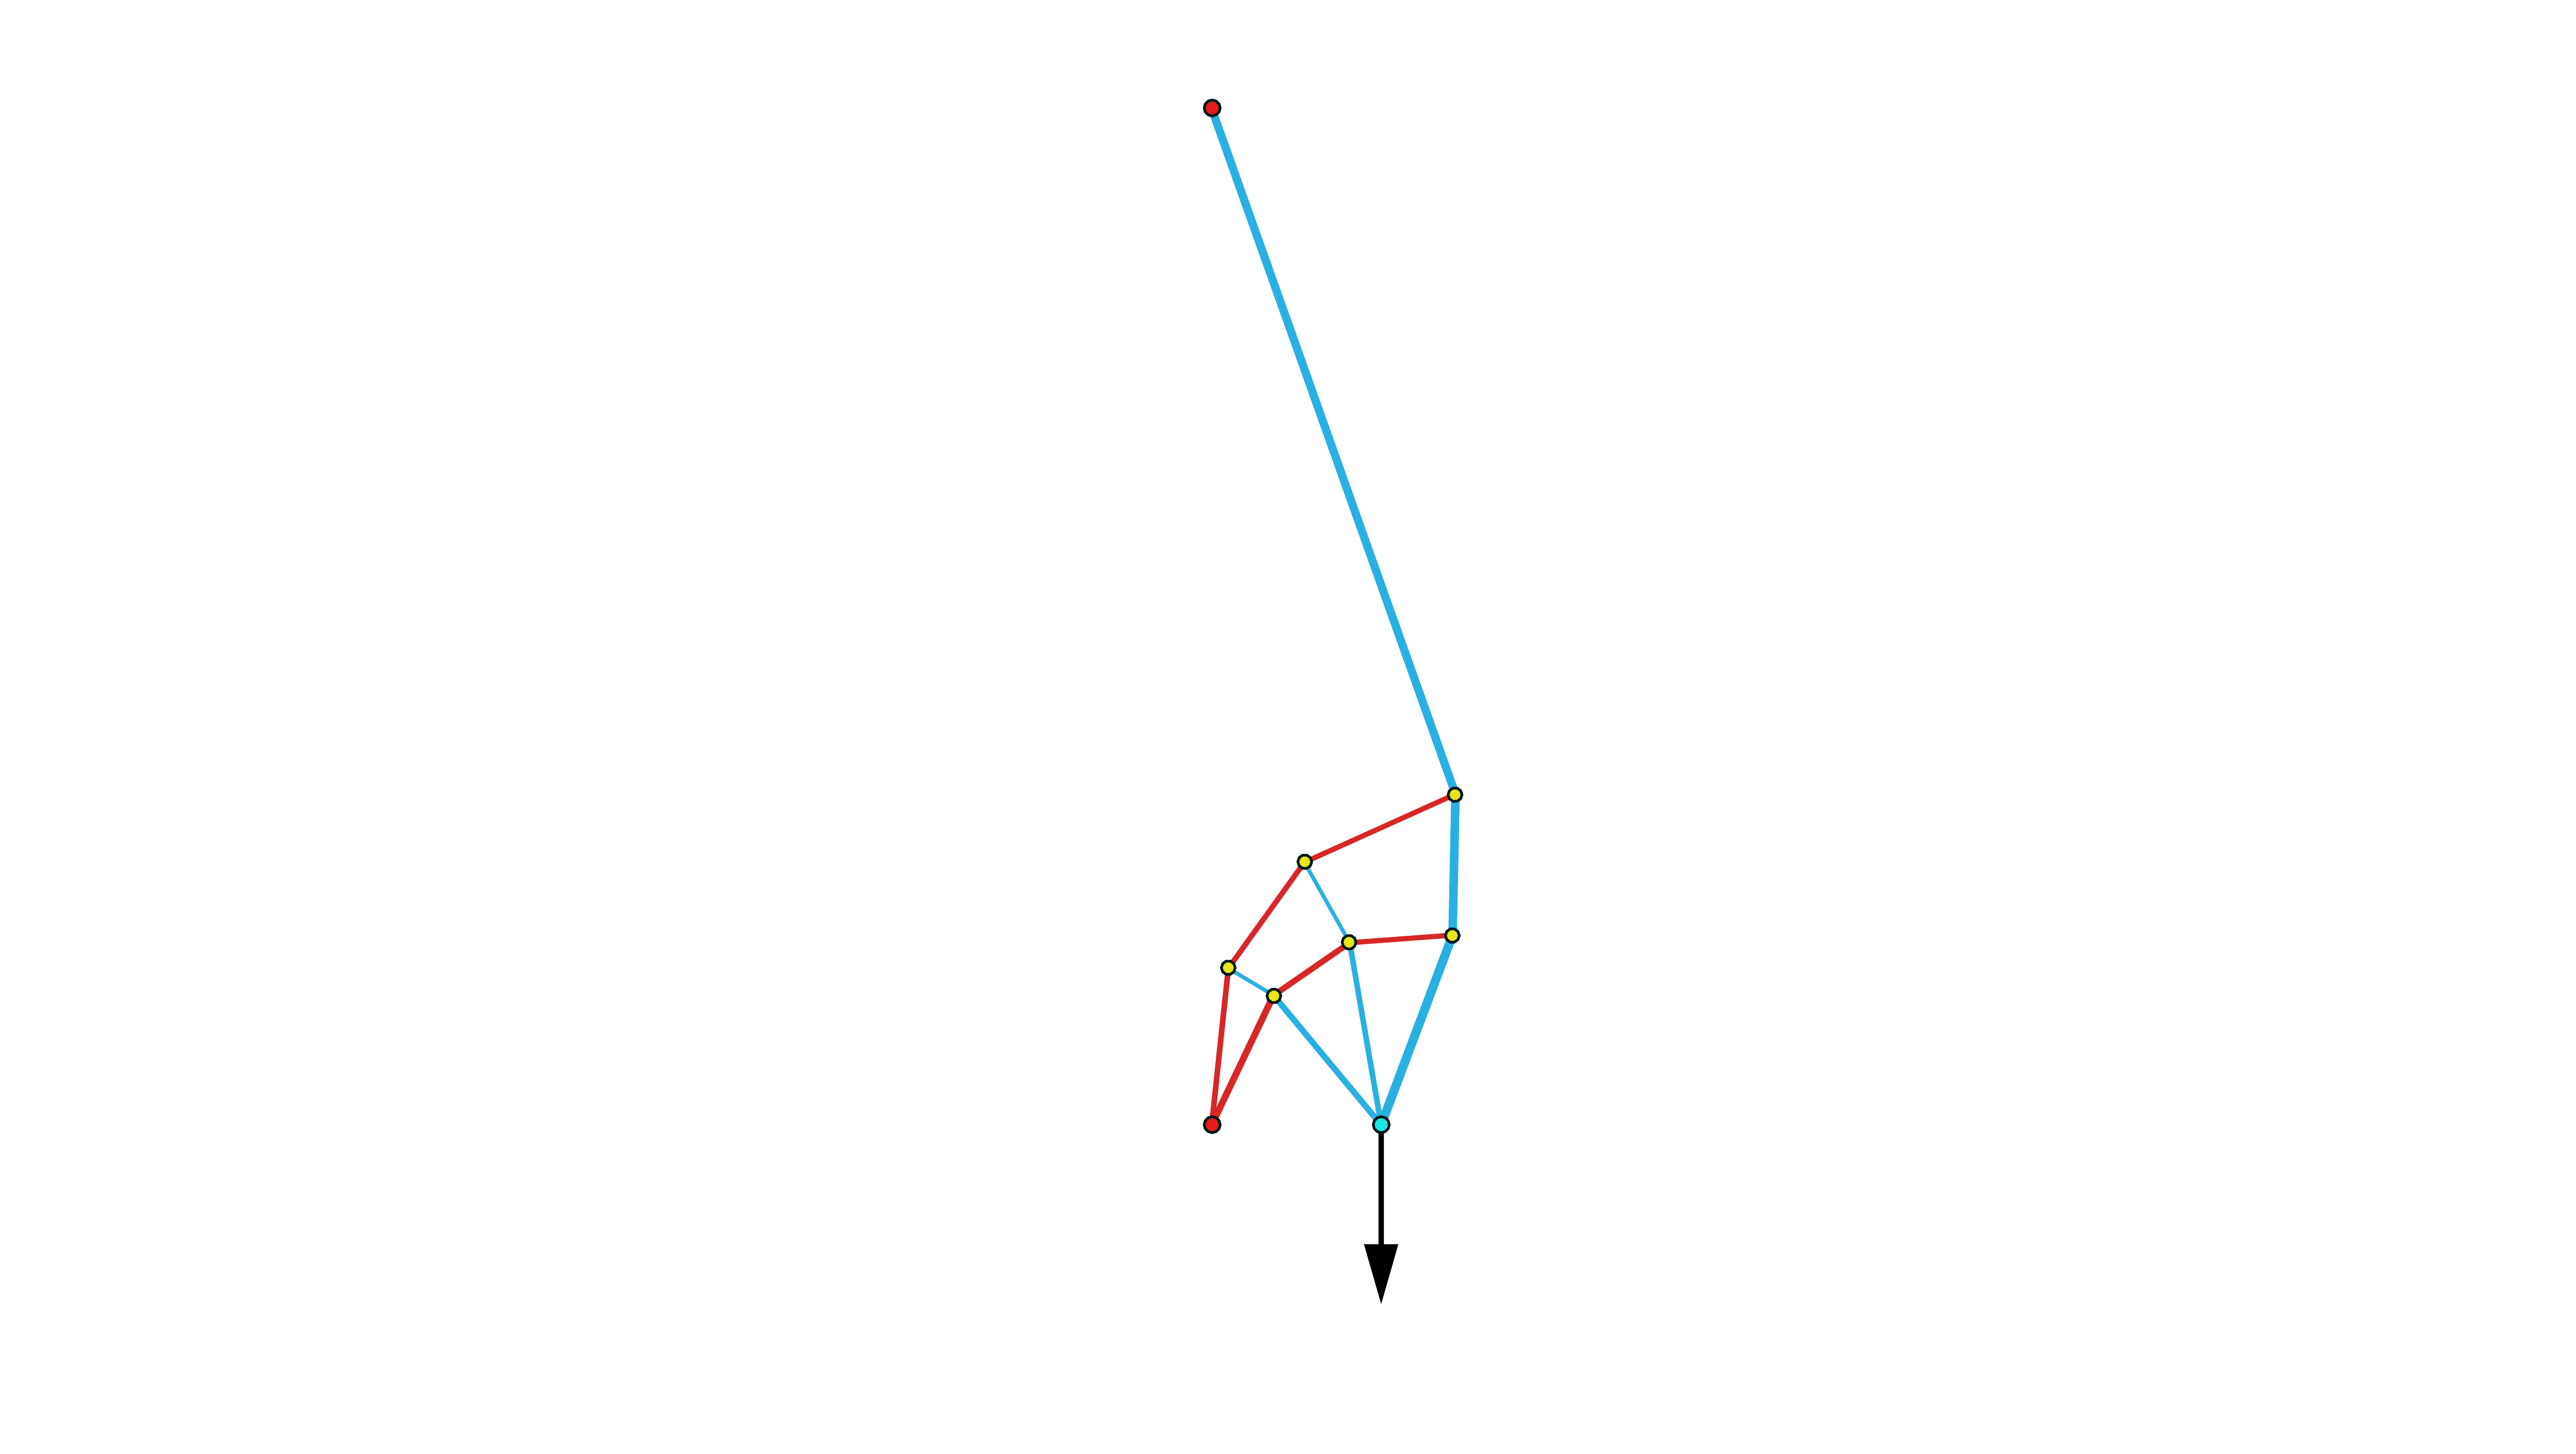}	
			%\cput(50,2){\contour{white}{$(a)$}}		
		\end{overpic}
		\begin{overpic}			
			[height=.75\columnwidth,trim={20cm 1cm 20cm 1cm},clip]{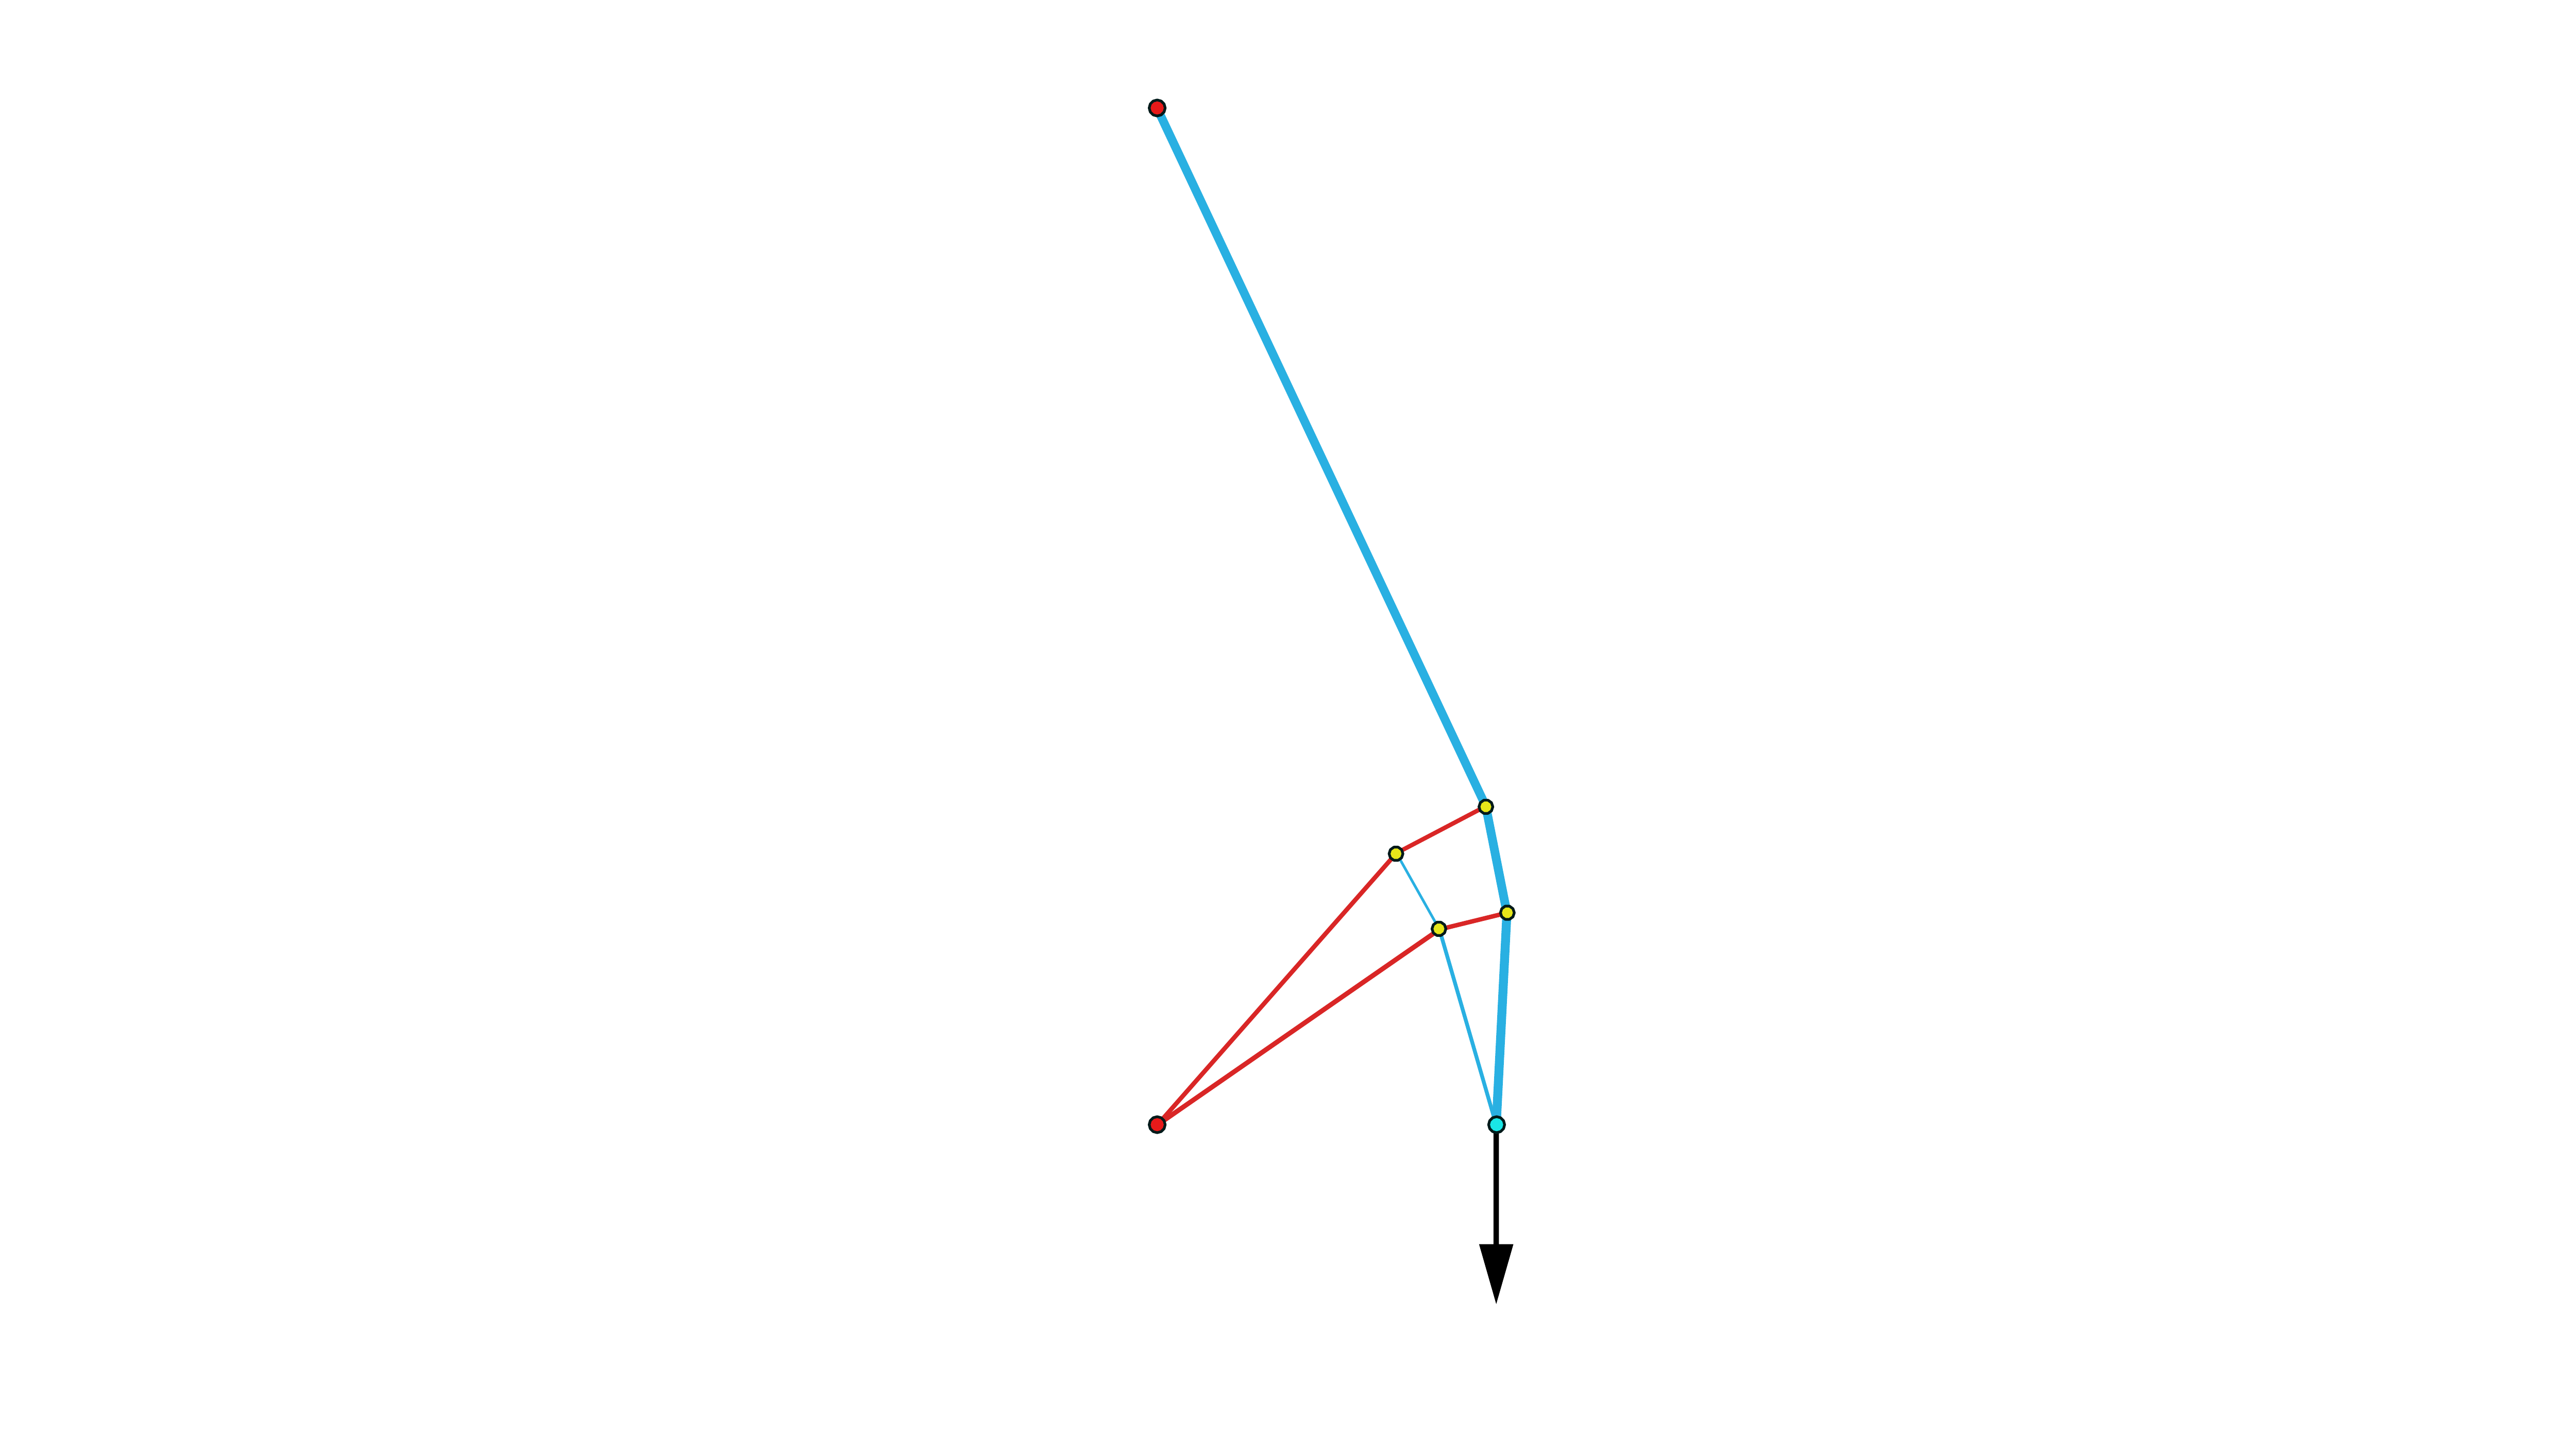}	
			%	\cput(50,2){\contour{white}{$(a)$}}		
		\end{overpic}
		\begin{overpic}			
			[height=.75\columnwidth,trim={18cm 1cm 15cm 1cm},clip]{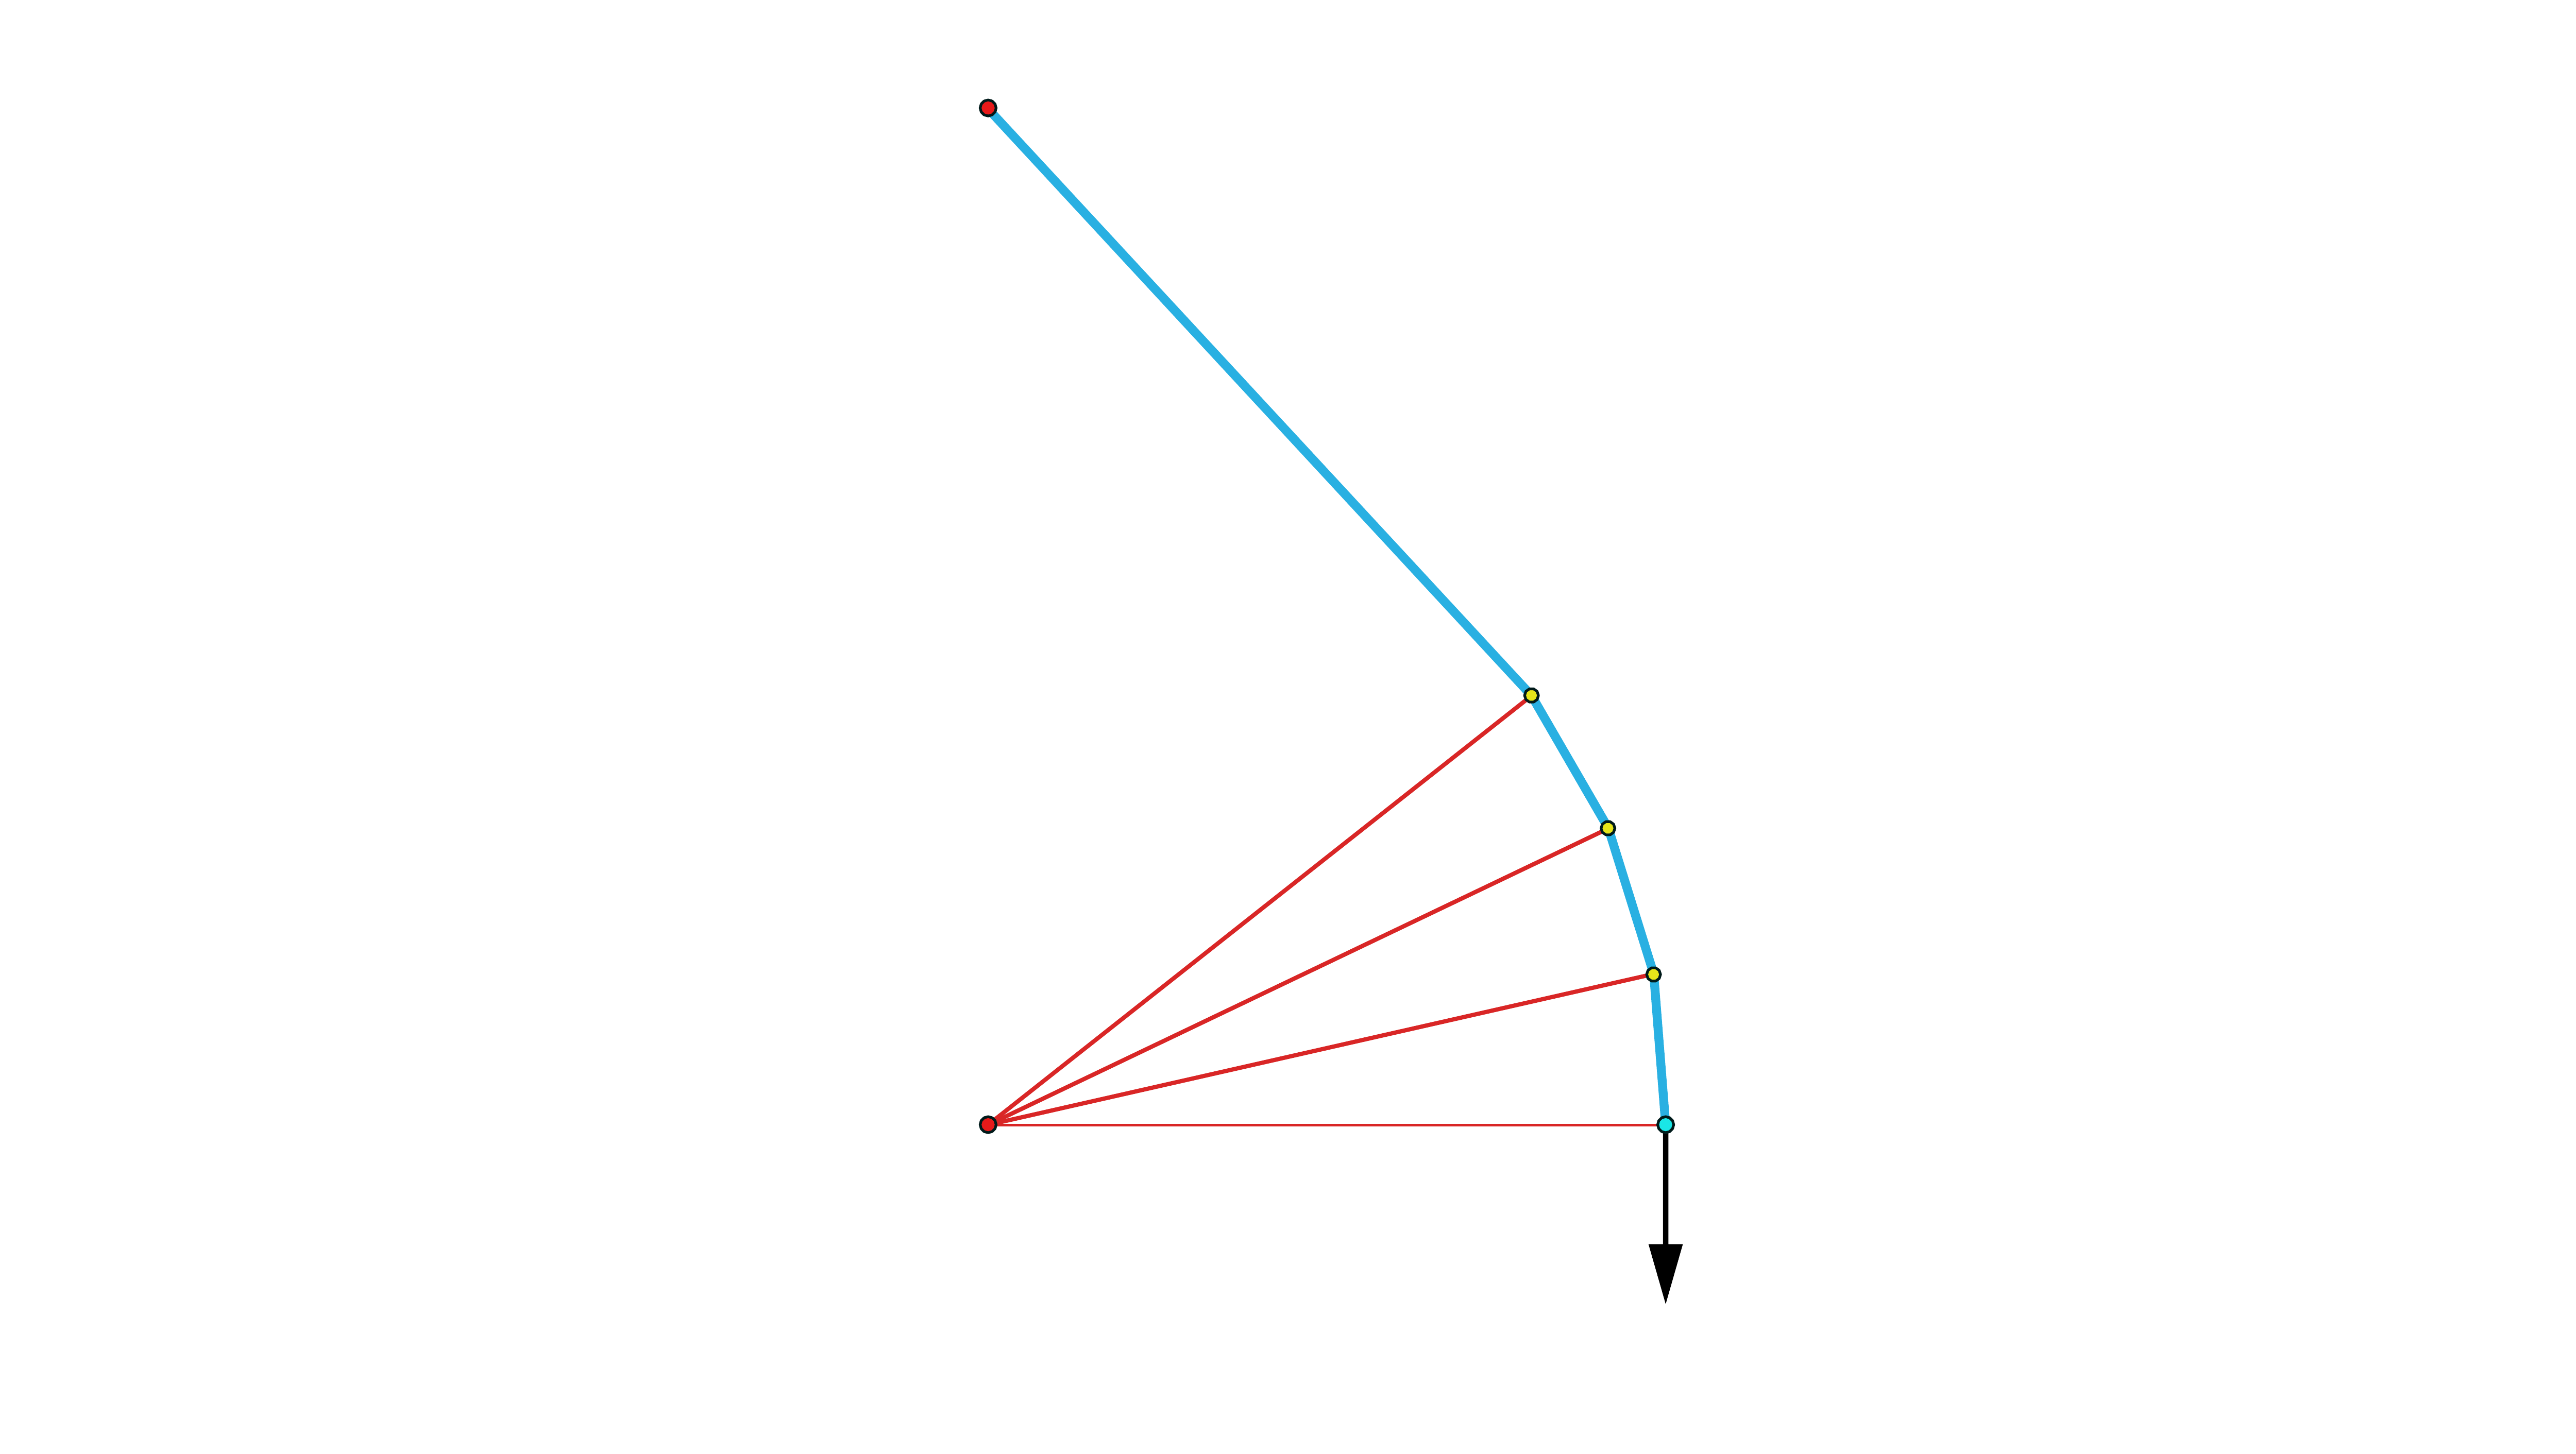}	
			%	\cput(50,2){\contour{white}{$(a)$}}			
		\end{overpic}
		\begin{overpic}			
			[height=.75\columnwidth,trim={12.5cm 1cm 10cm 1cm},clip]{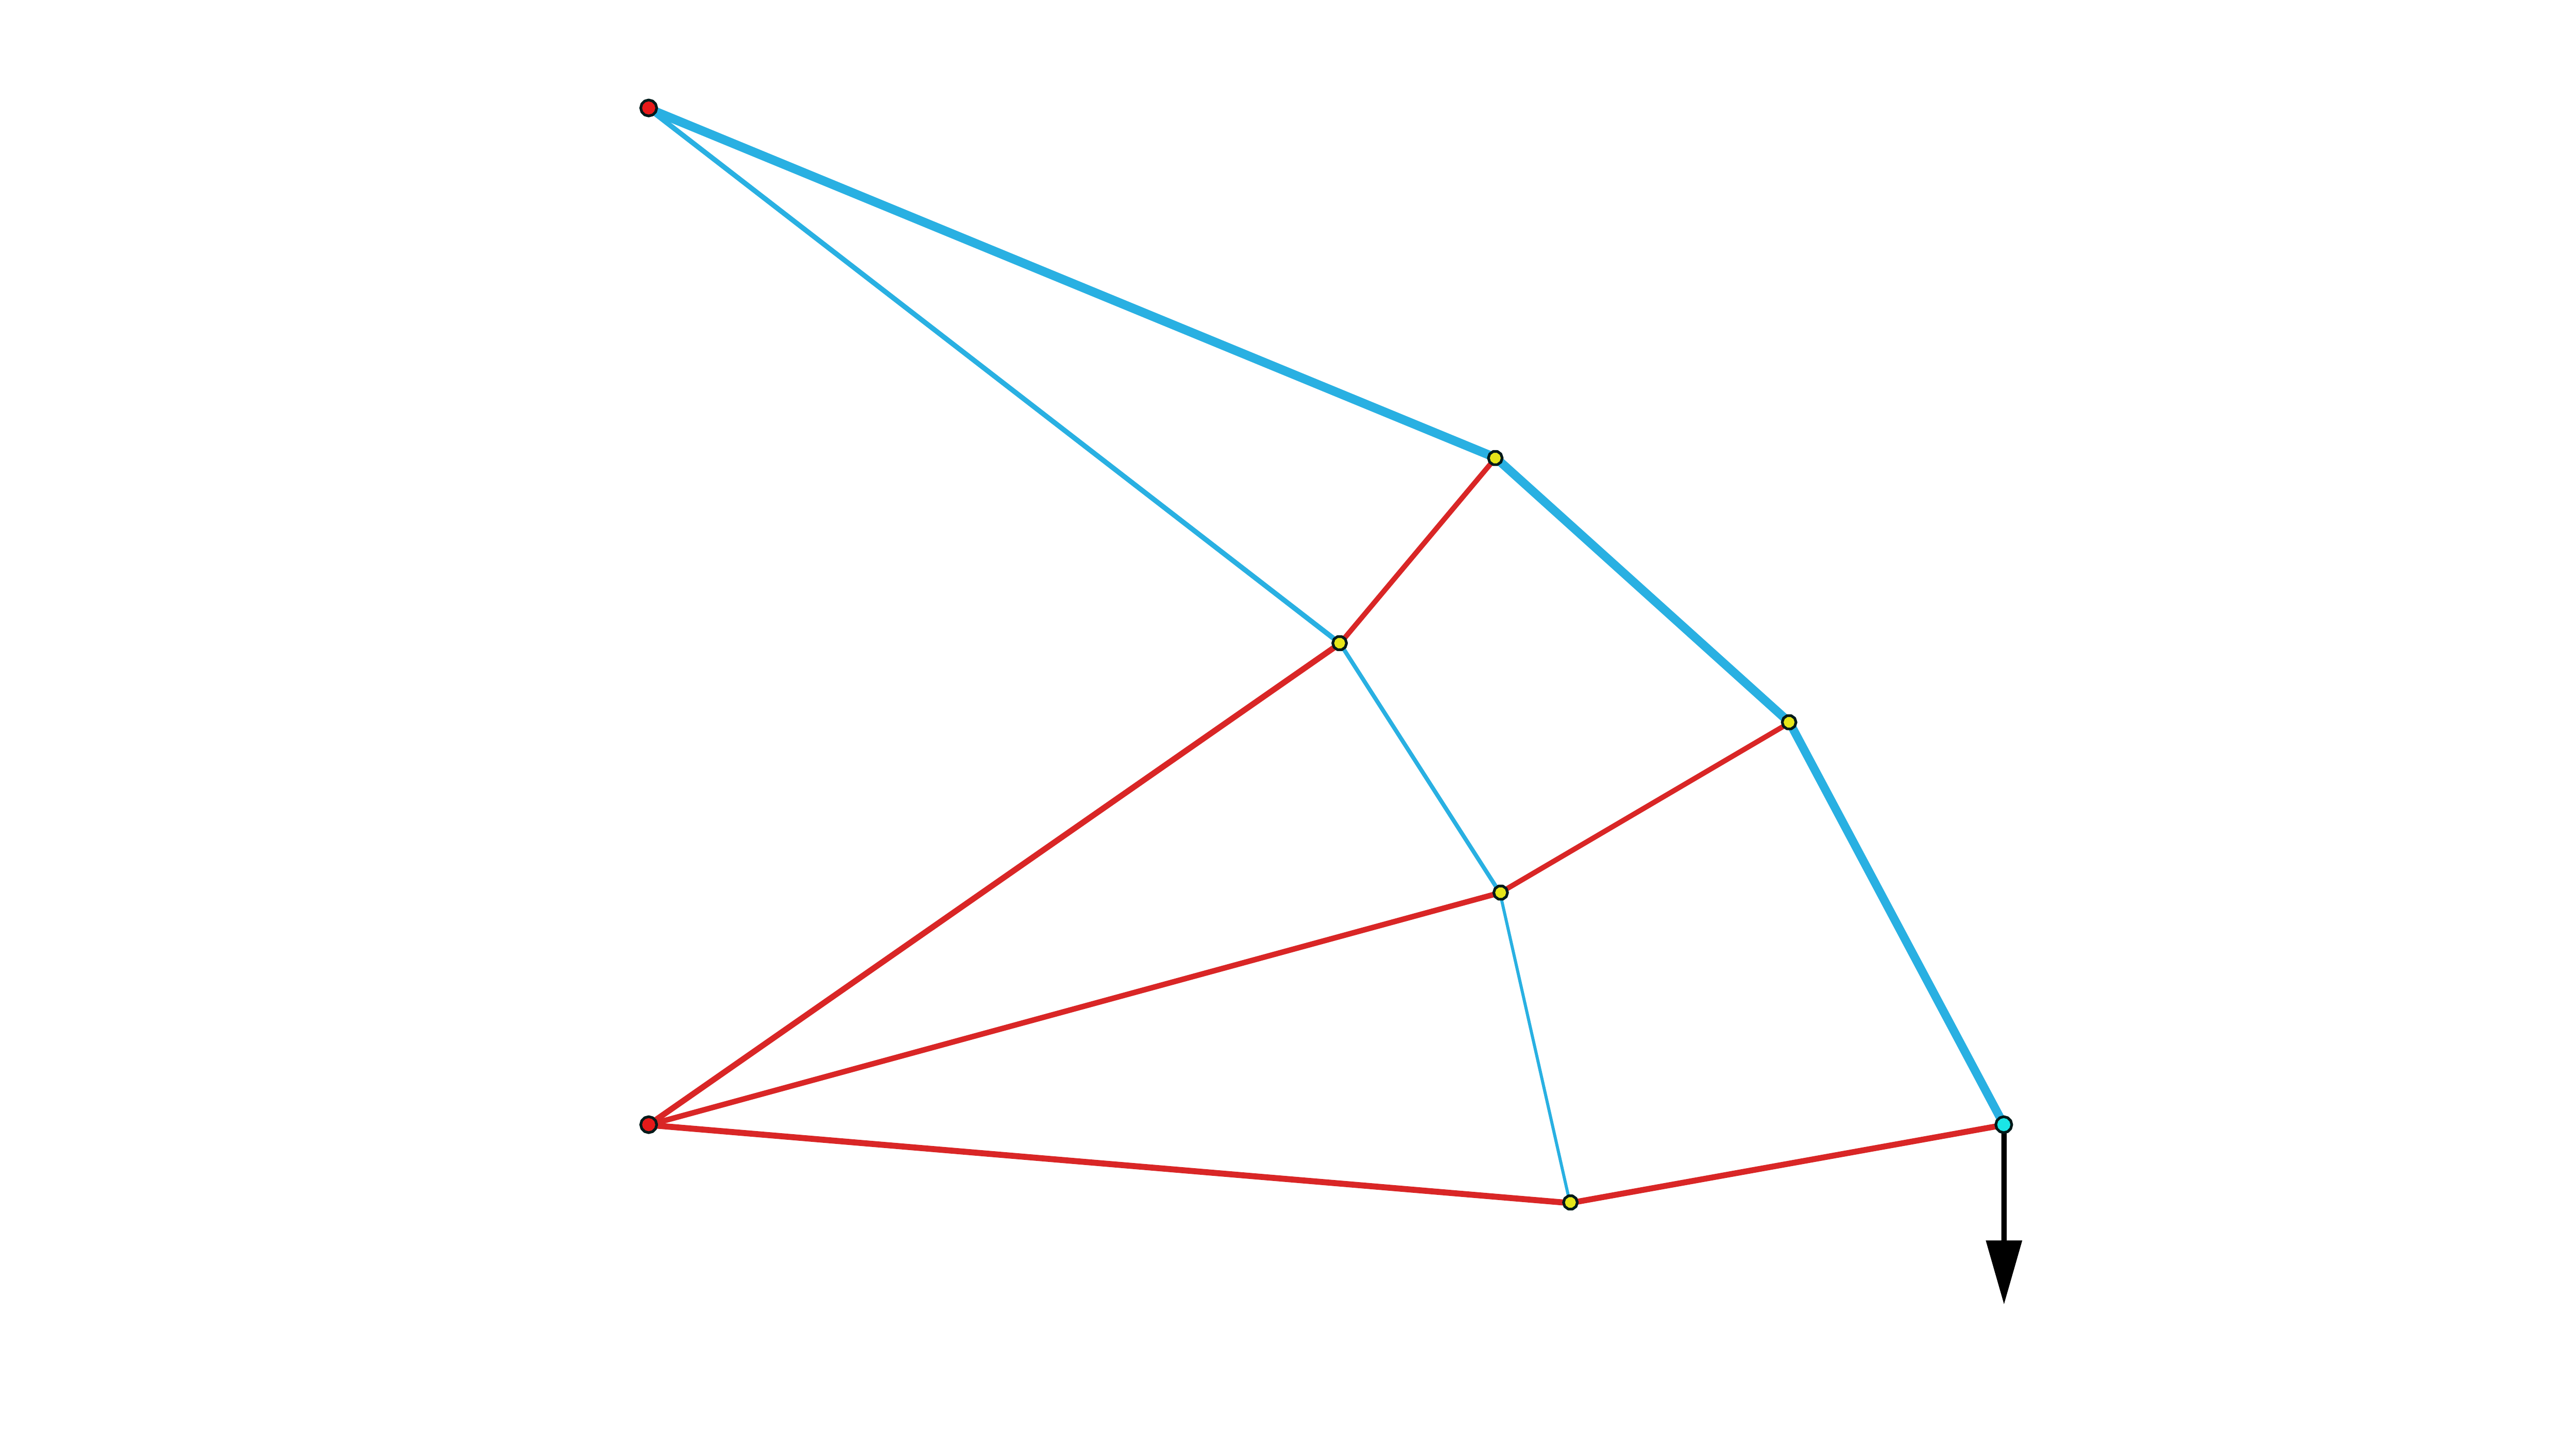}	
			%	\cput(50,2){\contour{white}{$(a)$}}			
		\end{overpic}
	}
	\centering{
		\begin{overpic}	
			[height=.75\columnwidth,trim={20cm 1cm 20cm 1cm},clip]{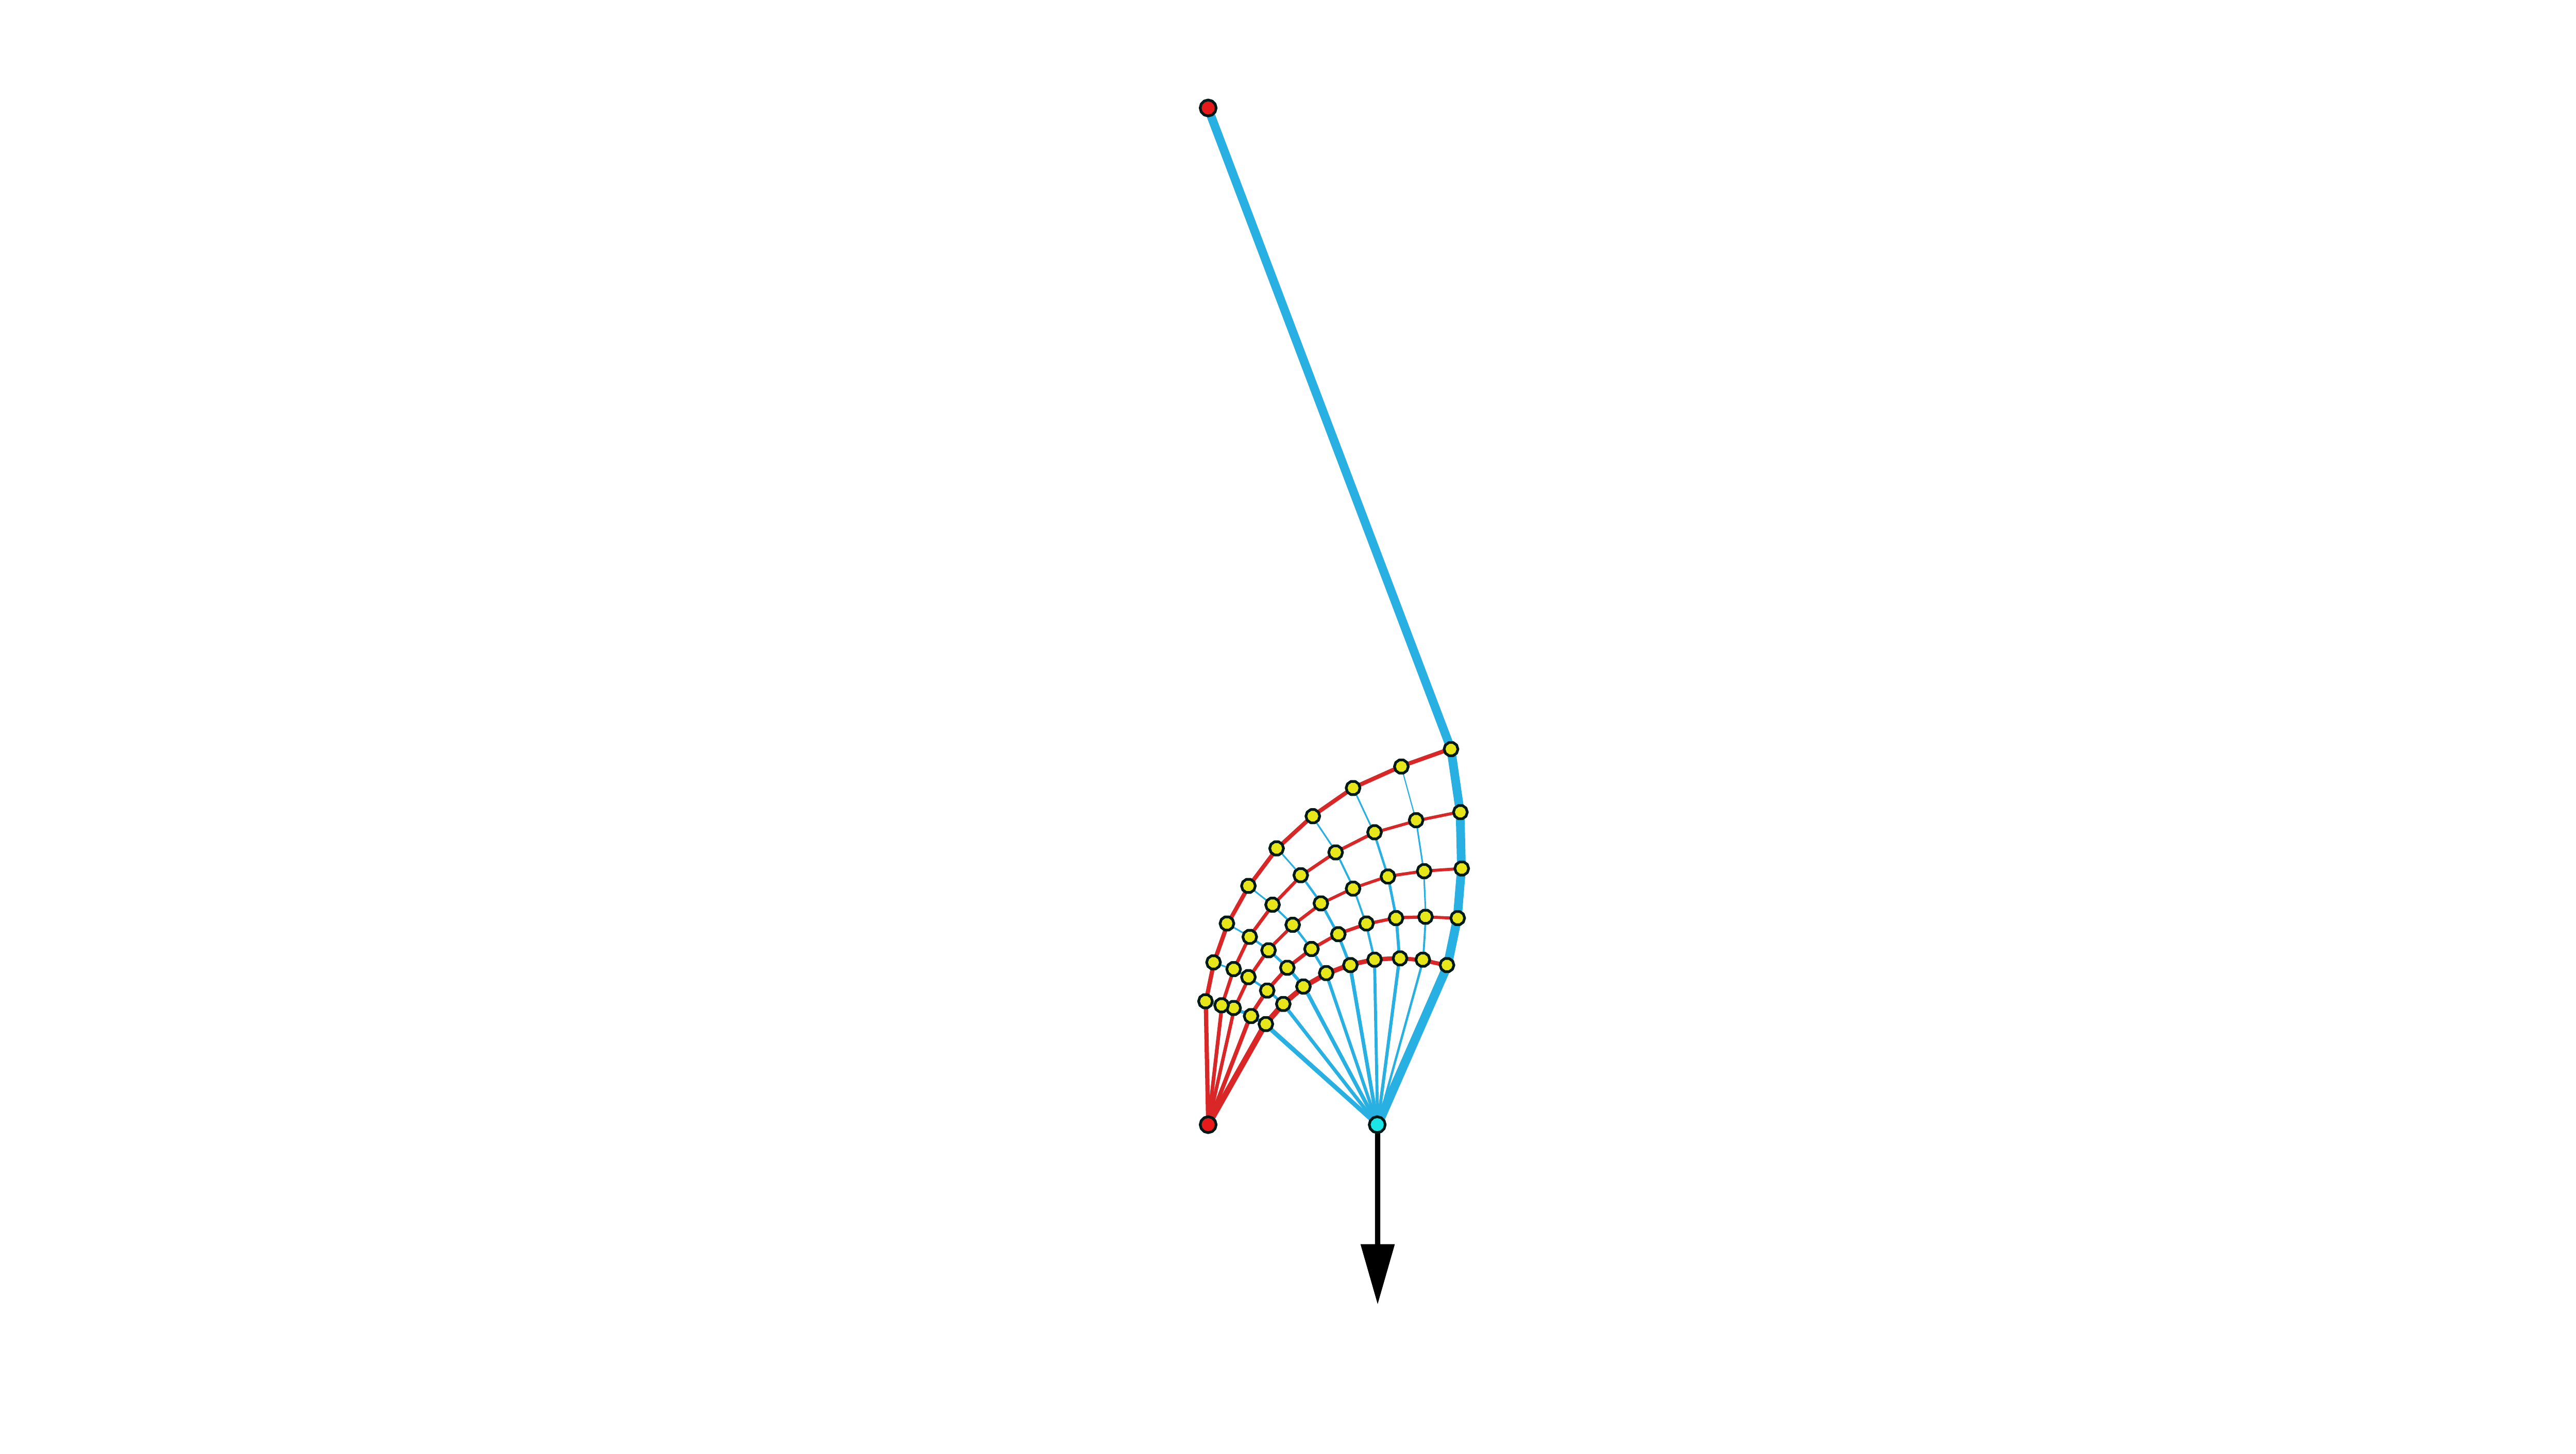}	
			%	\cput(50,2){\contour{white}{$(a)$}}		
		\end{overpic}
		\begin{overpic}			
			[height=.75\columnwidth,trim={20cm 1cm 20cm 1cm},clip]{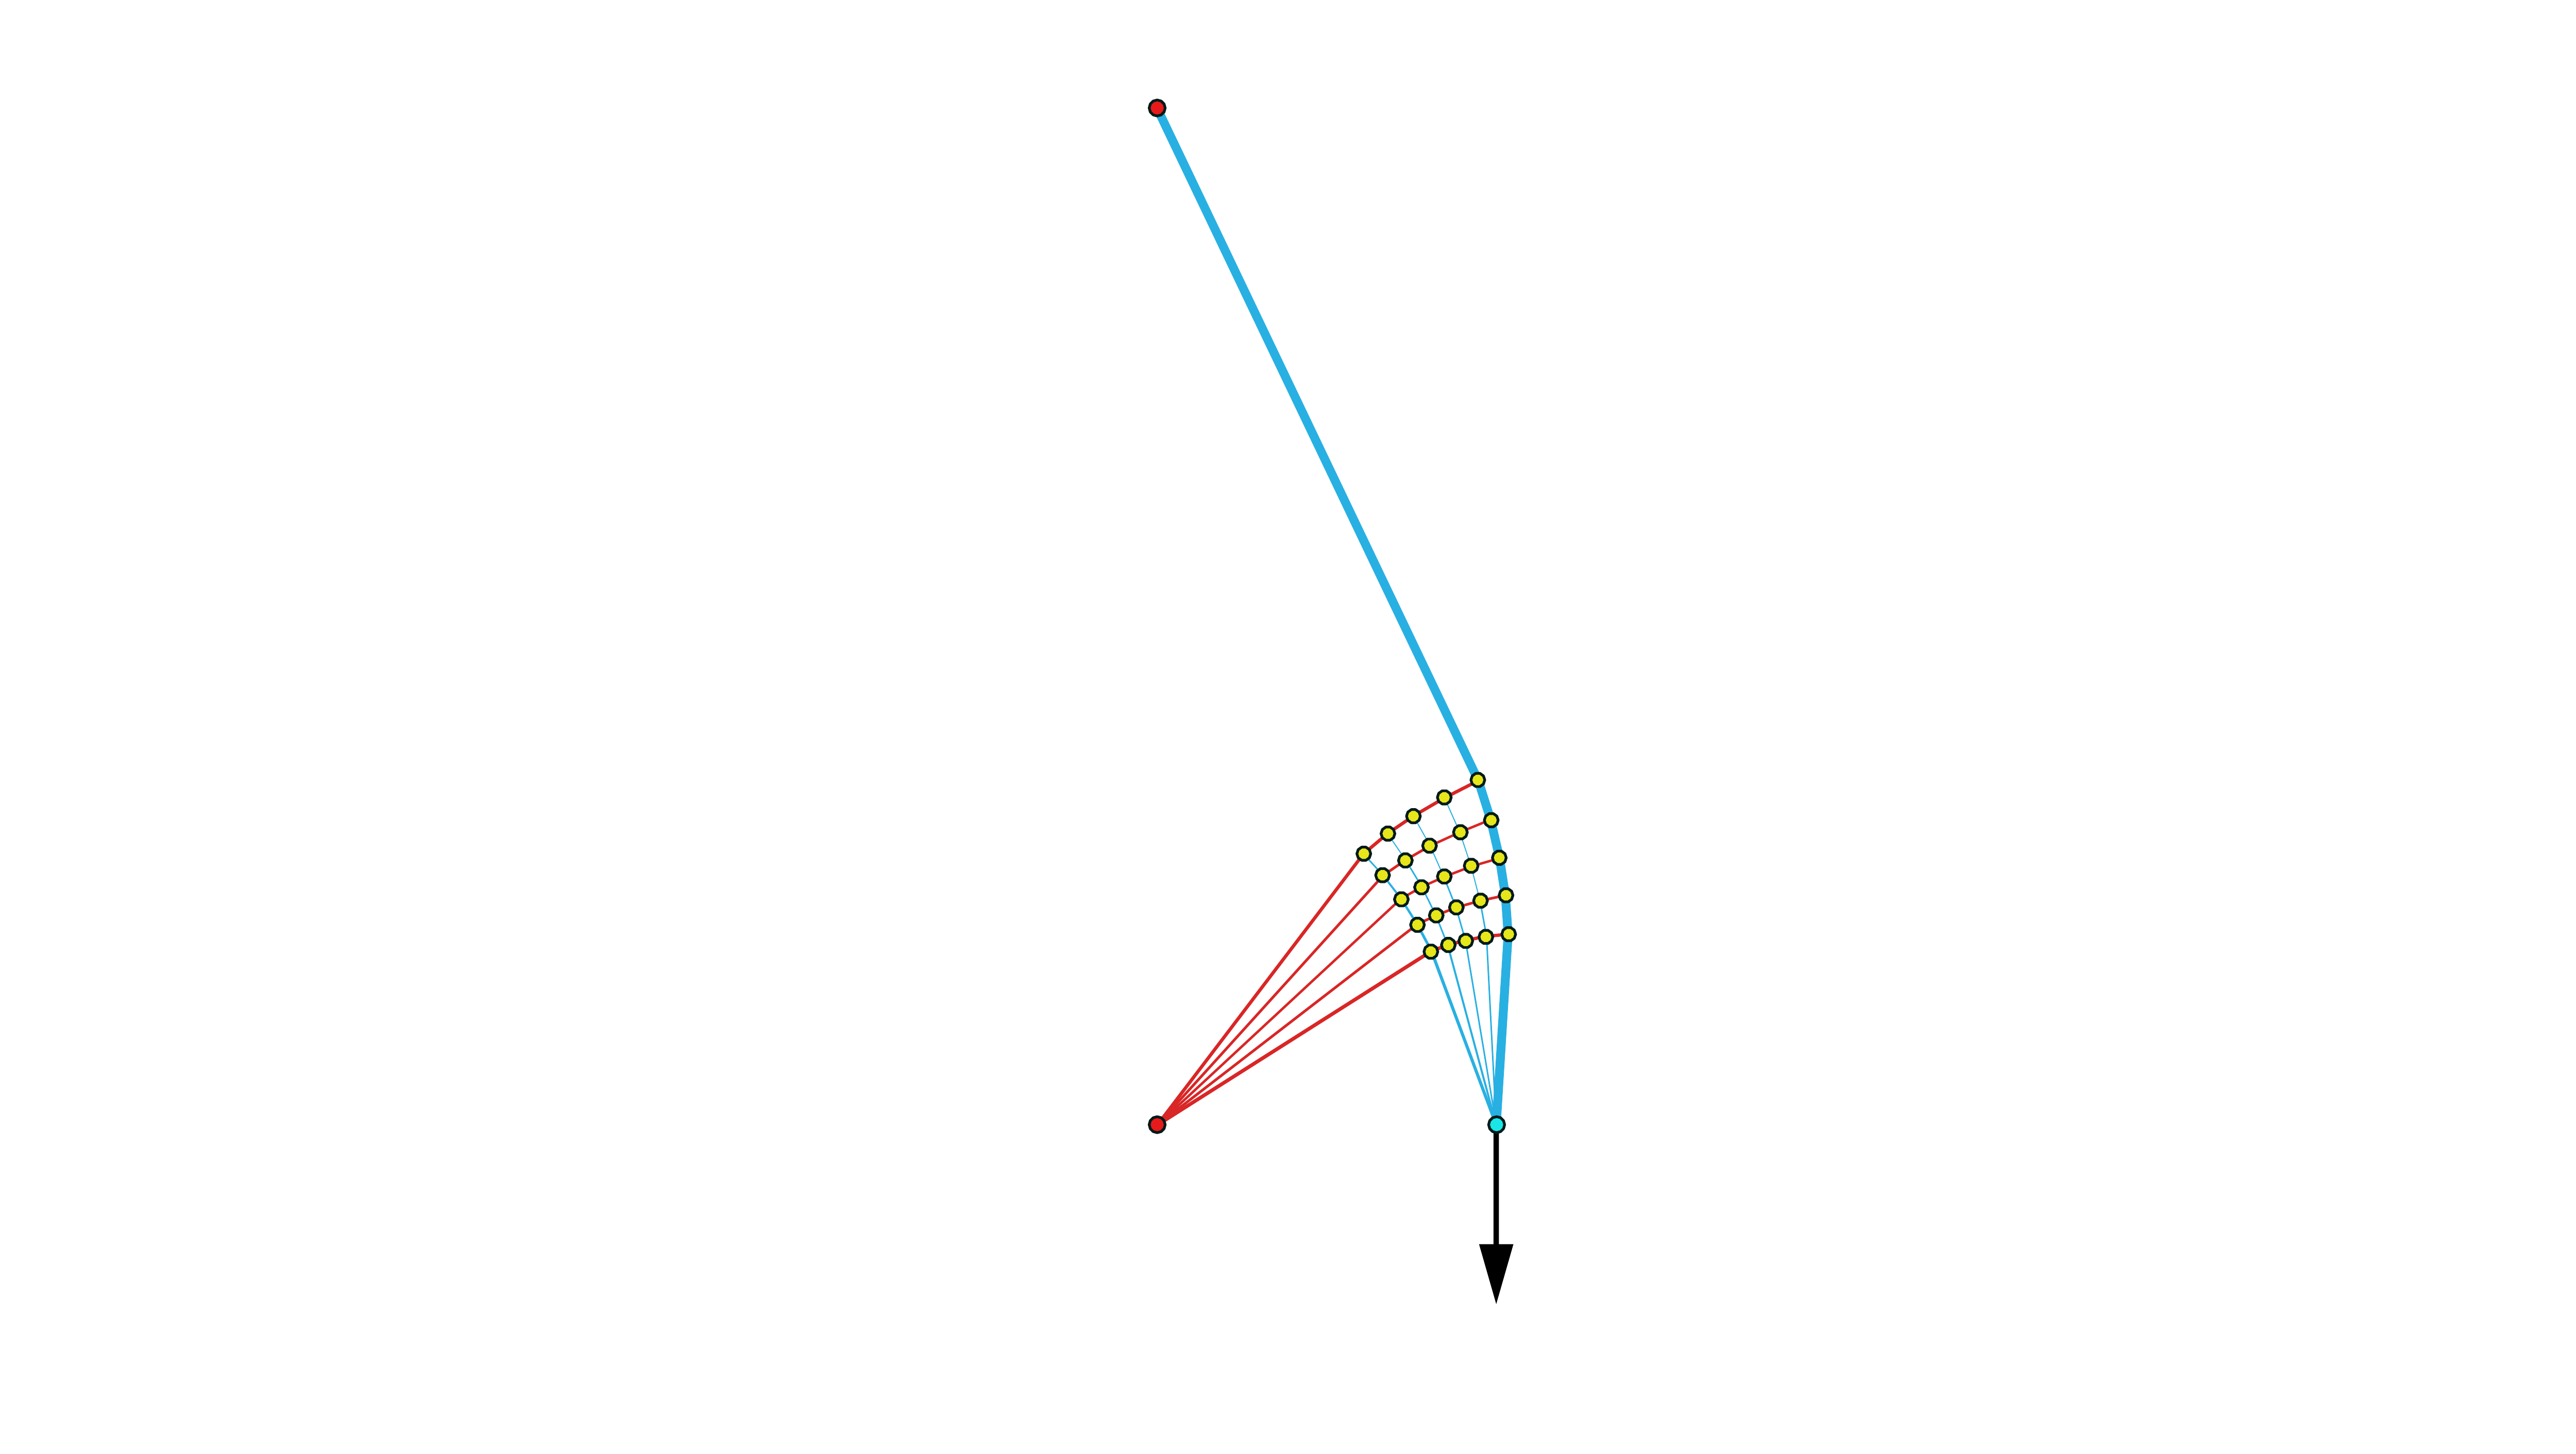}	
			%	\cput(50,2){\contour{white}{$(a)$}}		
		\end{overpic}
		\begin{overpic}			
			[height=.75\columnwidth,trim={18cm 1cm 15cm 1cm},clip]{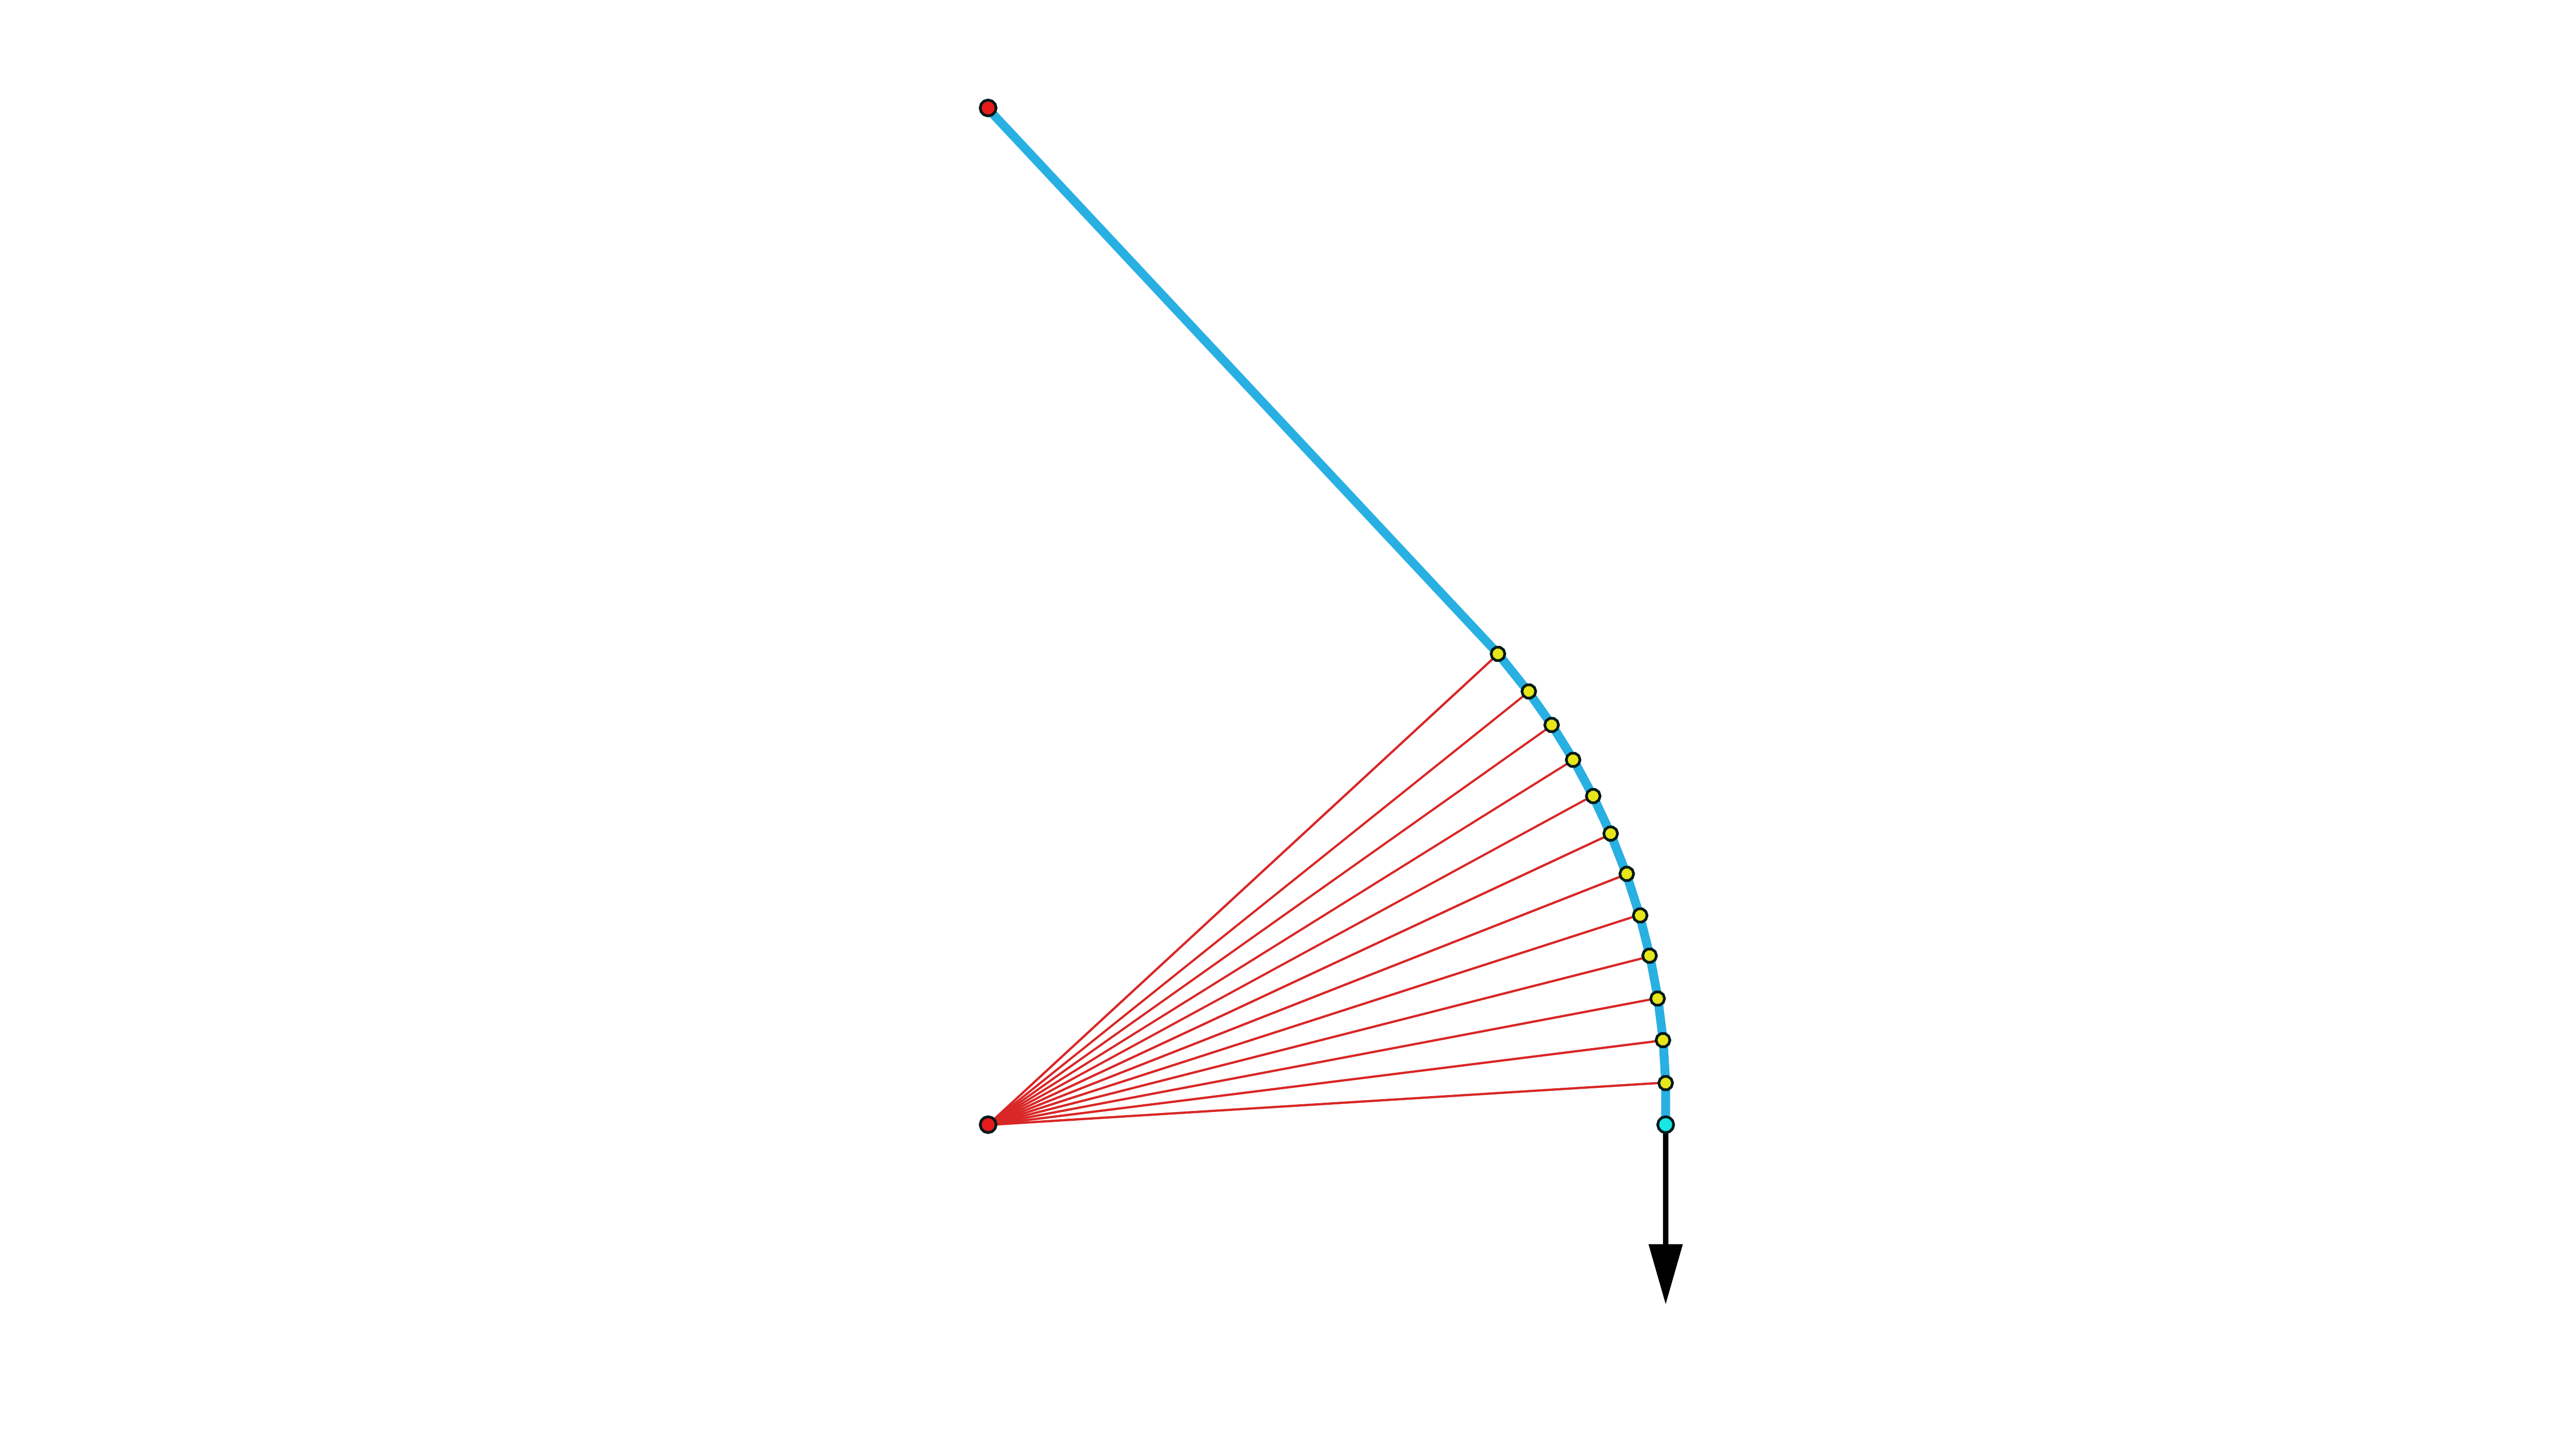}	
			%	\cput(50,2){\contour{white}{$(a)$}}			
		\end{overpic}
		\begin{overpic}			
			[height=.75\columnwidth,trim={12.5cm 1cm 10cm 1cm},clip]{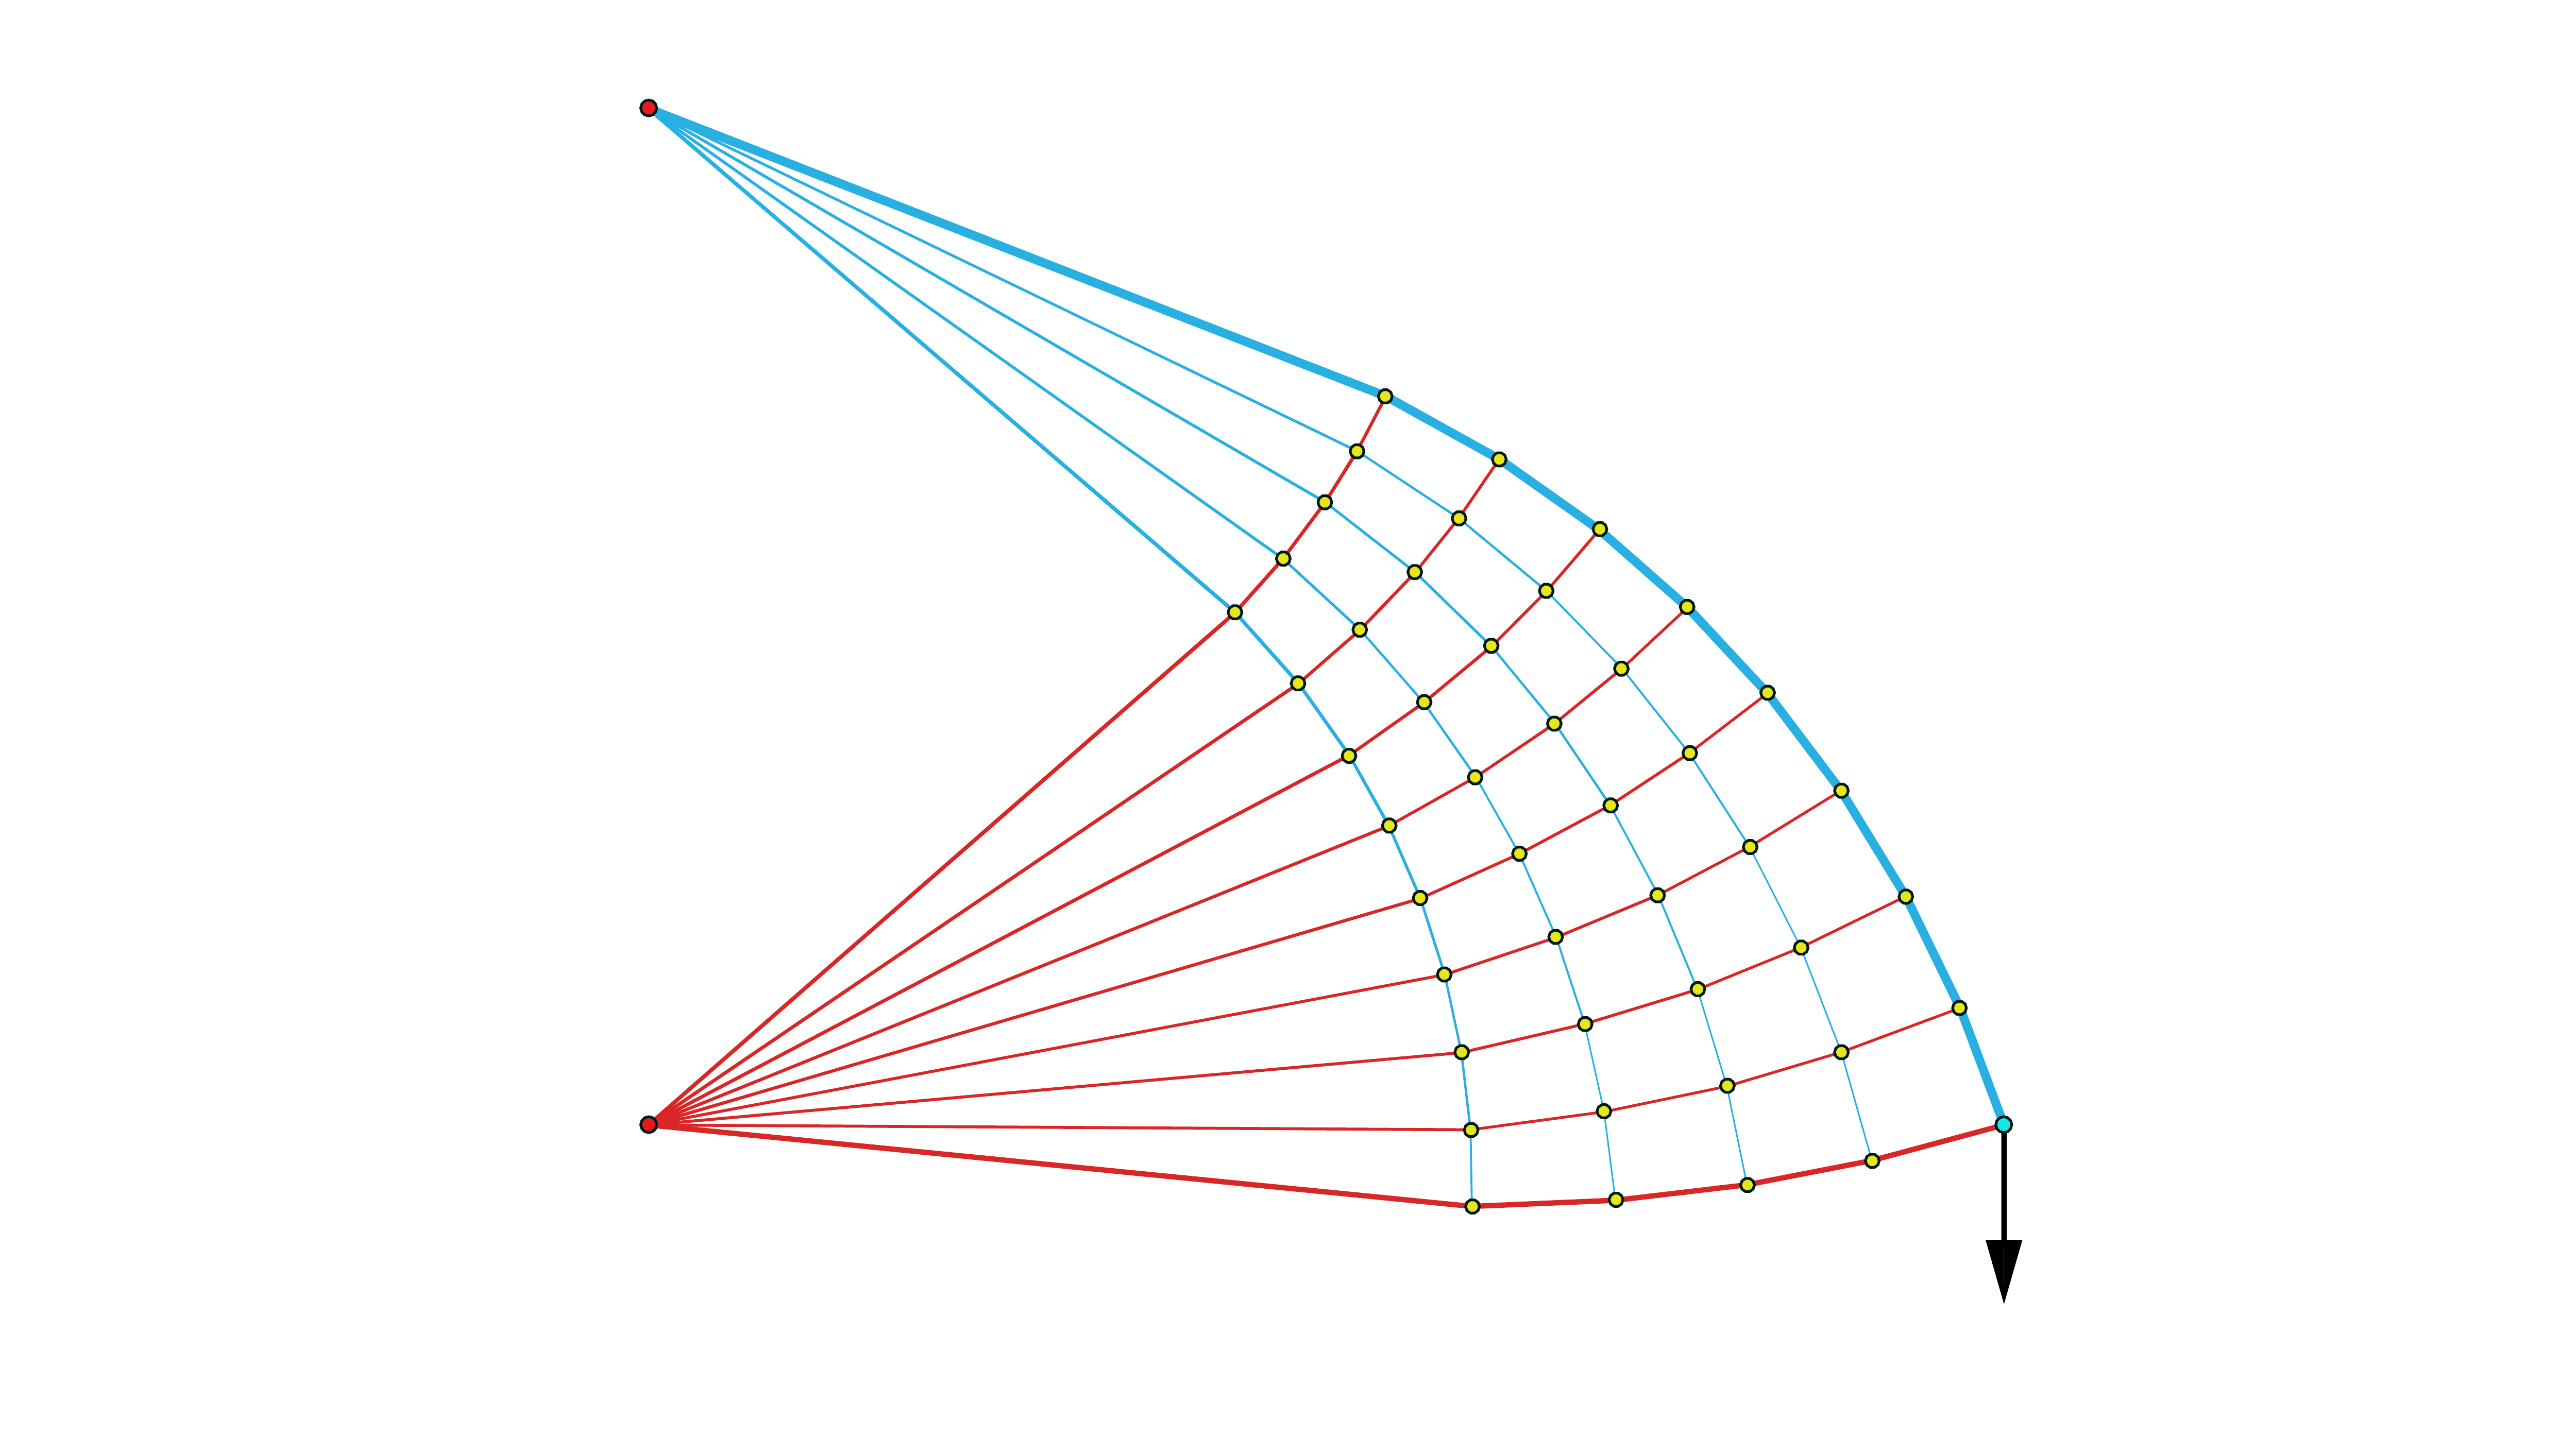}	
			%	\cput(50,2){\contour{white}{$(a)$}}			
		\end{overpic}							
	}	
	\caption{
		\label{fig:ex_oneforce}
		Input functional specification has two supporting points $A(0,0)$ and $B(0,0.3)$ and an external force applied at $C(l,0)$. The above optimized trusses are for $l=0.05, 1, 0.2$ and 0.4.}
\end{figure*}
\clearpage
